# Supplementary material for: Encode, Shuffle, Analyze Privacy Revisited: Formalizations and Empirical Evaluation
Source: arXiv:2001.03618 ancillary file (2020-01-10)
Supplement: Supplementary file 1 [file horse.pdf]

TABLE IV: Experimental results of reconstructing the Horse image dataset by varying  $\varepsilon_c$  and evaluating a central DP mechanism, attribute fragmenting, and both attribute and report fragmenting achieving  $(\varepsilon_c, \delta_c)$ -central DP with  $\delta_c = 5 \times 10^{-8}$ .

| Central privacy guarantee | No LDP (Gaussian mechanism)                                                                                                                               | Attribute-fragmented LDP report                                                                                                                                             | Attribute- and report-fragmented LDP reports                                                                                                                                |                                                                                                                                                                               |                                                                                                                                                                               |
|---------------------------|-----------------------------------------------------------------------------------------------------------------------------------------------------------|-----------------------------------------------------------------------------------------------------------------------------------------------------------------------------|-----------------------------------------------------------------------------------------------------------------------------------------------------------------------------|-------------------------------------------------------------------------------------------------------------------------------------------------------------------------------|-------------------------------------------------------------------------------------------------------------------------------------------------------------------------------|
|                           |                                                                                                                                                           |                                                                                                                                                                             | $\tau = 4$ reports                                                                                                                                                          | $\tau = 16$ reports                                                                                                                                                           | $\tau = 256$ reports                                                                                                                                                          |
| $\varepsilon_c = 0.05$    | 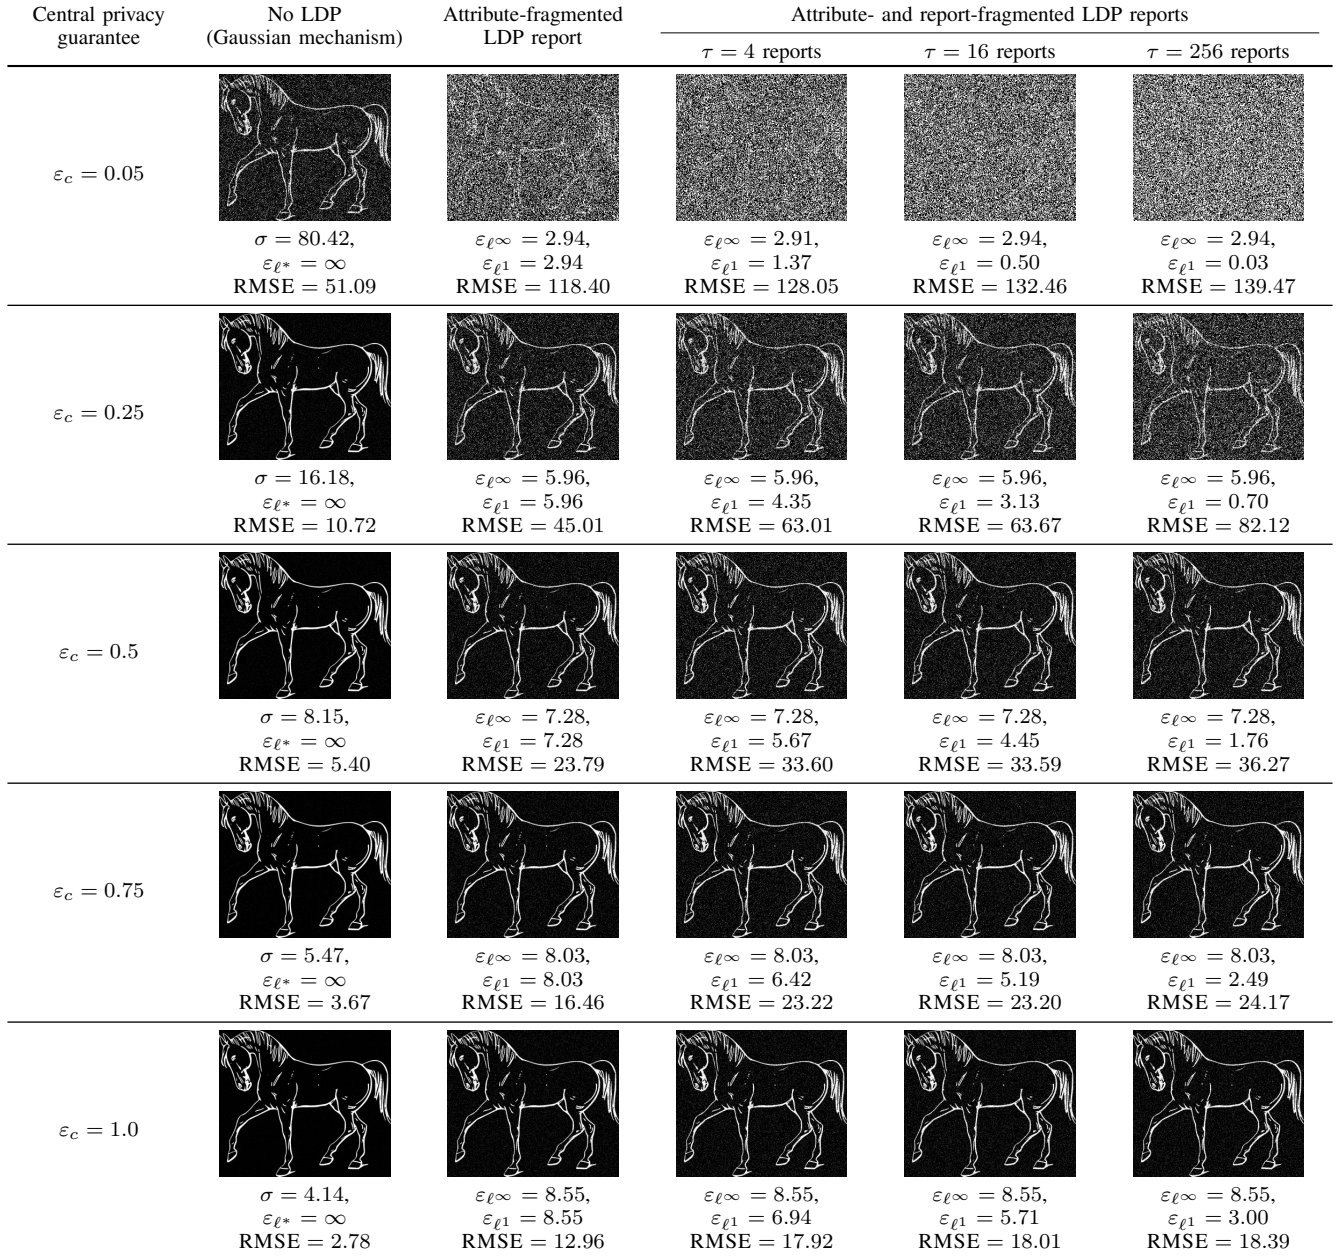<br>$\sigma = 80.42,$<br>$\varepsilon_{\ell^*} = \infty$<br>RMSE = 51.09 | 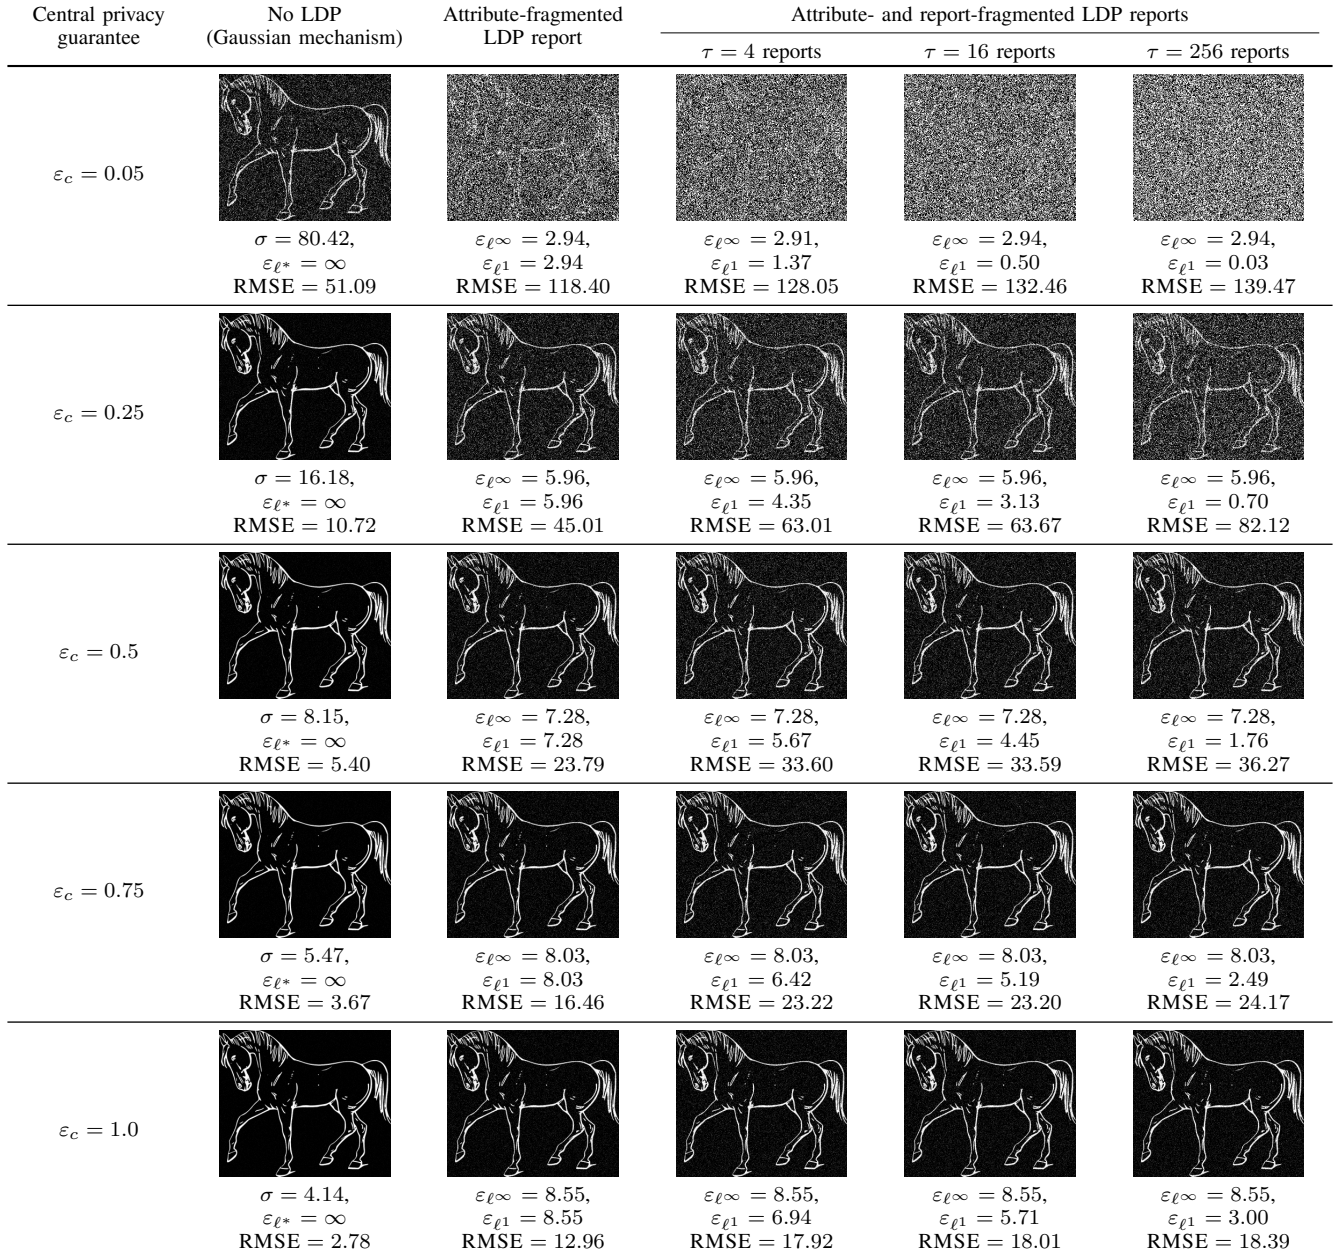<br>$\varepsilon_{\ell^\infty} = 2.94,$<br>$\varepsilon_{\ell^1} = 2.94$<br>RMSE = 118.40  | 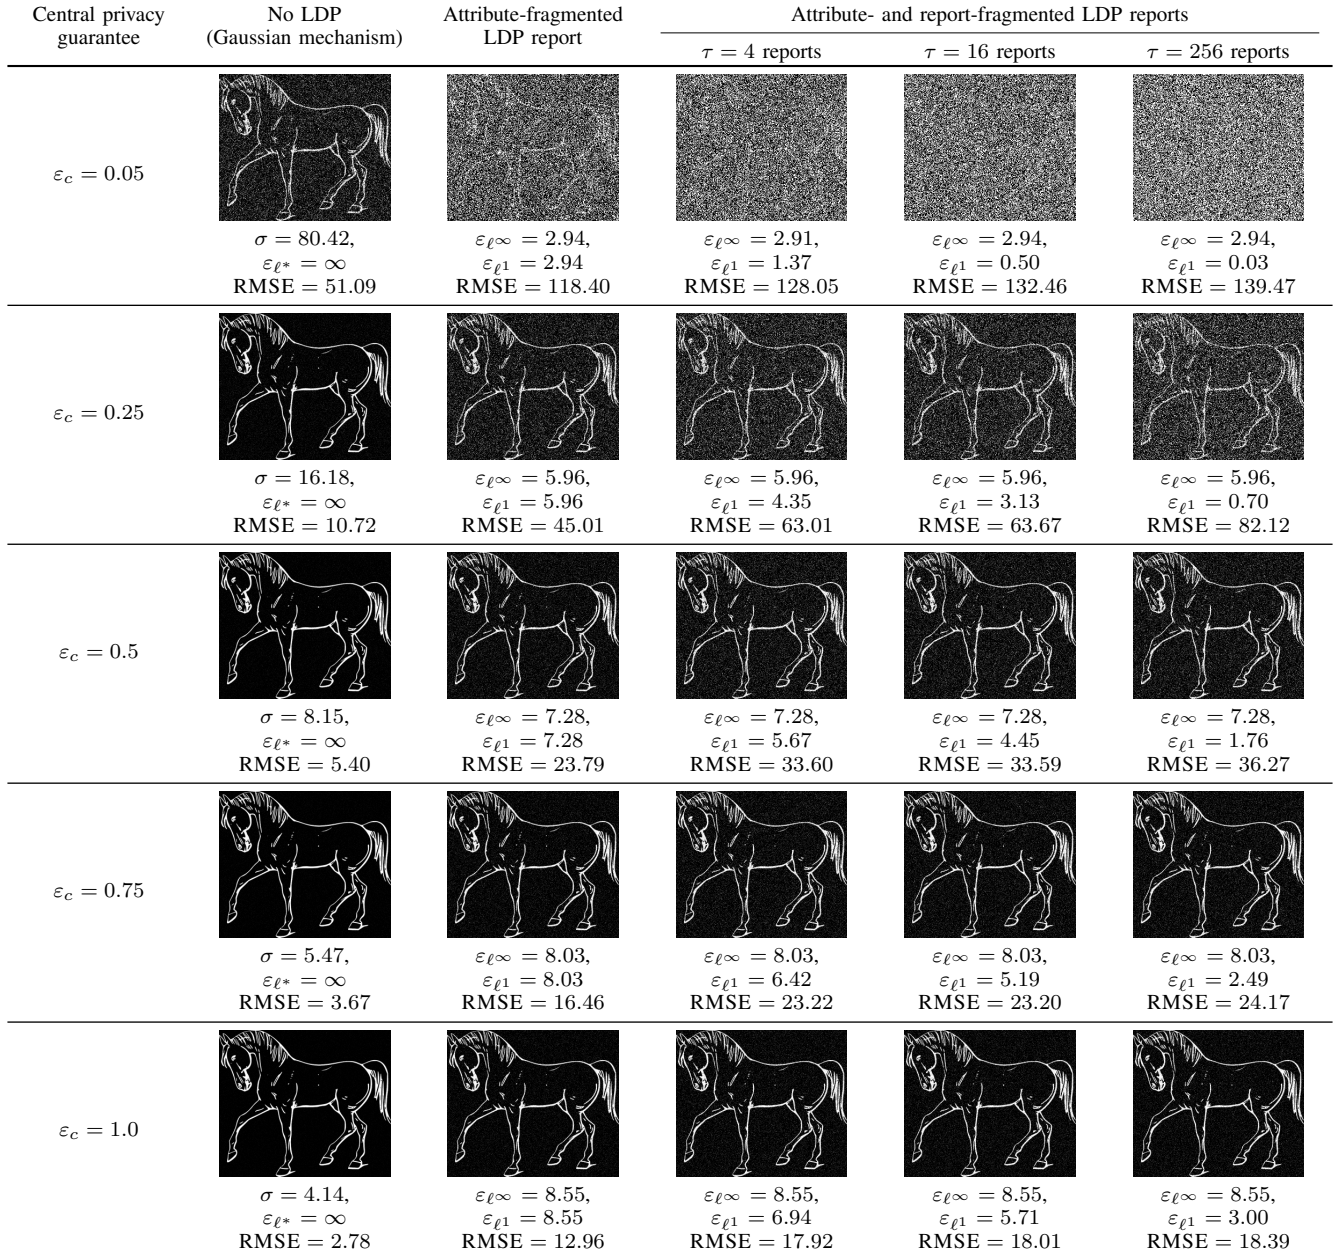<br>$\varepsilon_{\ell^\infty} = 2.91,$<br>$\varepsilon_{\ell^1} = 1.37$<br>RMSE = 128.05  | 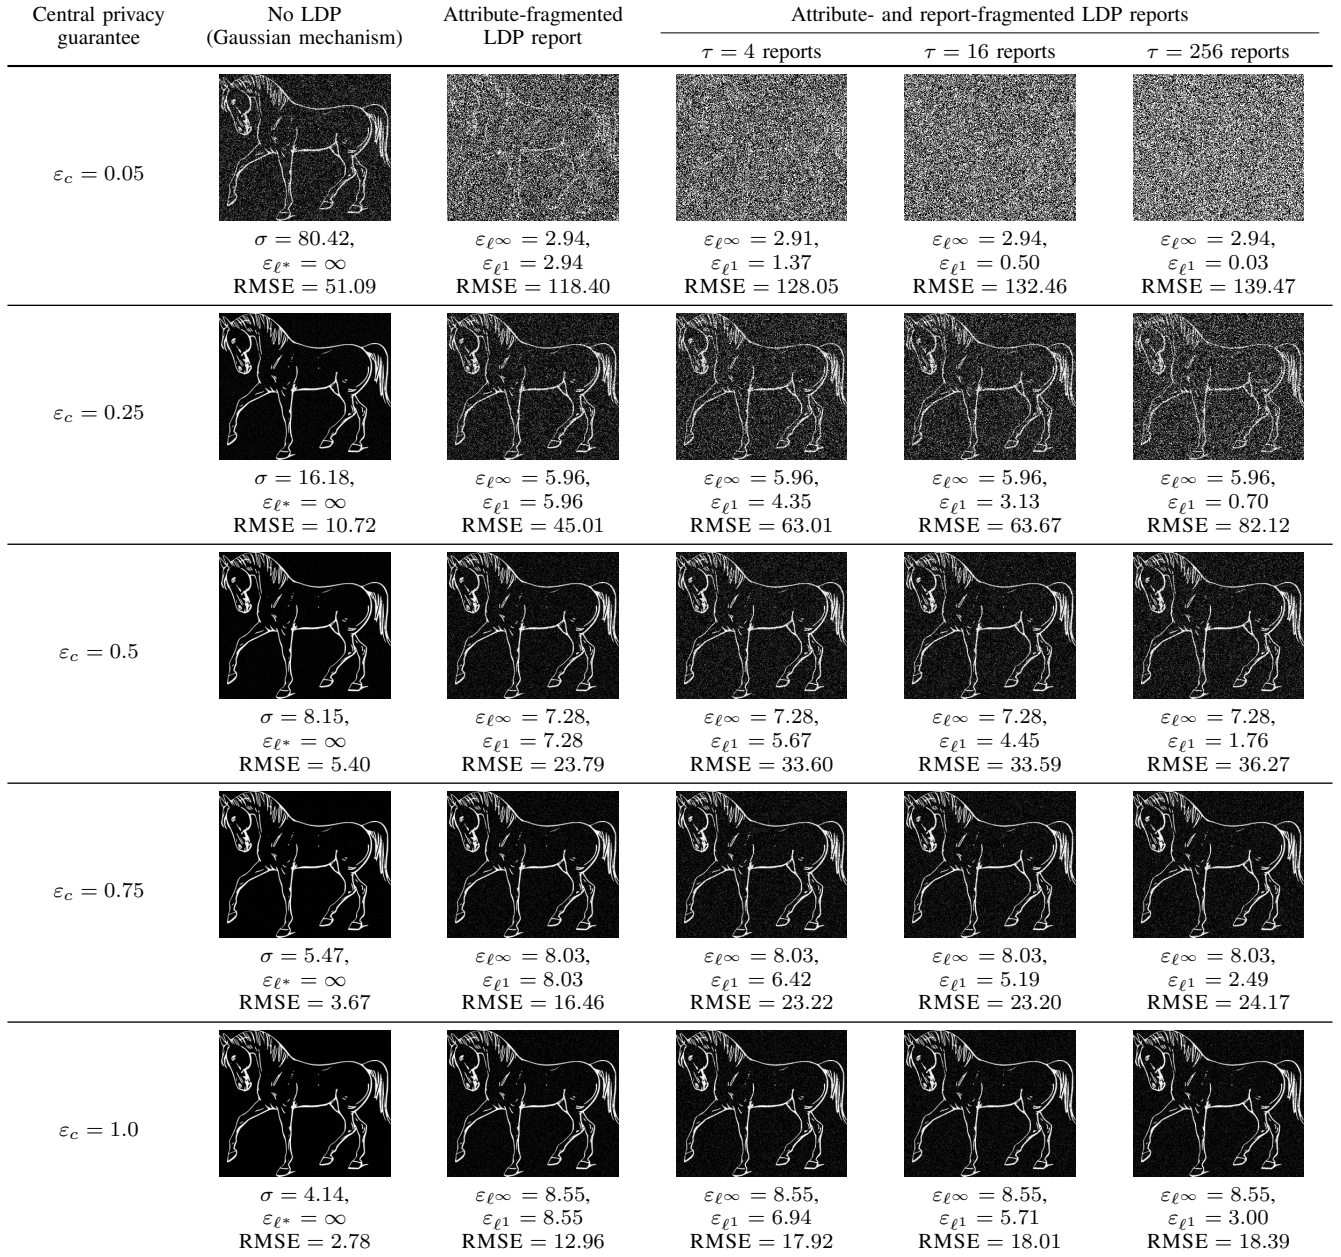<br>$\varepsilon_{\ell^\infty} = 2.94,$<br>$\varepsilon_{\ell^1} = 0.50$<br>RMSE = 132.46  | 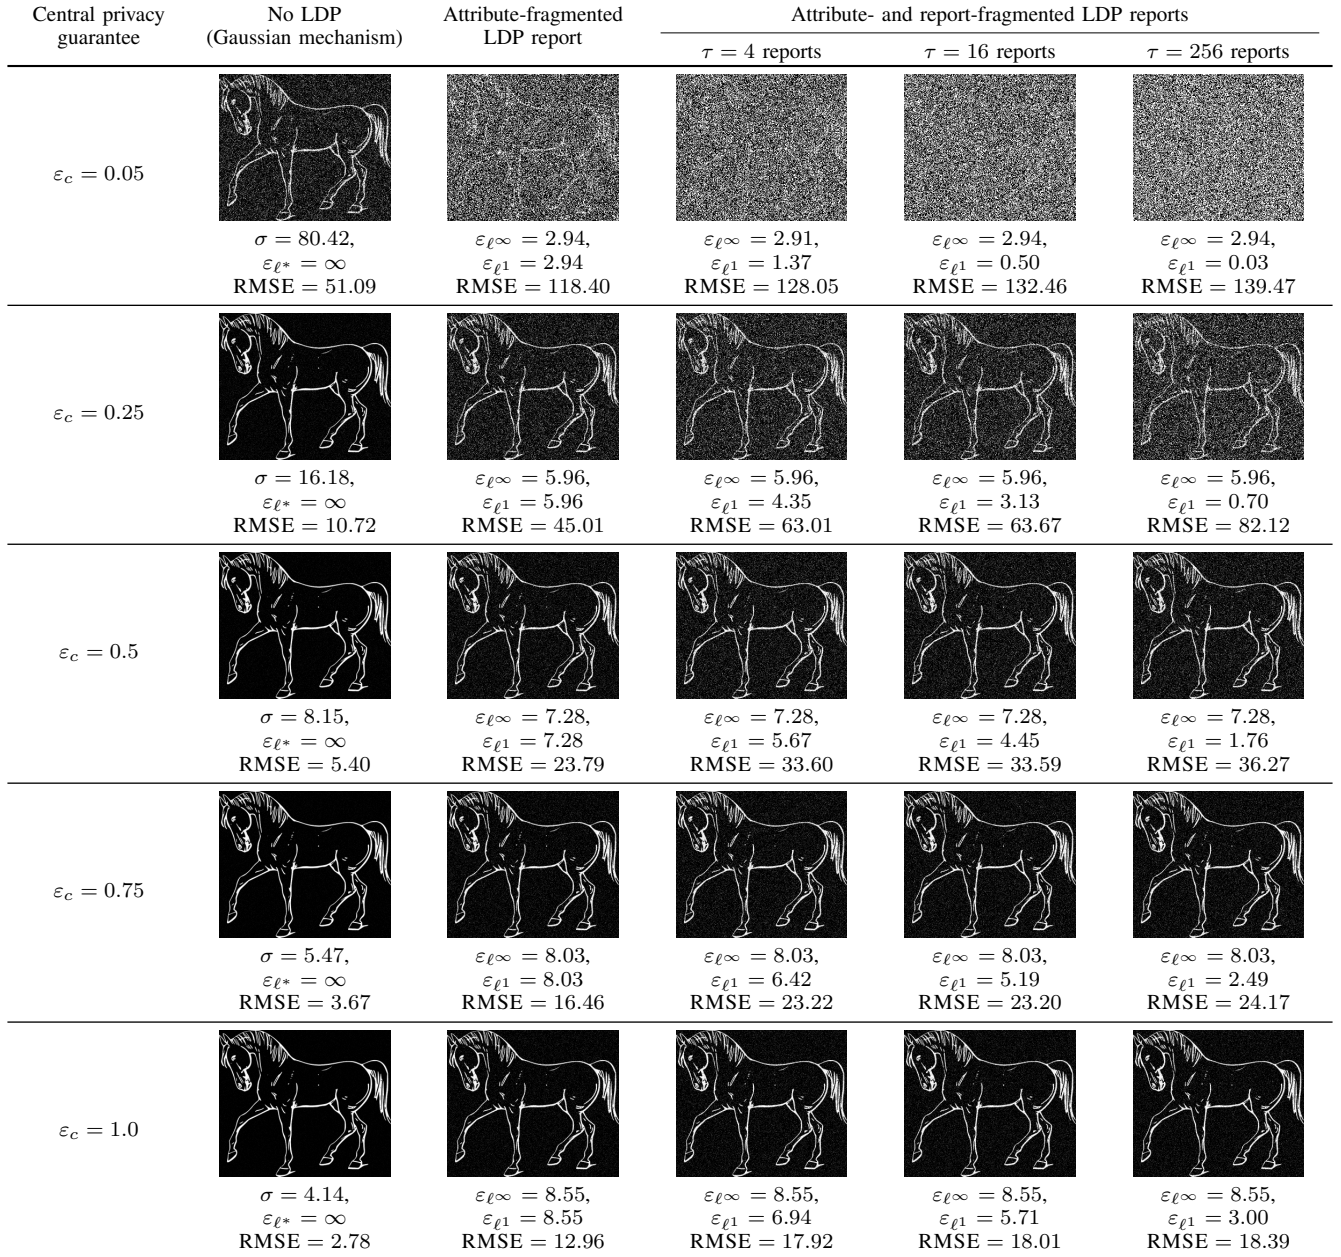<br>$\varepsilon_{\ell^\infty} = 2.94,$<br>$\varepsilon_{\ell^1} = 0.03$<br>RMSE = 139.47  |
| $\varepsilon_c = 0.25$    | 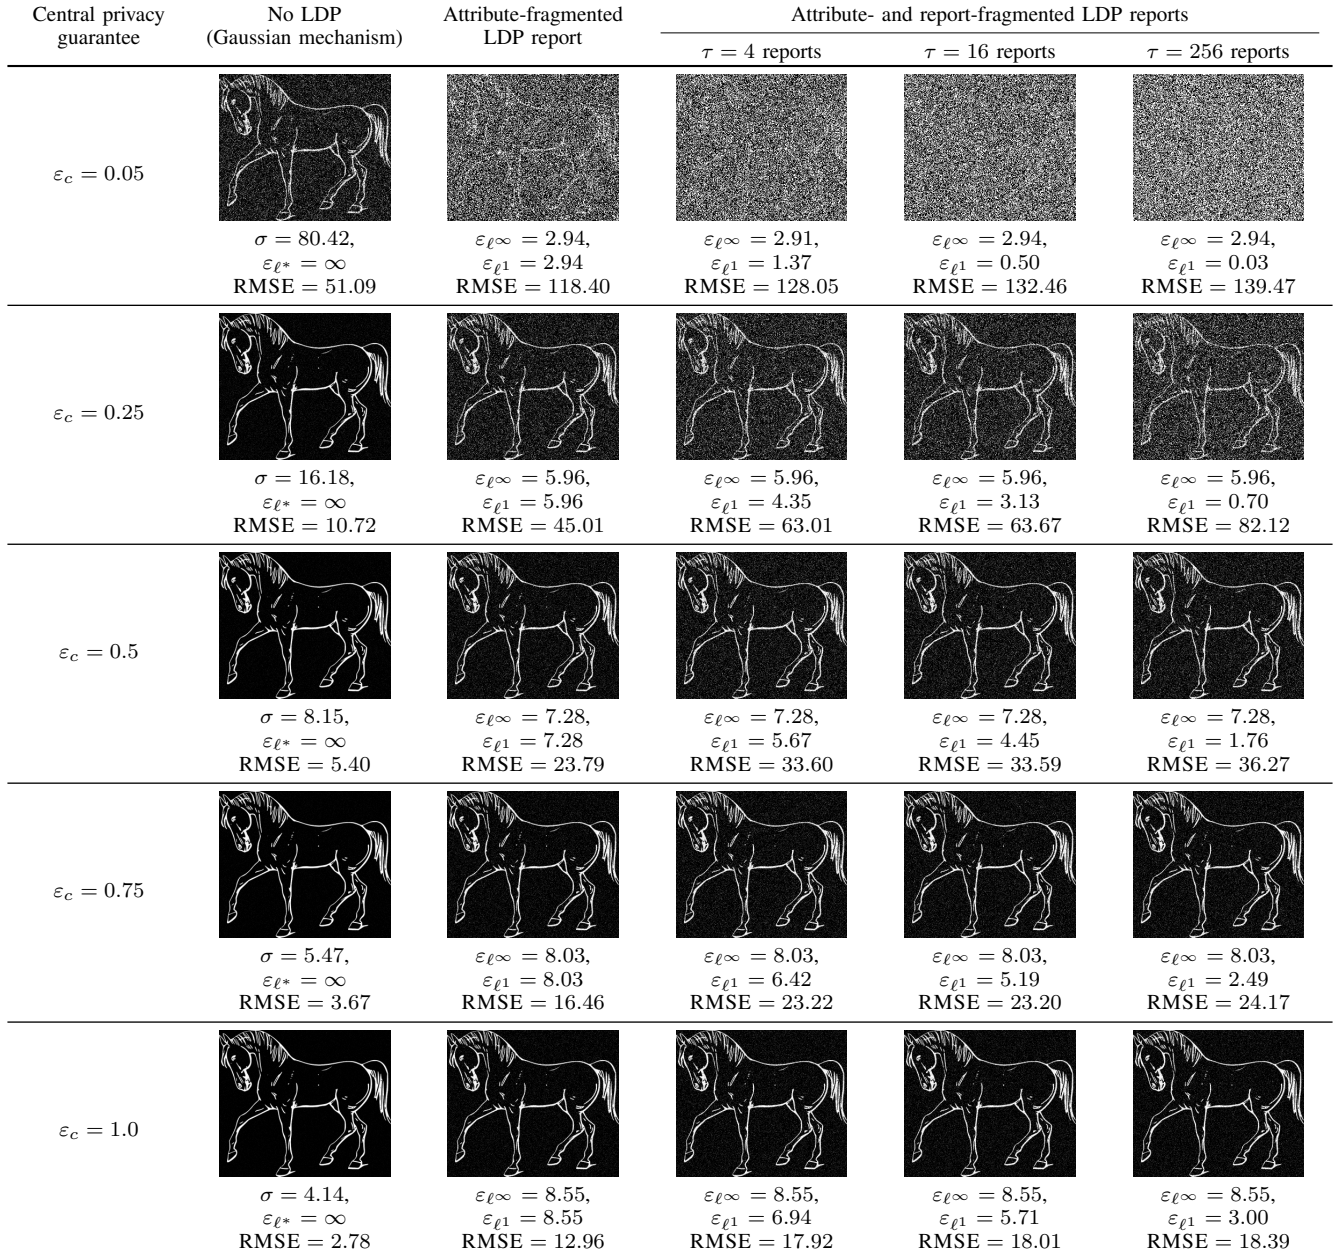<br>$\sigma = 16.18,$<br>$\varepsilon_{\ell^*} = \infty$<br>RMSE = 10.72 | 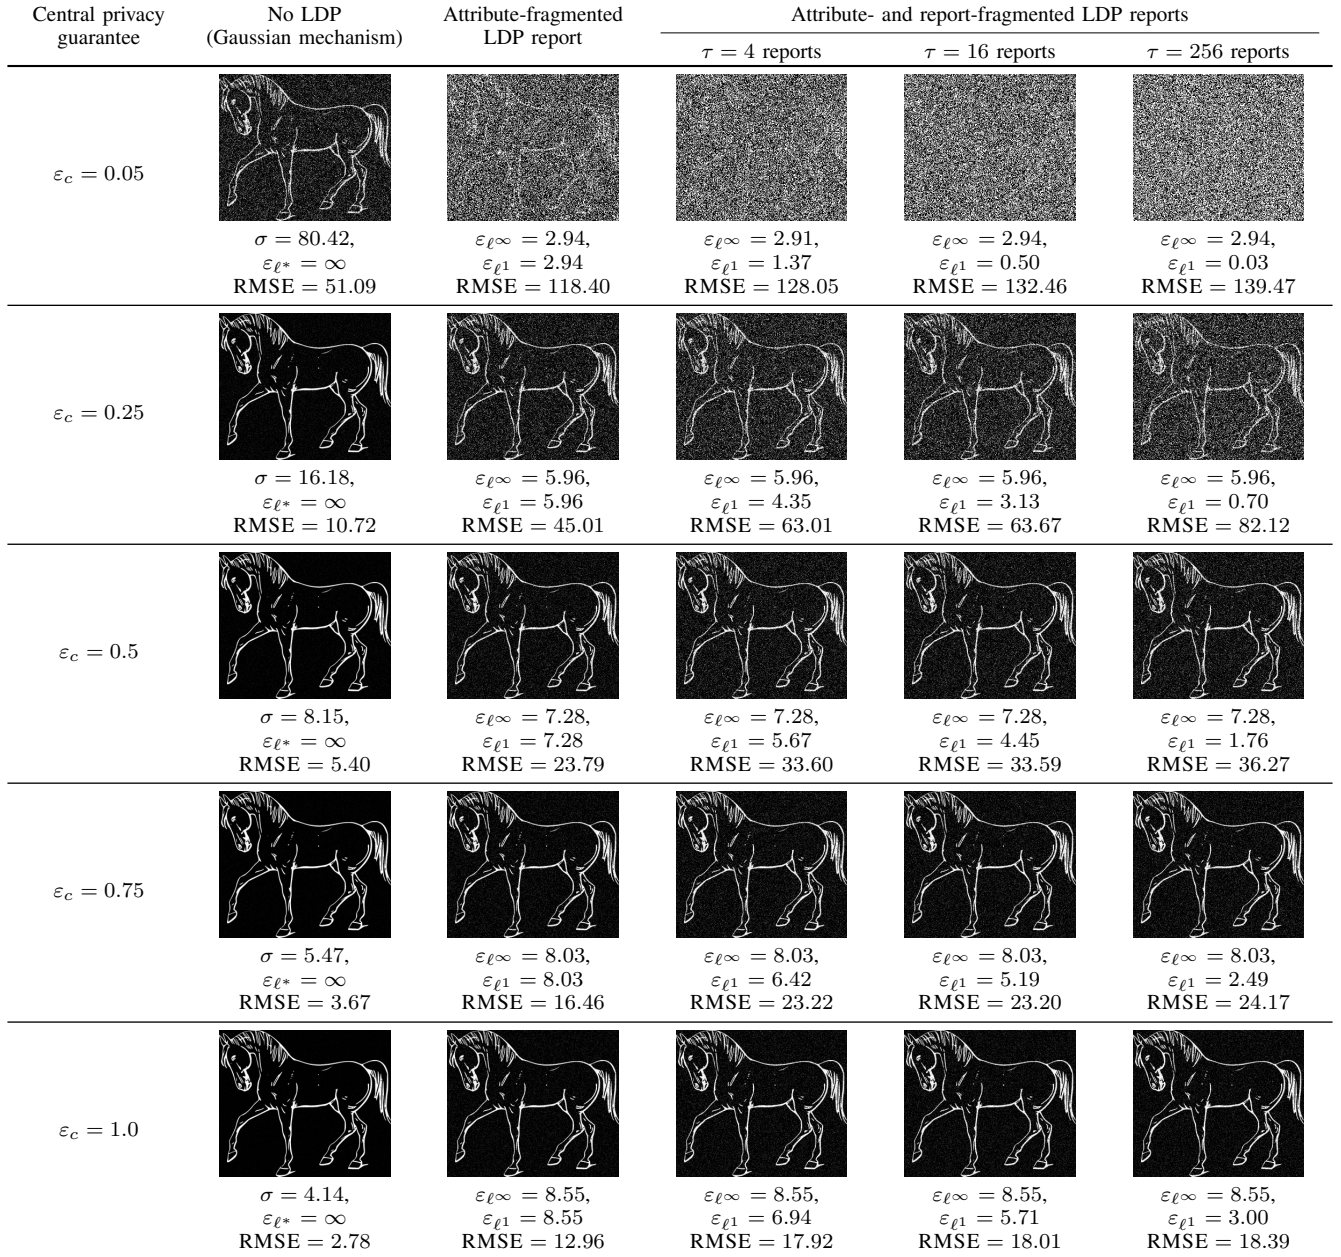<br>$\varepsilon_{\ell^\infty} = 5.96,$<br>$\varepsilon_{\ell^1} = 5.96$<br>RMSE = 45.01   | 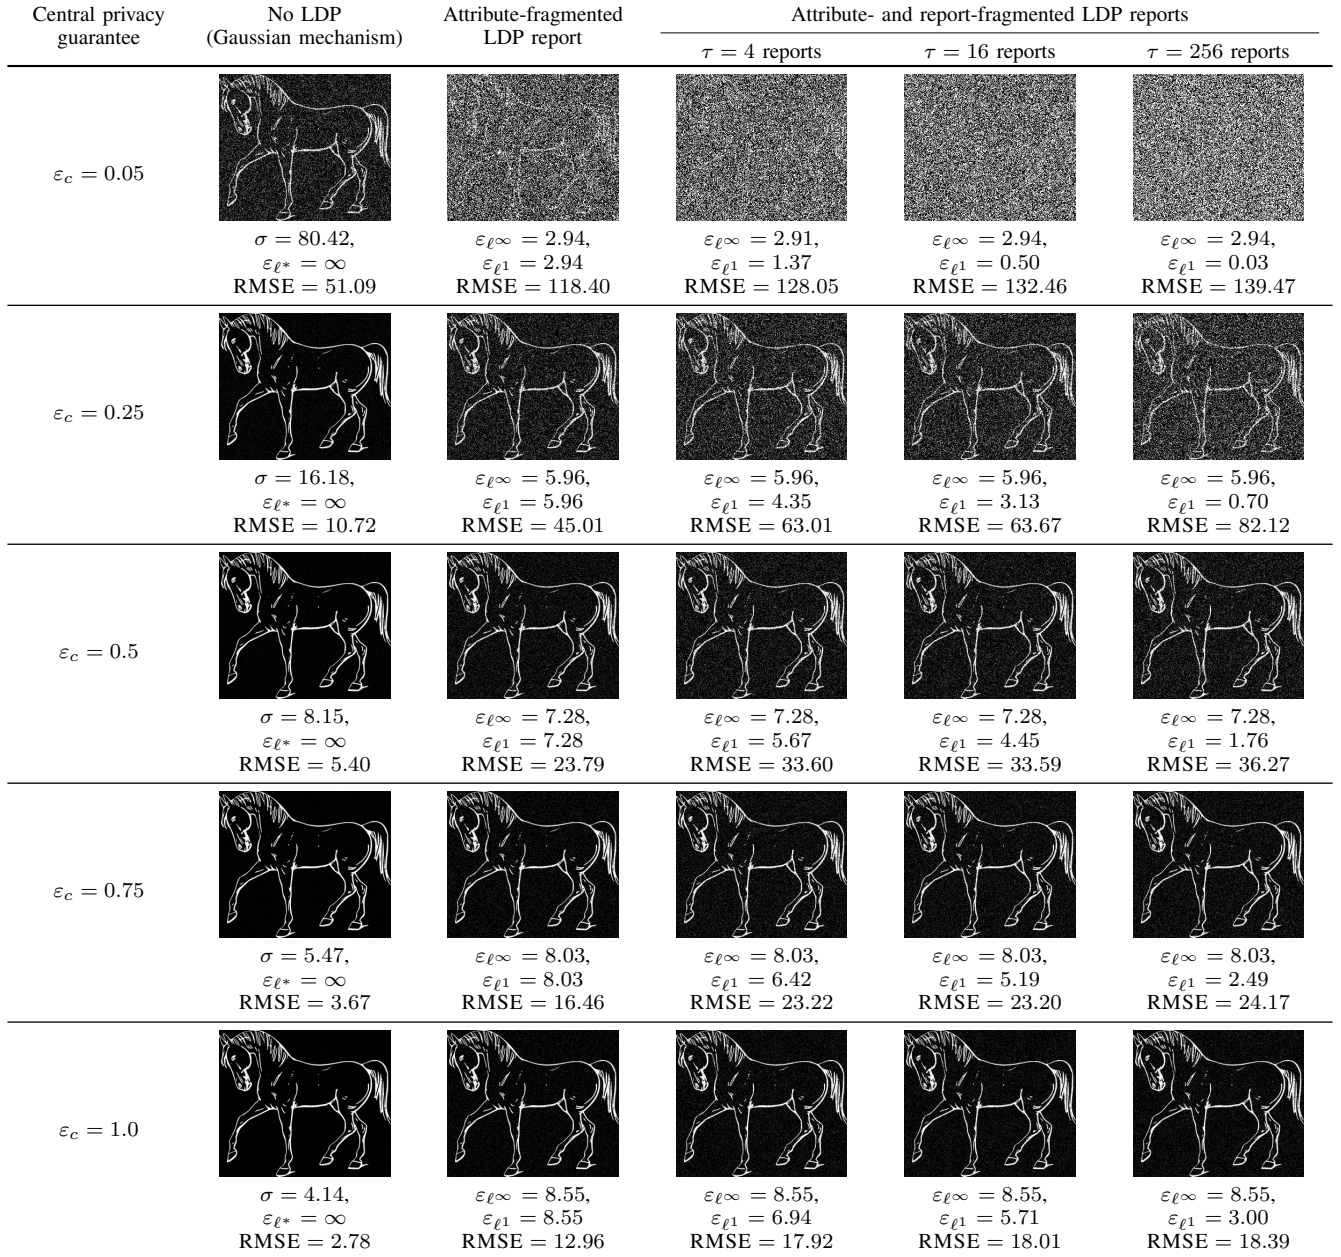<br>$\varepsilon_{\ell^\infty} = 5.96,$<br>$\varepsilon_{\ell^1} = 4.35$<br>RMSE = 63.01   | 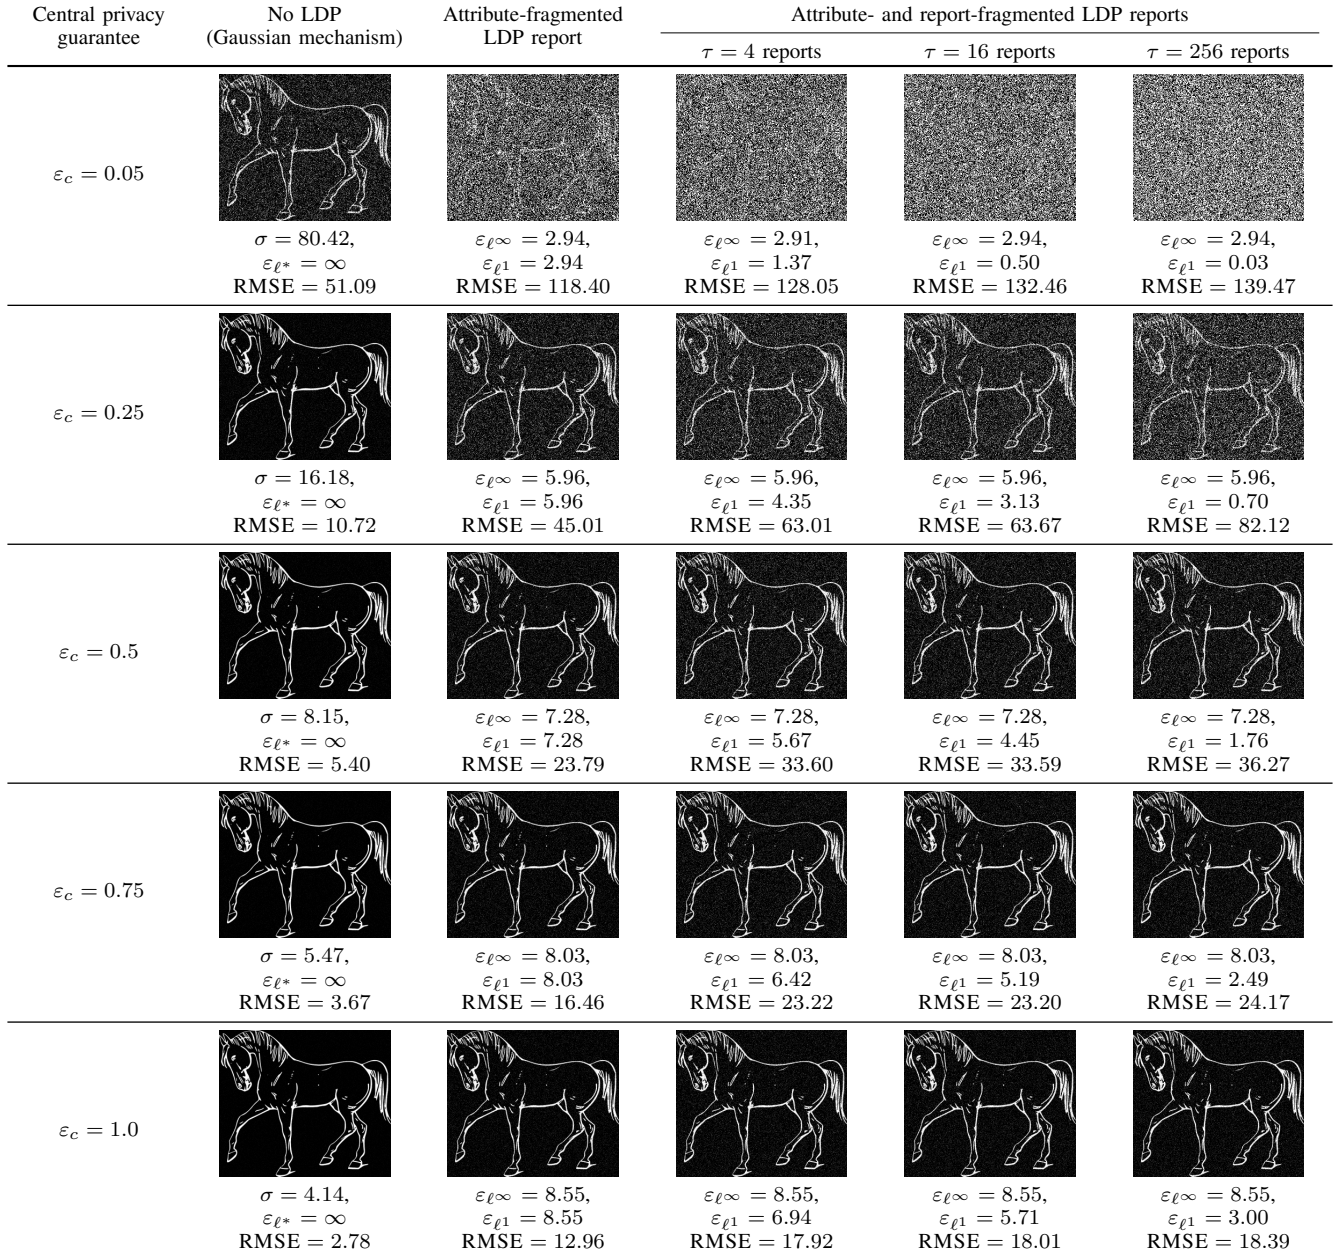<br>$\varepsilon_{\ell^\infty} = 5.96,$<br>$\varepsilon_{\ell^1} = 3.13$<br>RMSE = 63.67   | 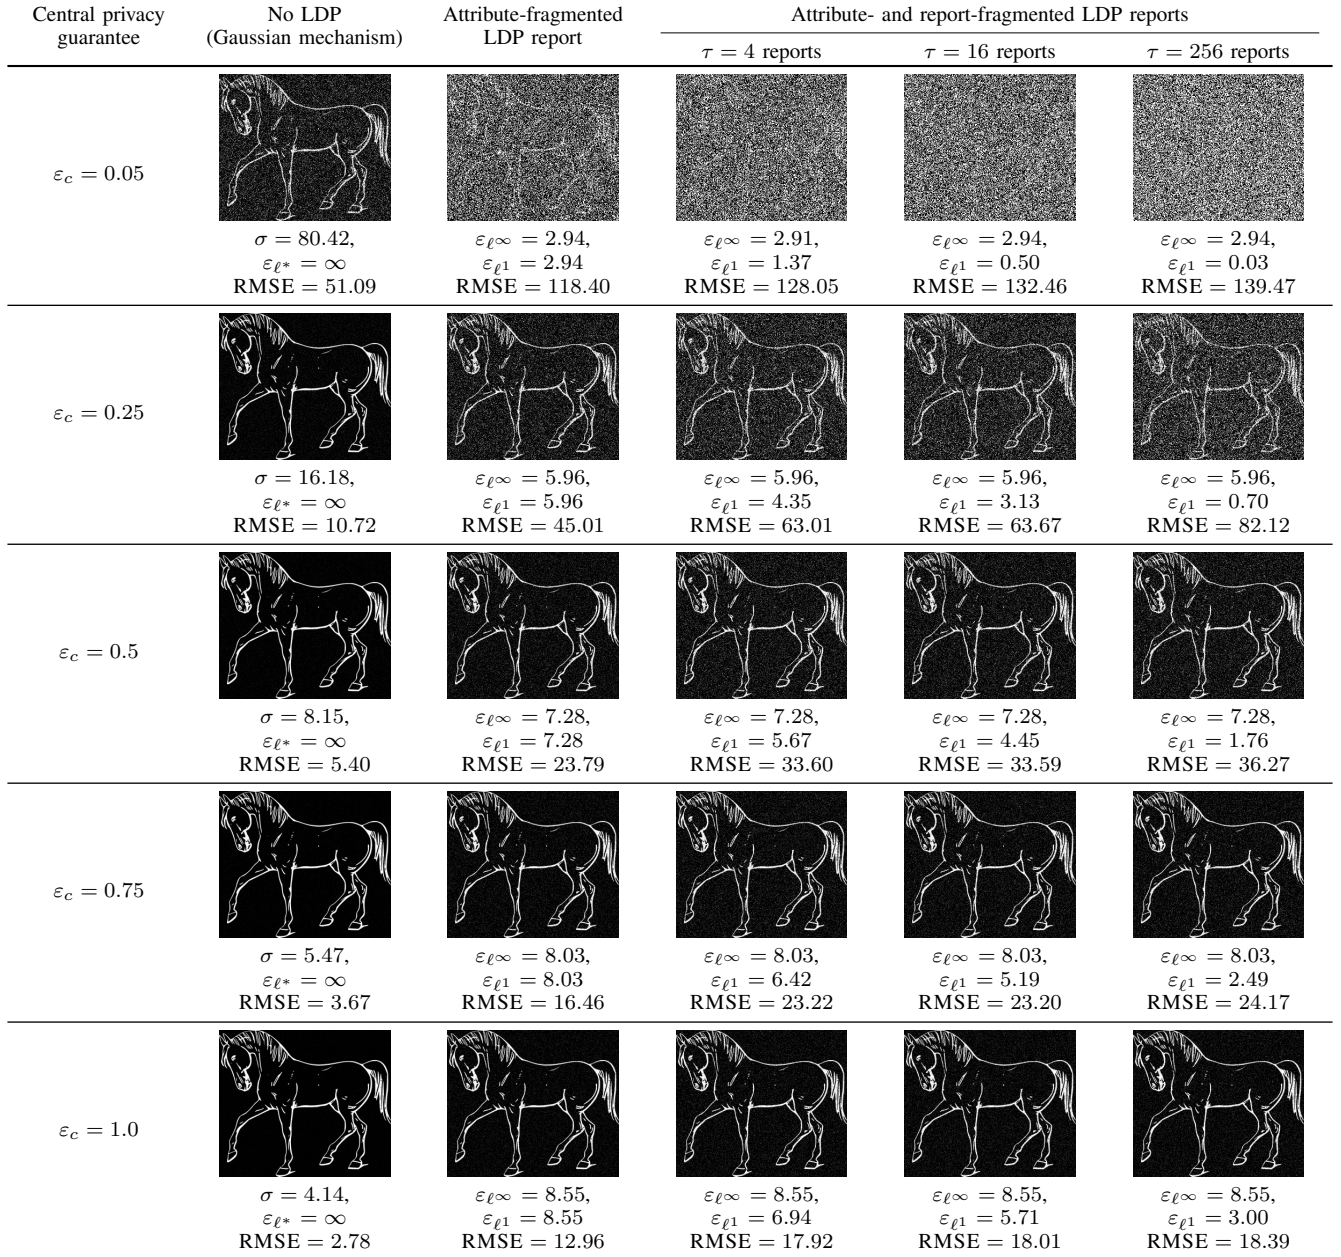<br>$\varepsilon_{\ell^\infty} = 5.96,$<br>$\varepsilon_{\ell^1} = 0.70$<br>RMSE = 82.12   |
| $\varepsilon_c = 0.5$     | 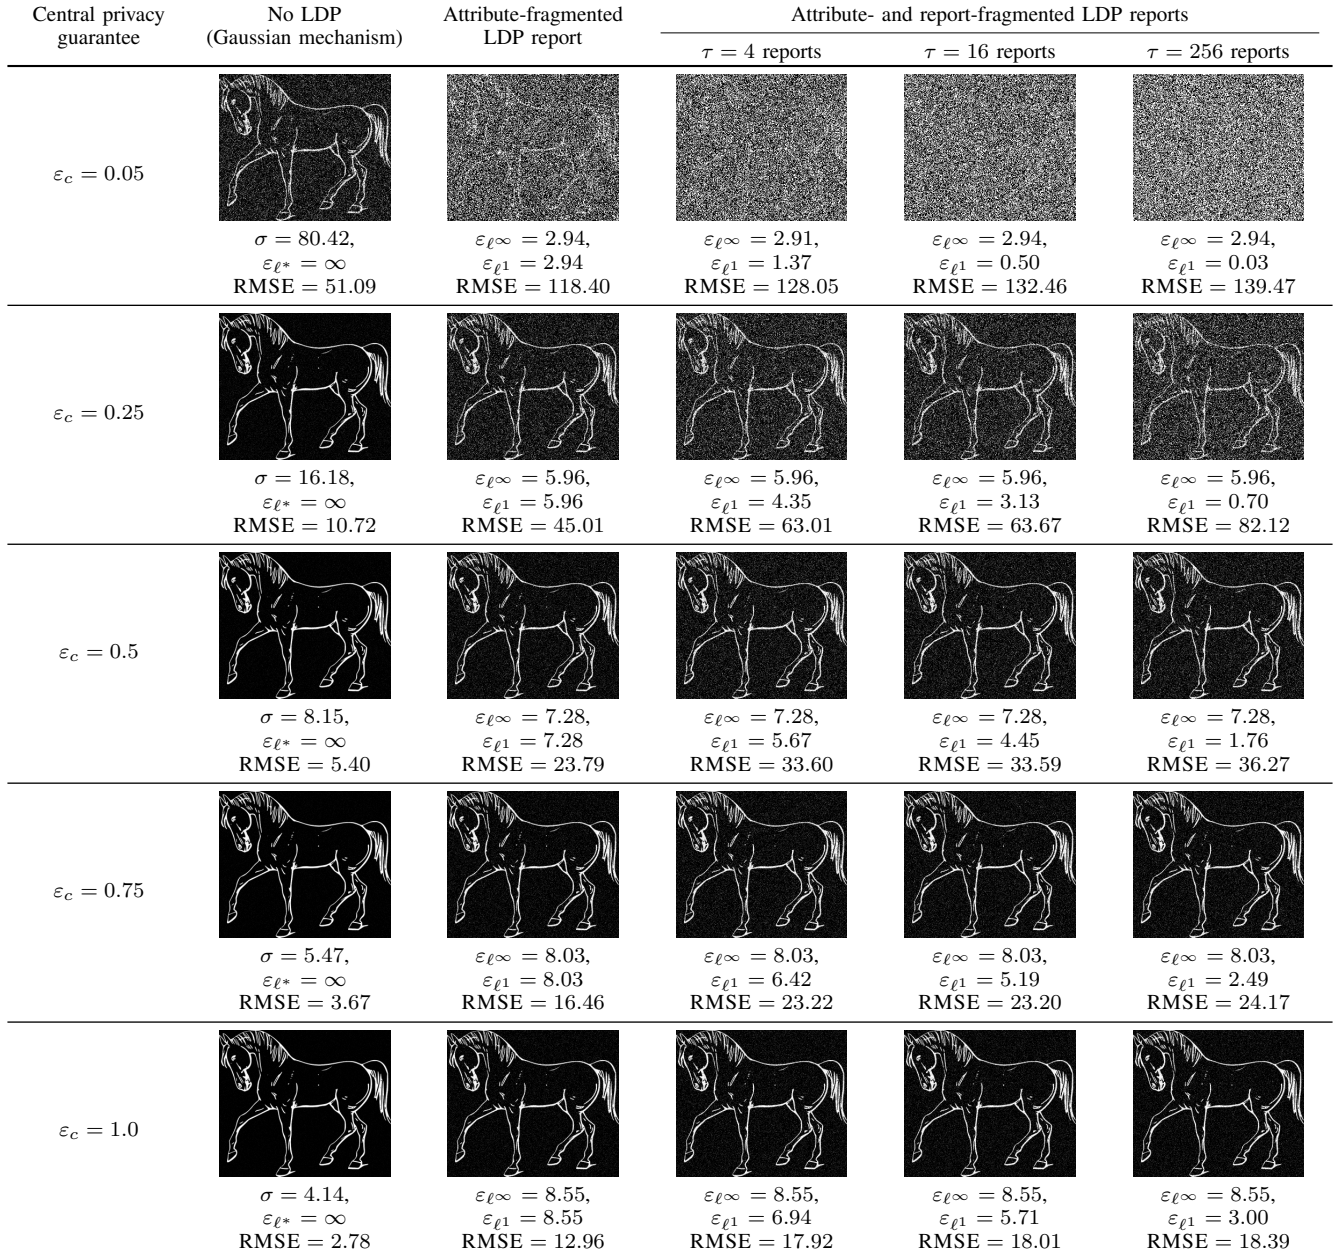<br>$\sigma = 8.15,$<br>$\varepsilon_{\ell^*} = \infty$<br>RMSE = 5.40  | 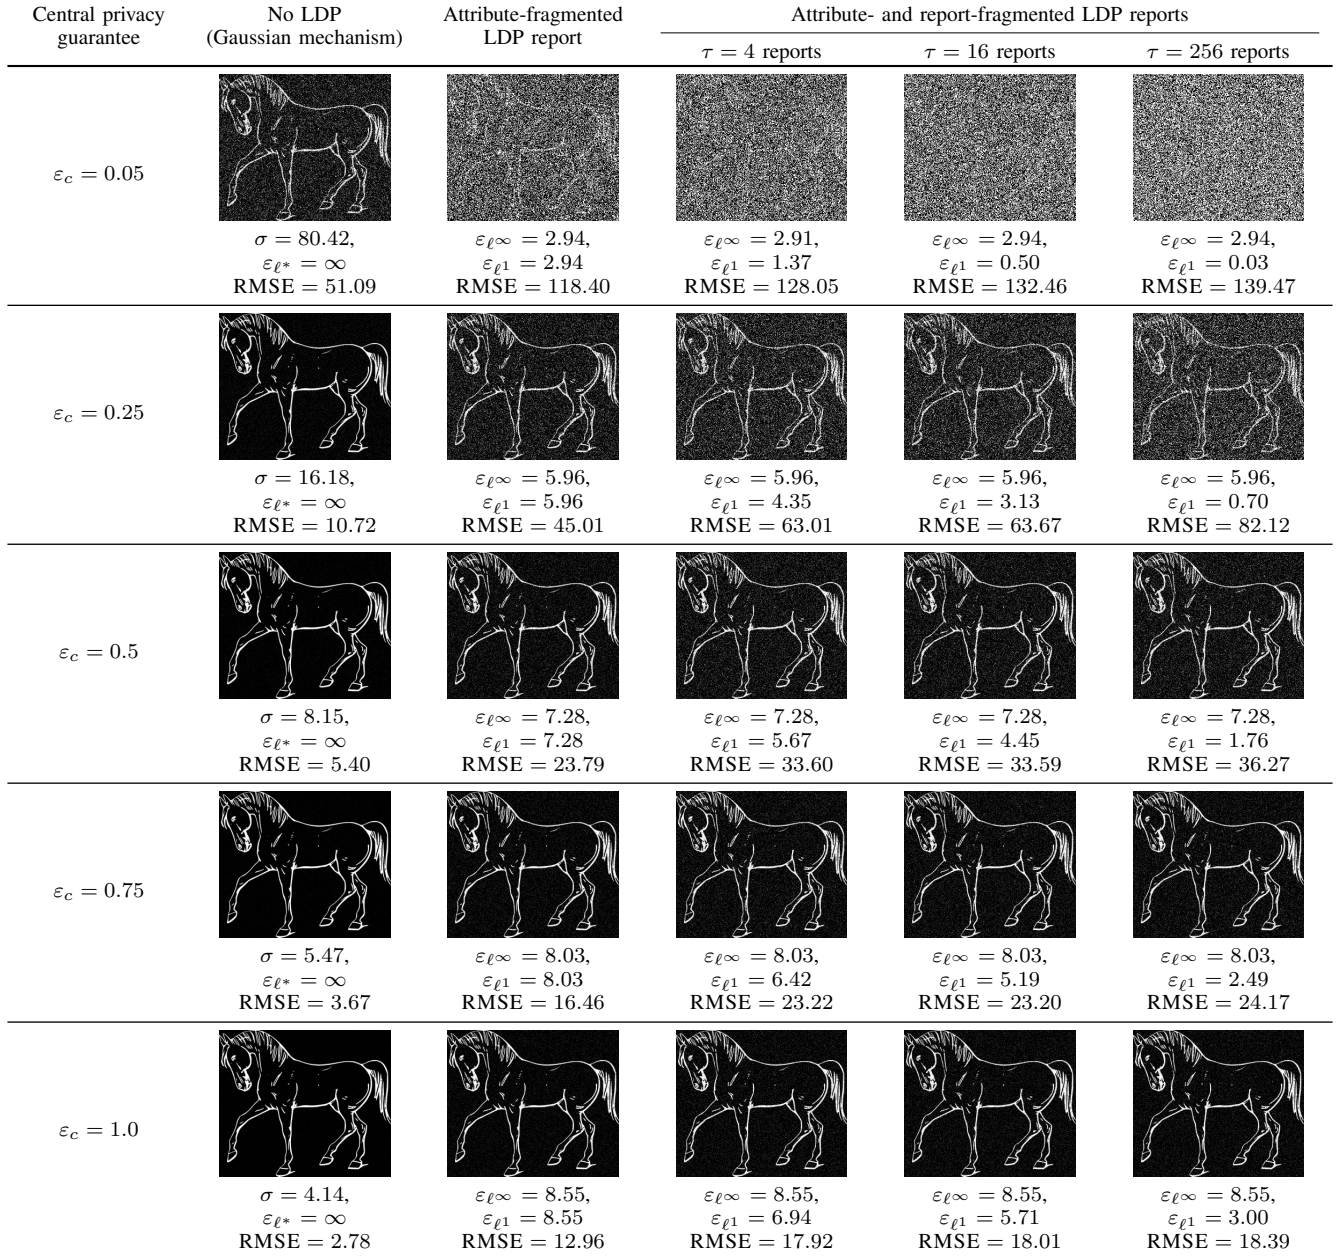<br>$\varepsilon_{\ell^\infty} = 7.28,$<br>$\varepsilon_{\ell^1} = 7.28$<br>RMSE = 23.79  | 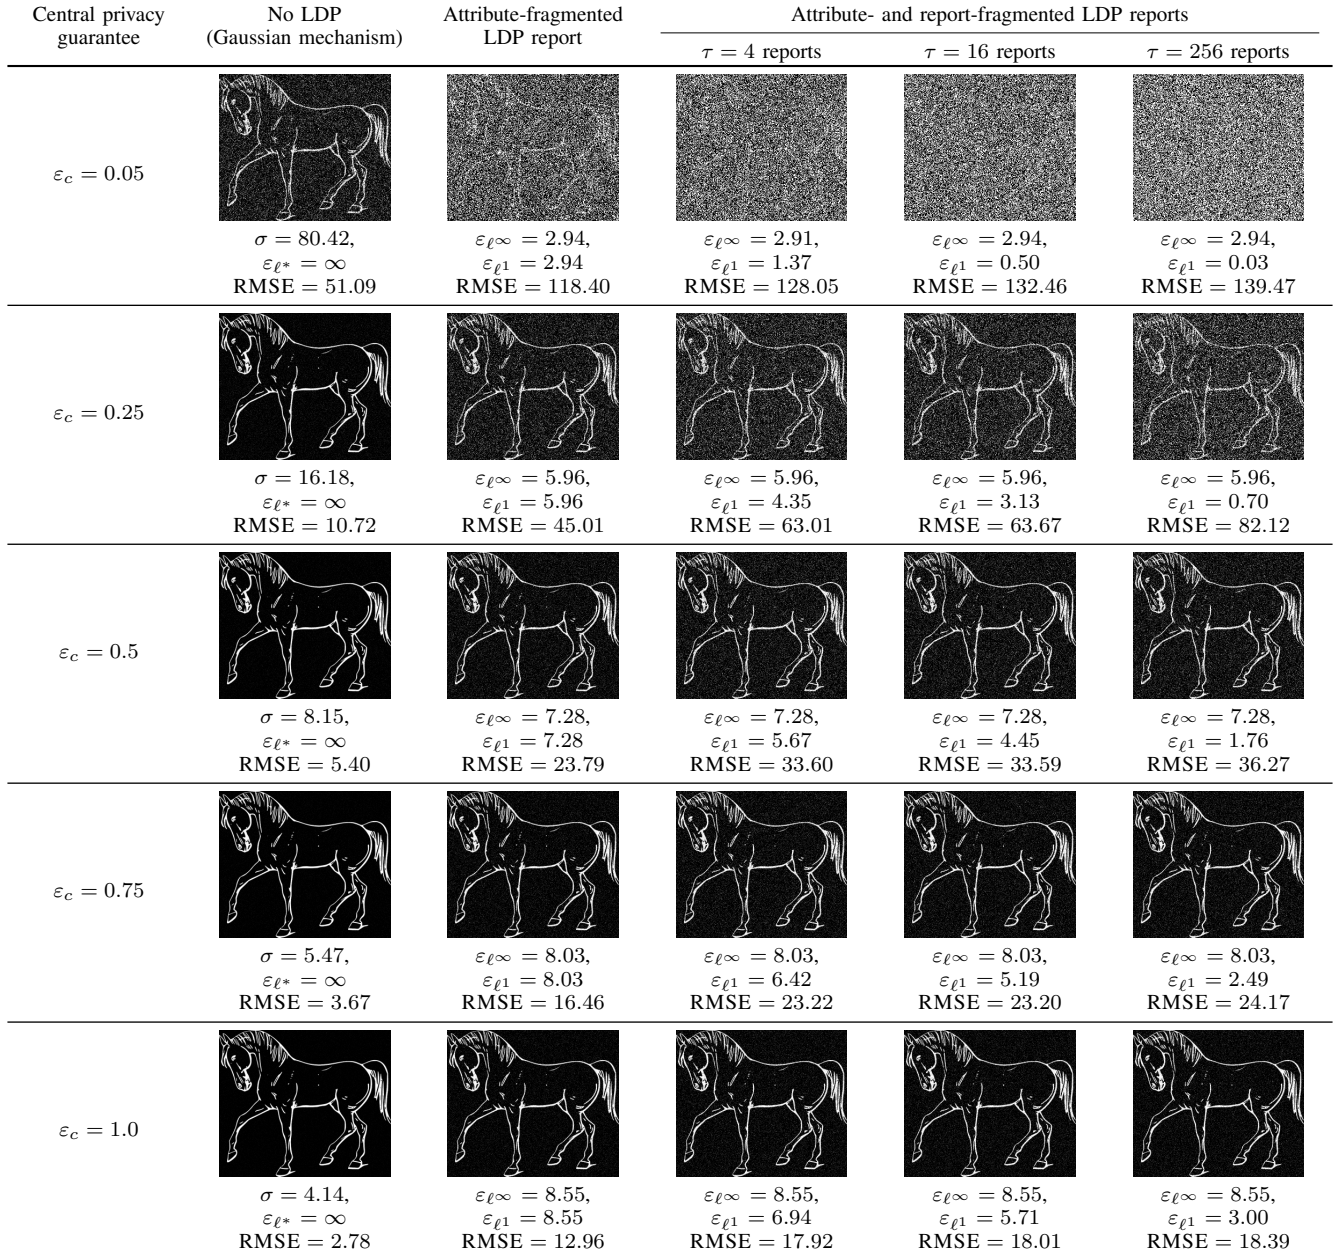<br>$\varepsilon_{\ell^\infty} = 7.28,$<br>$\varepsilon_{\ell^1} = 5.67$<br>RMSE = 33.60  | 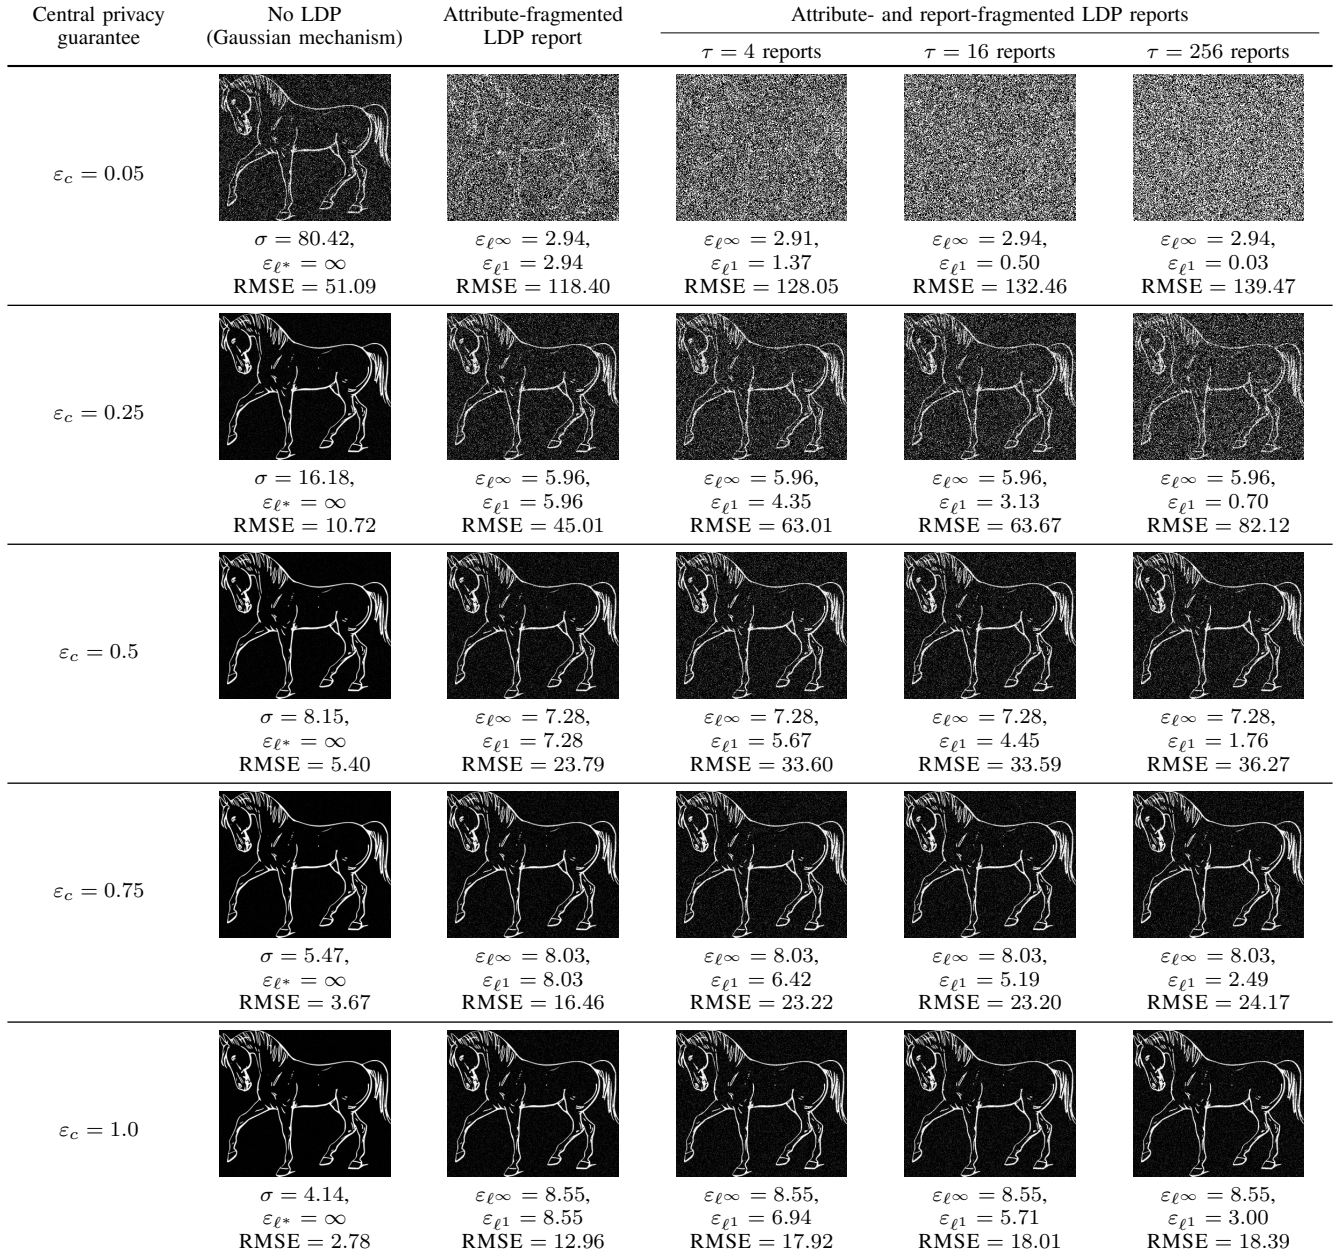<br>$\varepsilon_{\ell^\infty} = 7.28,$<br>$\varepsilon_{\ell^1} = 4.45$<br>RMSE = 33.59  | 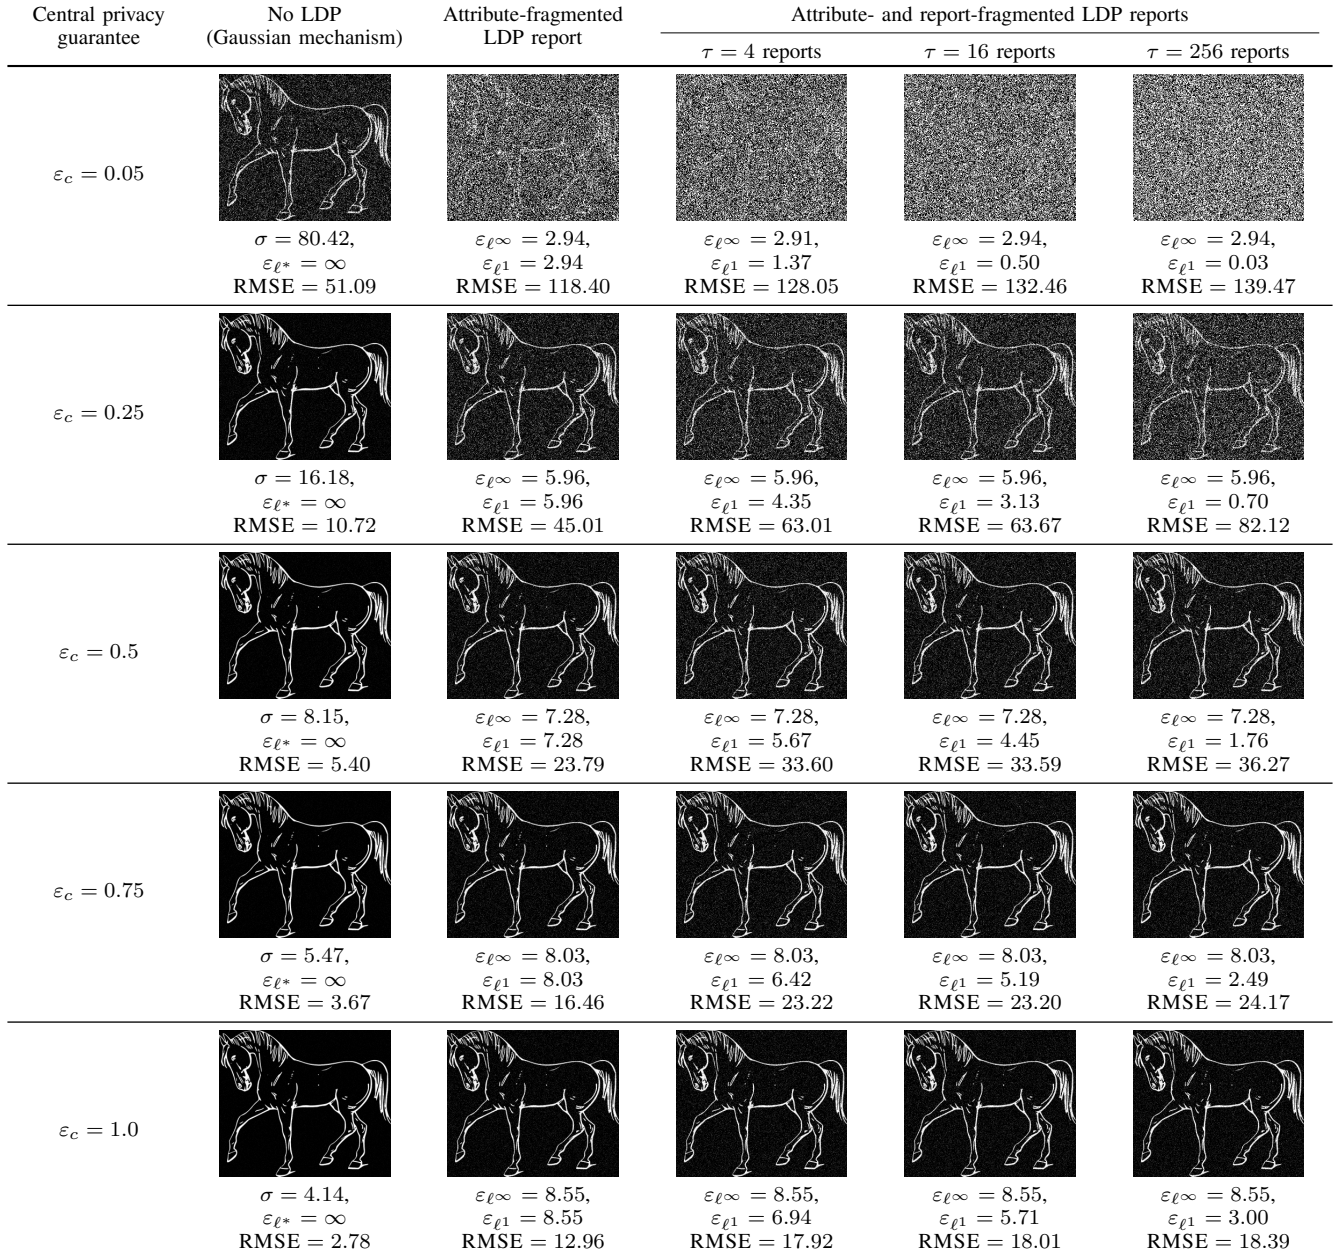<br>$\varepsilon_{\ell^\infty} = 7.28,$<br>$\varepsilon_{\ell^1} = 1.76$<br>RMSE = 36.27  |
| $\varepsilon_c = 0.75$    | 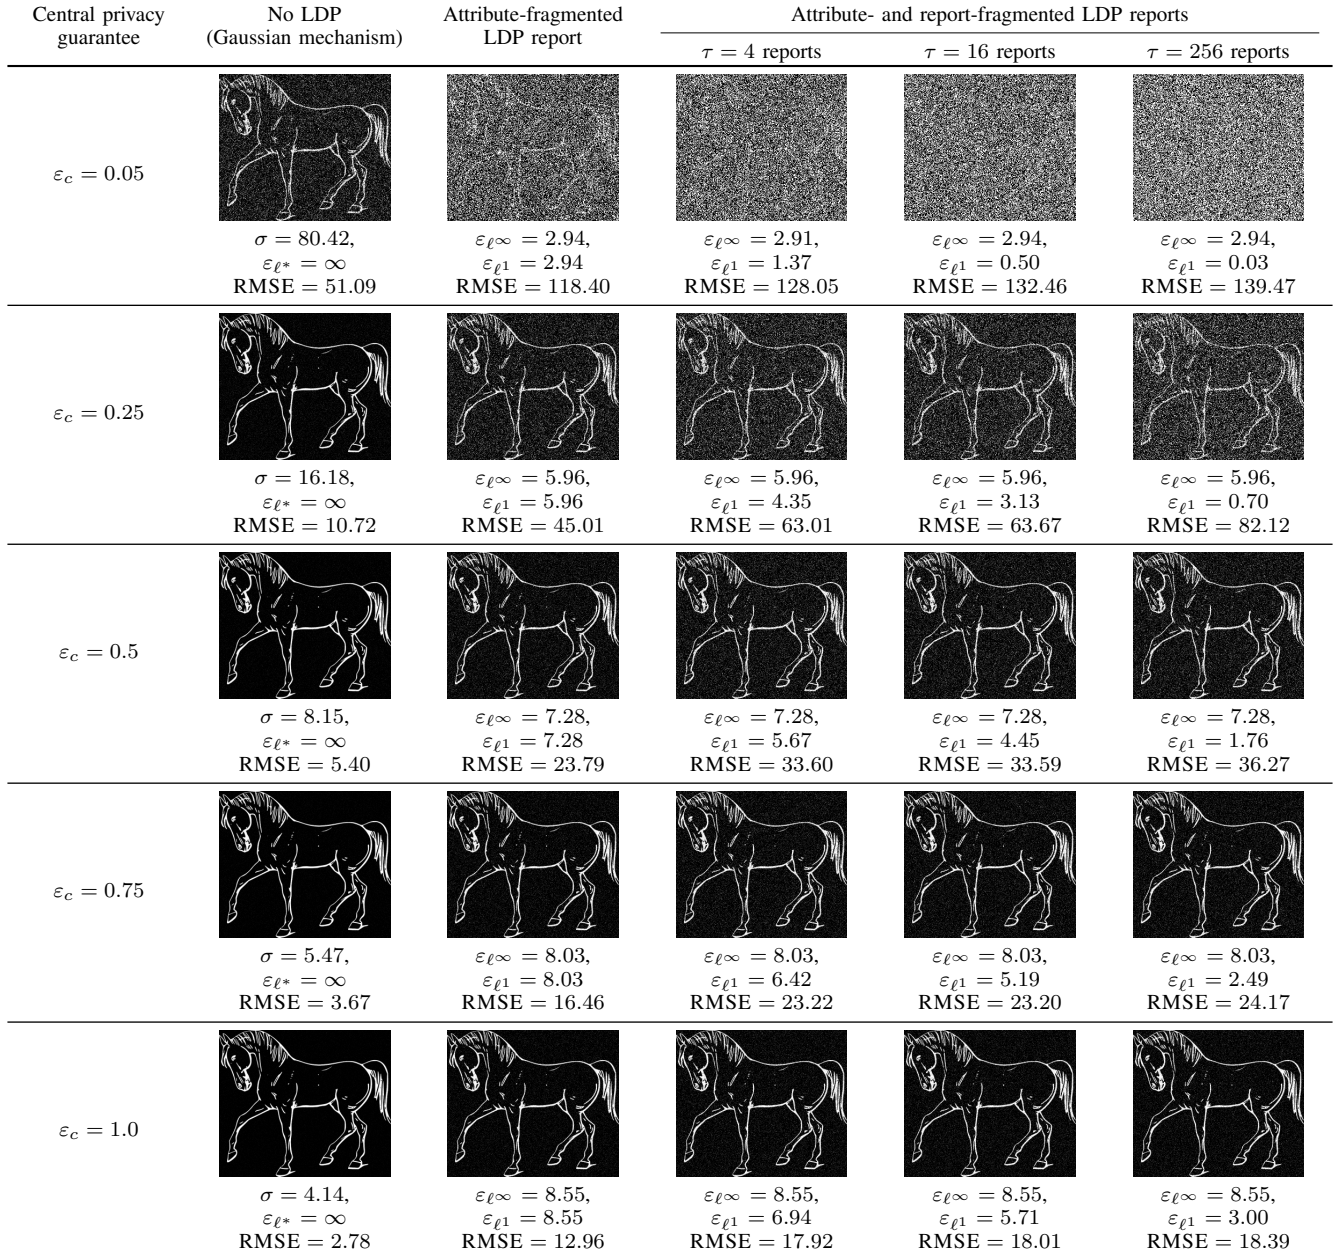<br>$\sigma = 5.47,$<br>$\varepsilon_{\ell^*} = \infty$<br>RMSE = 3.67 | 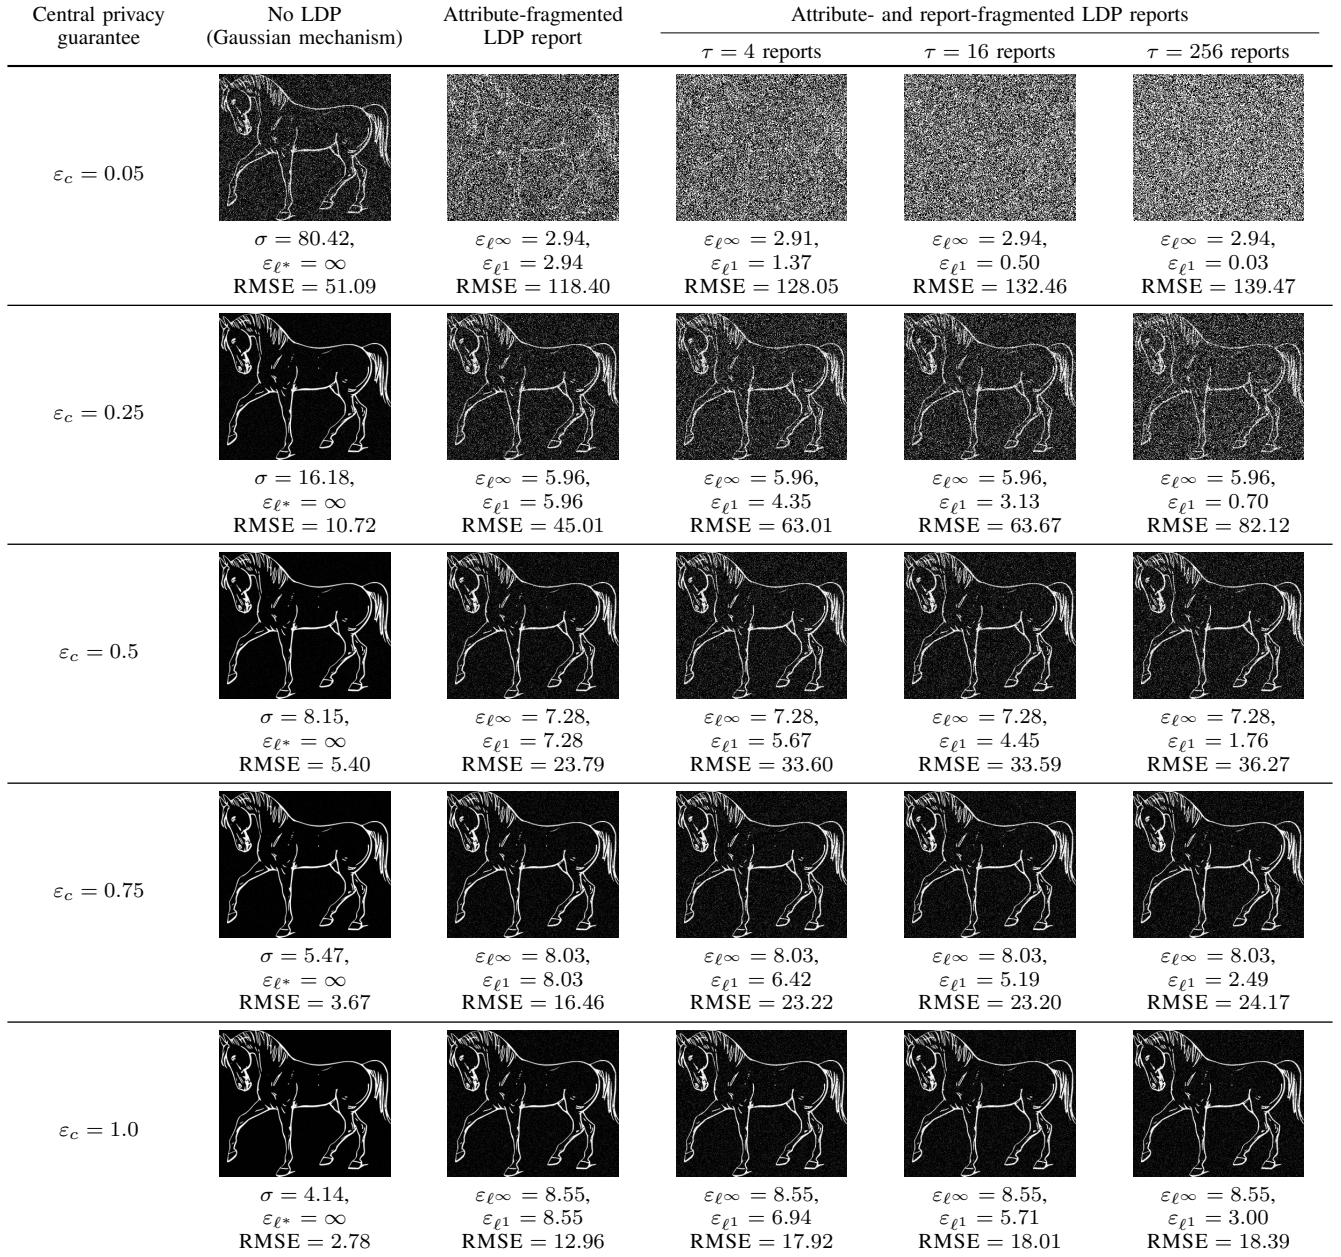<br>$\varepsilon_{\ell^\infty} = 8.03,$<br>$\varepsilon_{\ell^1} = 8.03$<br>RMSE = 16.46 | 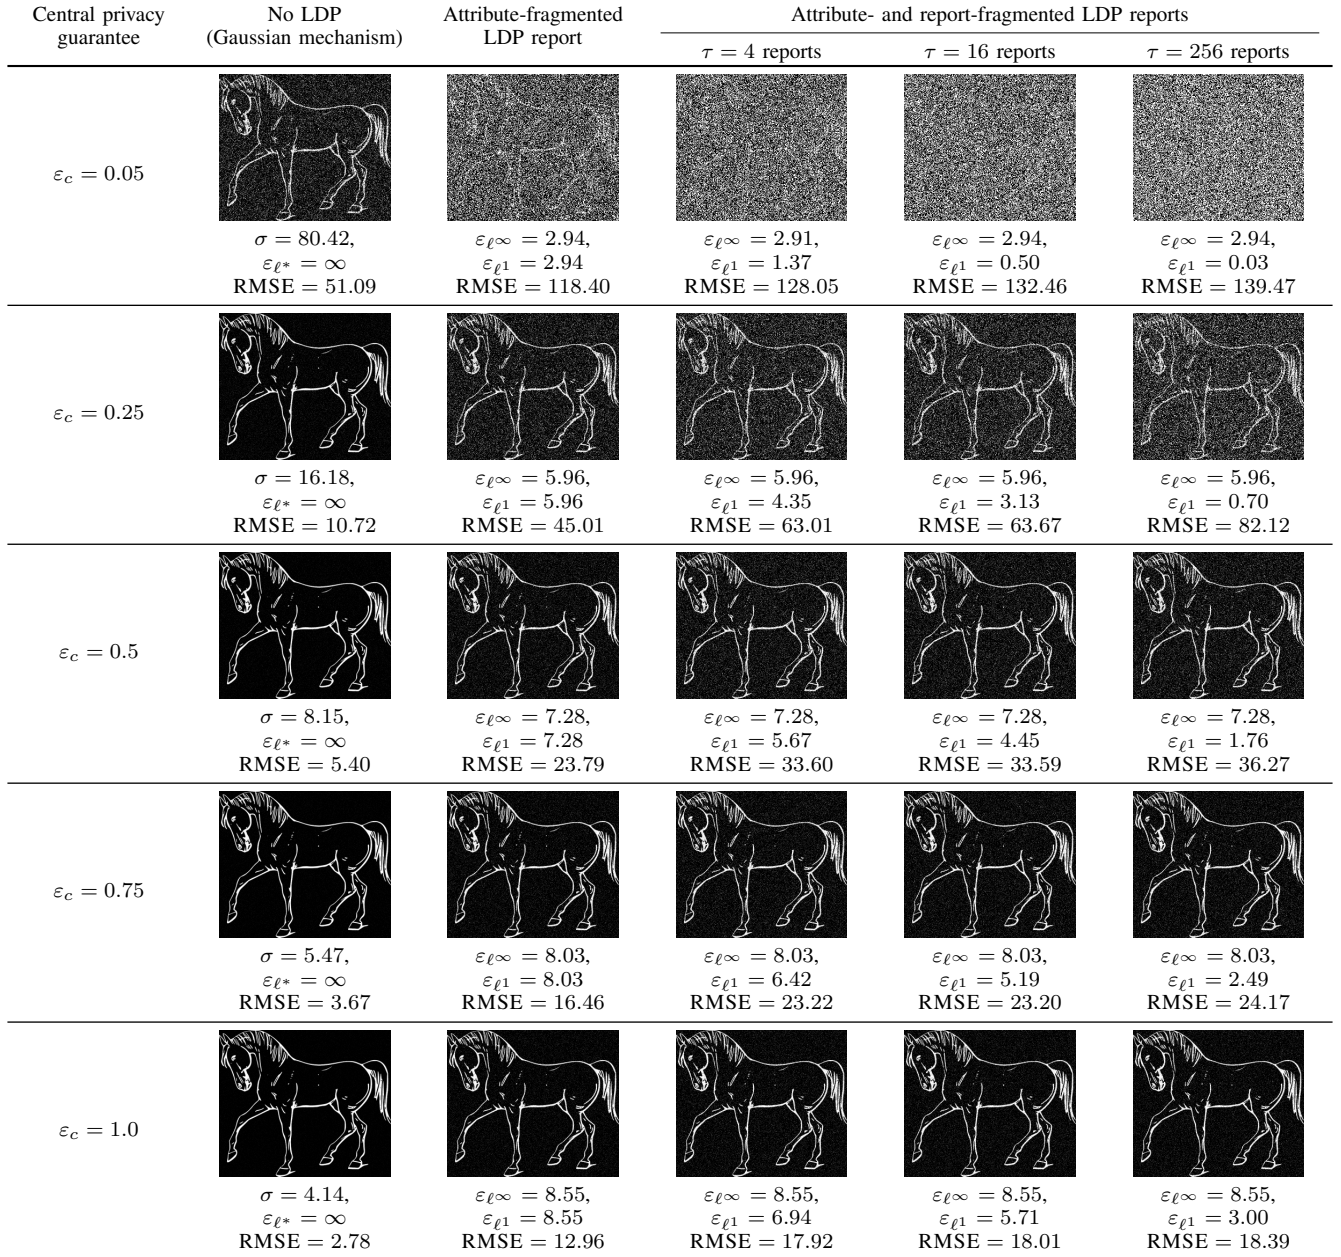<br>$\varepsilon_{\ell^\infty} = 8.03,$<br>$\varepsilon_{\ell^1} = 6.42$<br>RMSE = 23.22 | 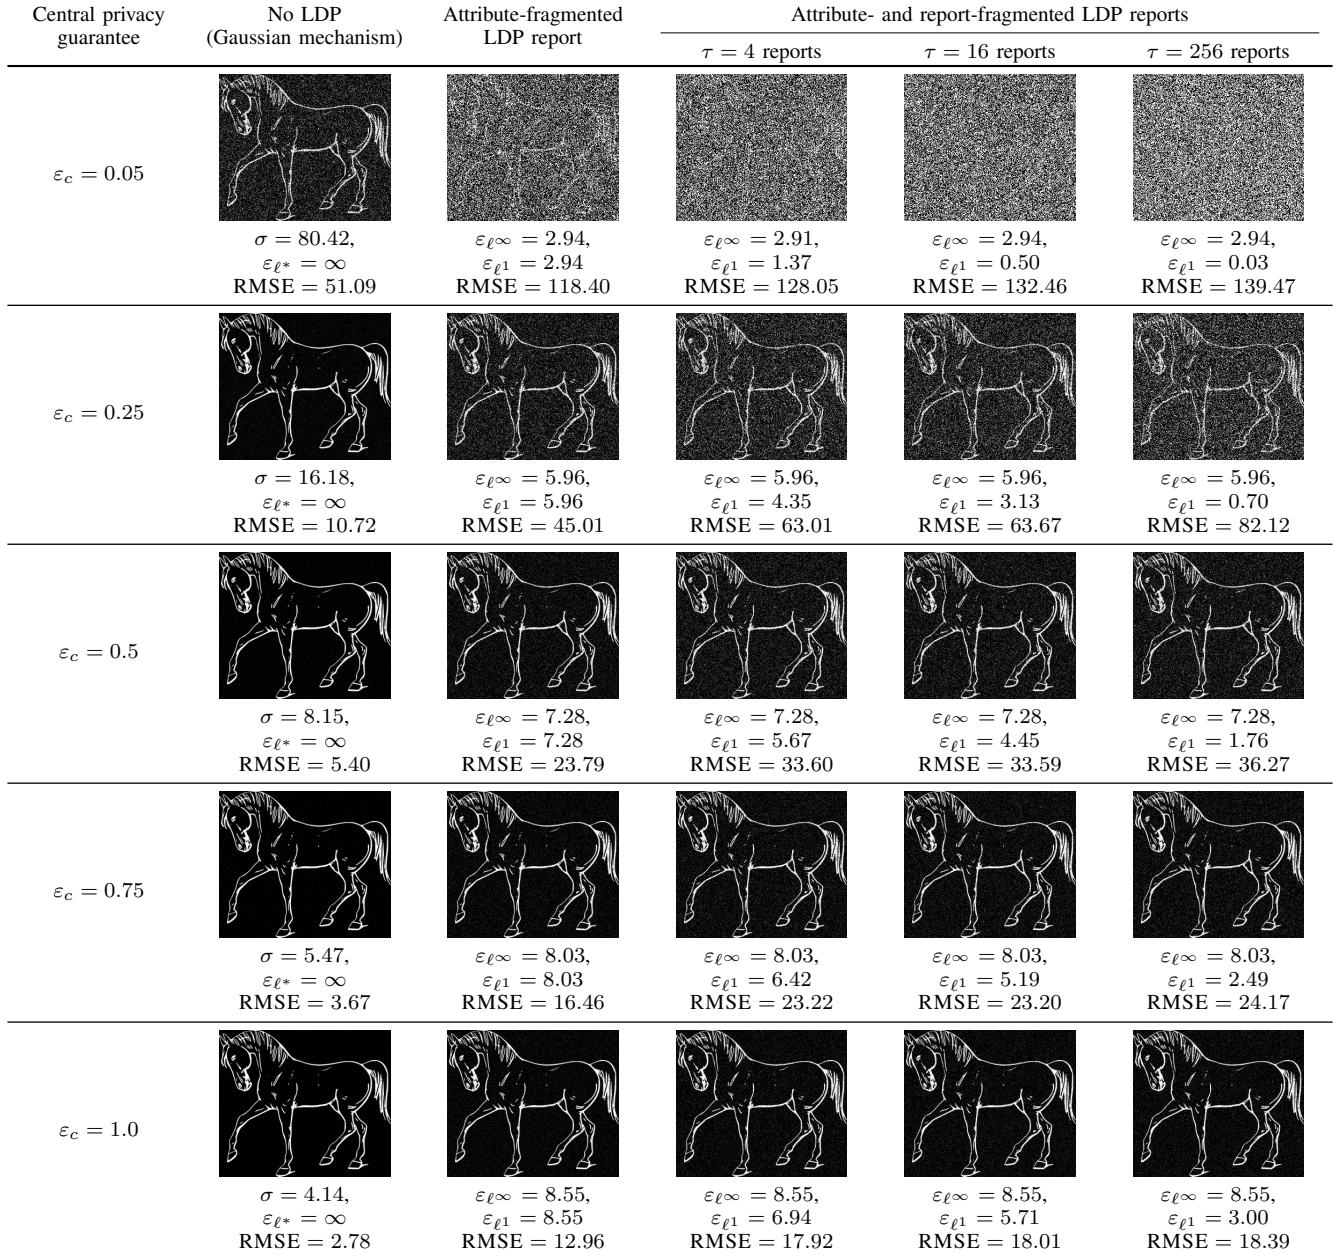<br>$\varepsilon_{\ell^\infty} = 8.03,$<br>$\varepsilon_{\ell^1} = 5.19$<br>RMSE = 23.20 | 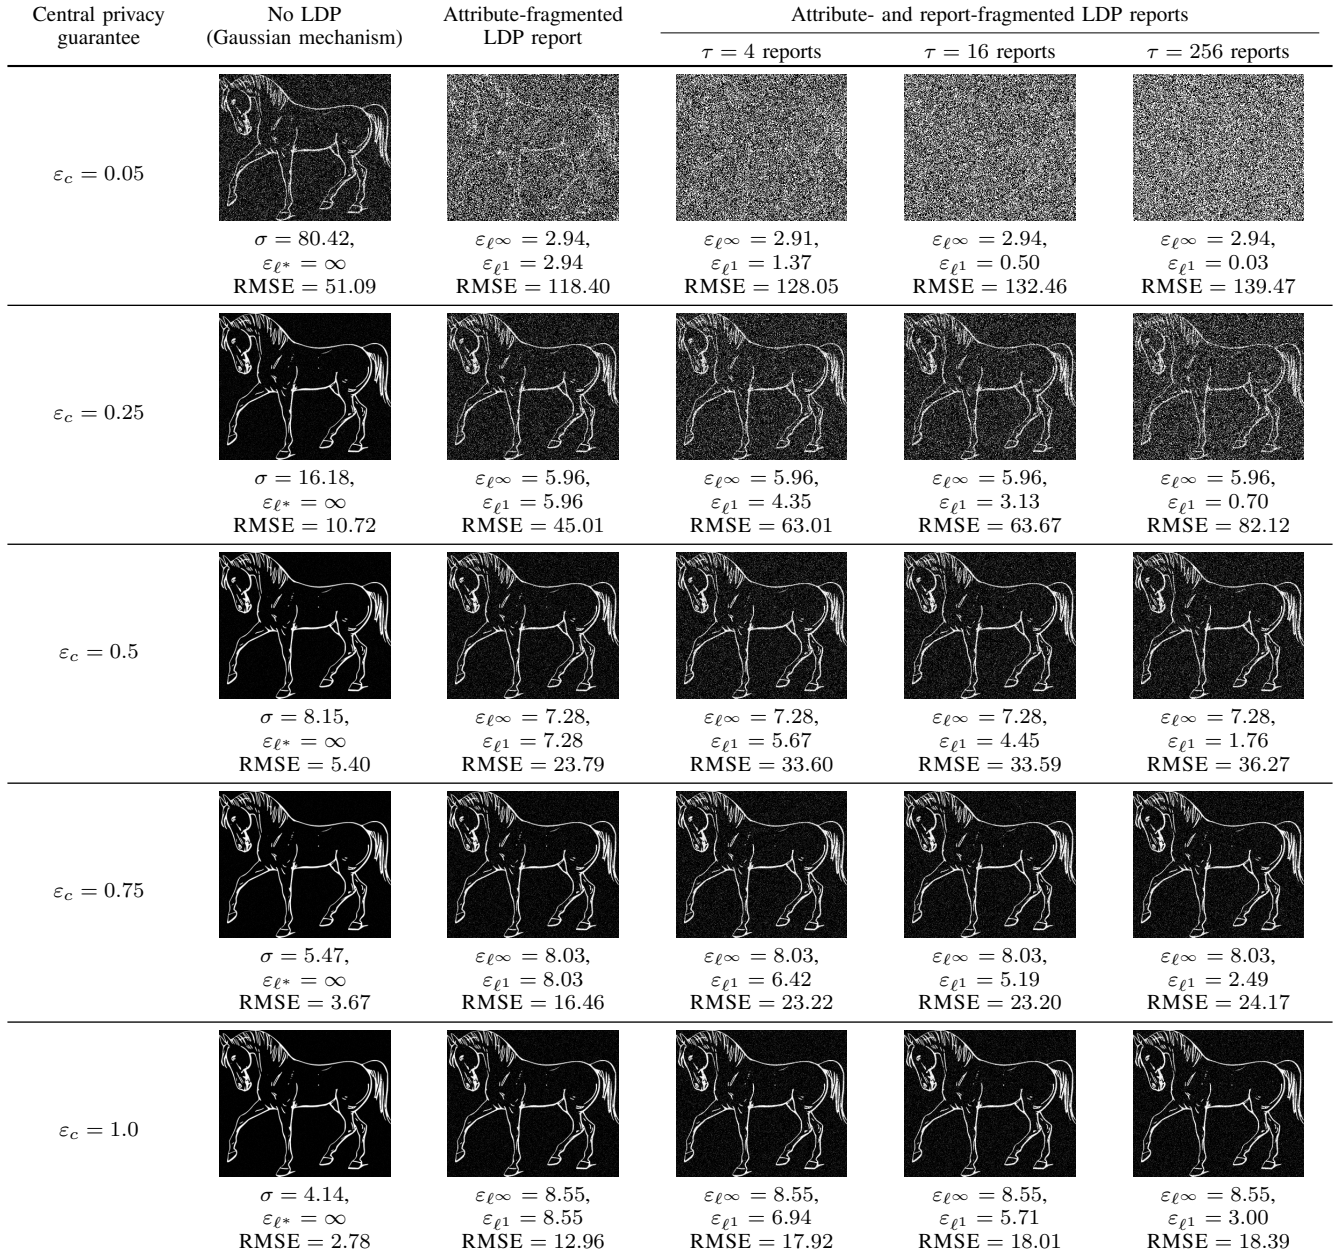<br>$\varepsilon_{\ell^\infty} = 8.03,$<br>$\varepsilon_{\ell^1} = 2.49$<br>RMSE = 24.17 |
| $\varepsilon_c = 1.0$     | 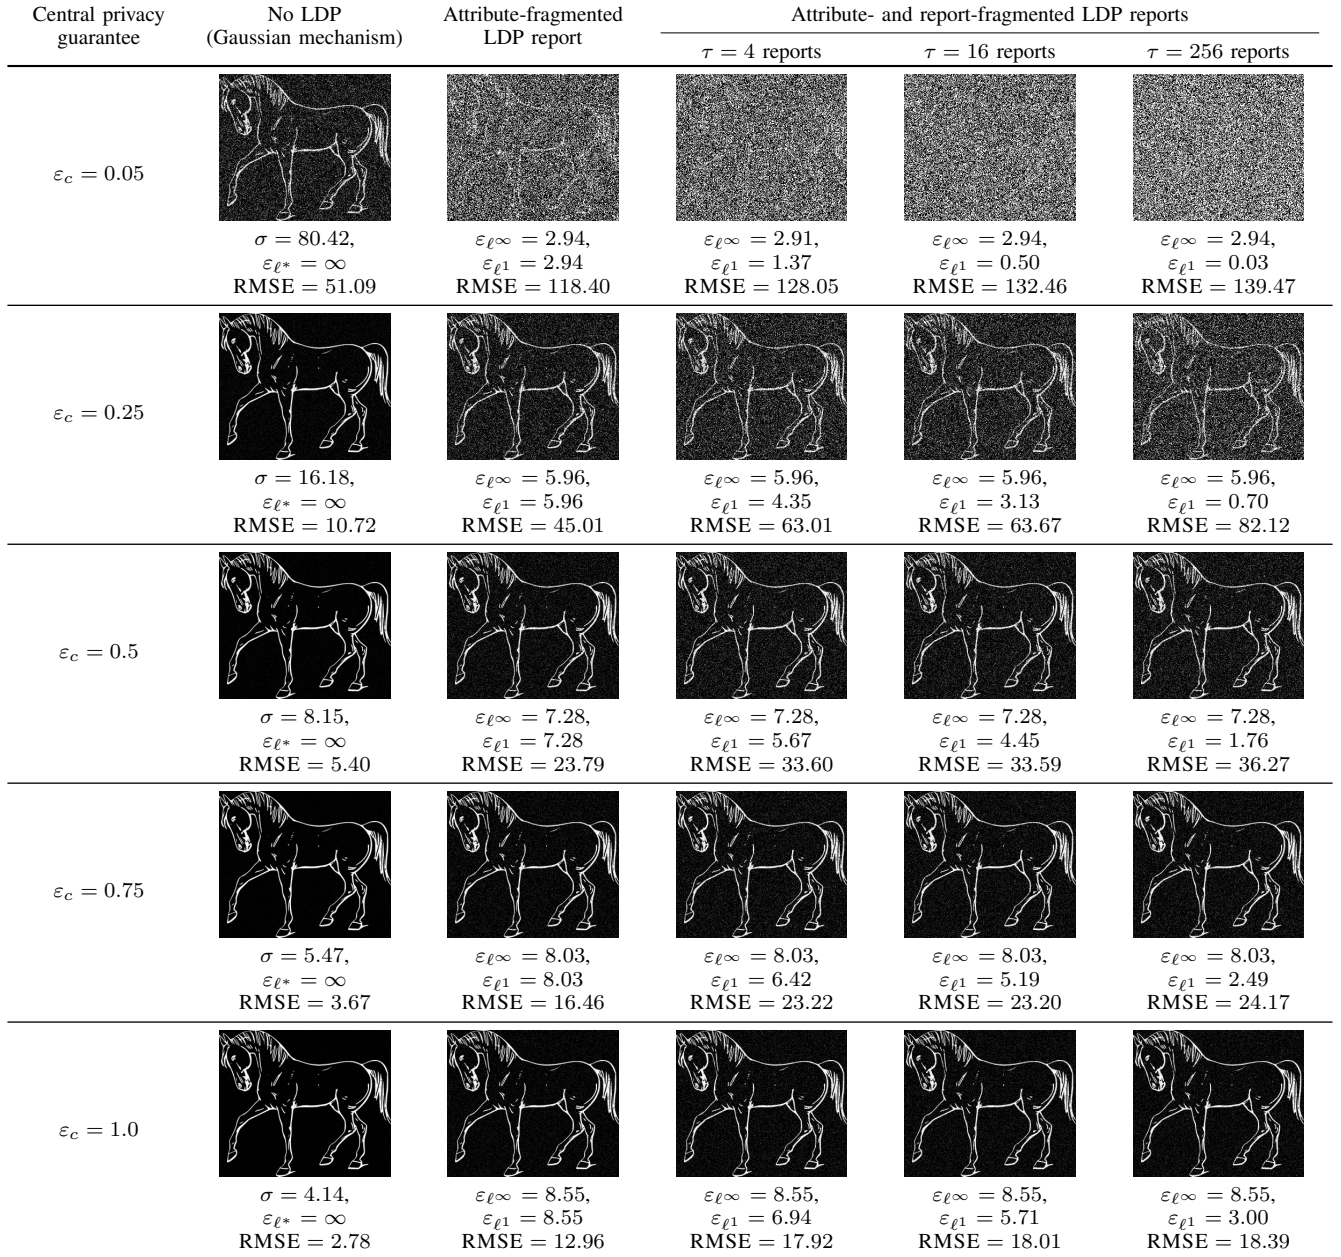<br>$\sigma = 4.14,$<br>$\varepsilon_{\ell^*} = \infty$<br>RMSE = 2.78 | 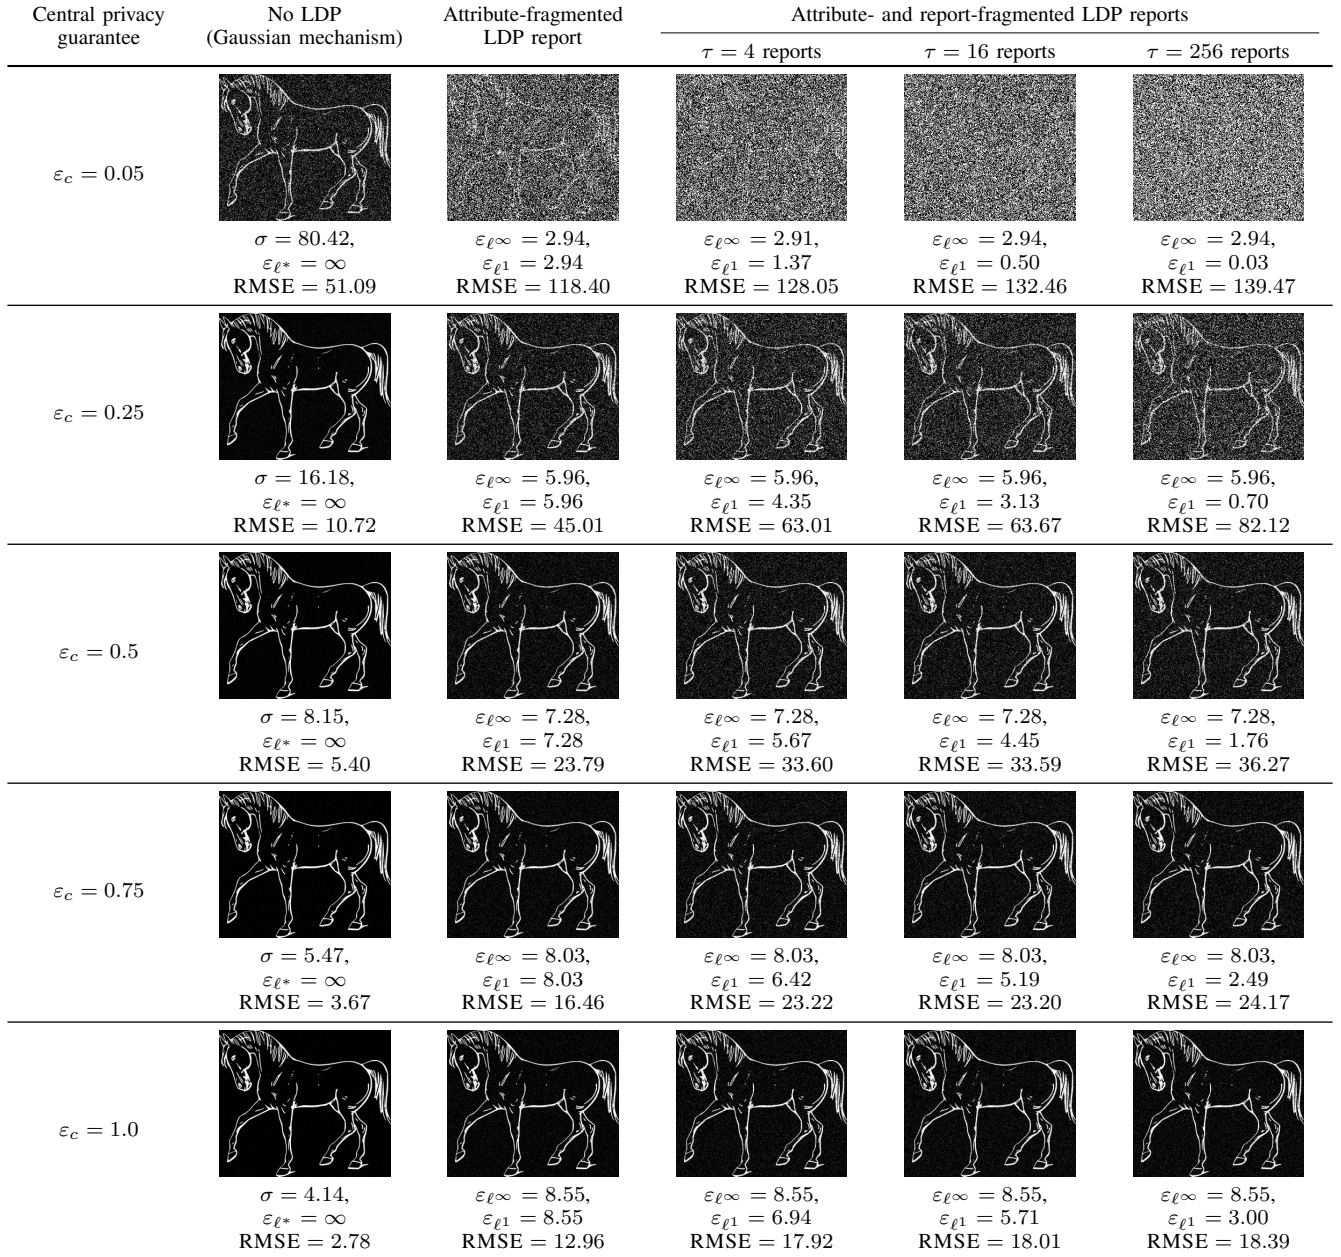<br>$\varepsilon_{\ell^\infty} = 8.55,$<br>$\varepsilon_{\ell^1} = 8.55$<br>RMSE = 12.96 | 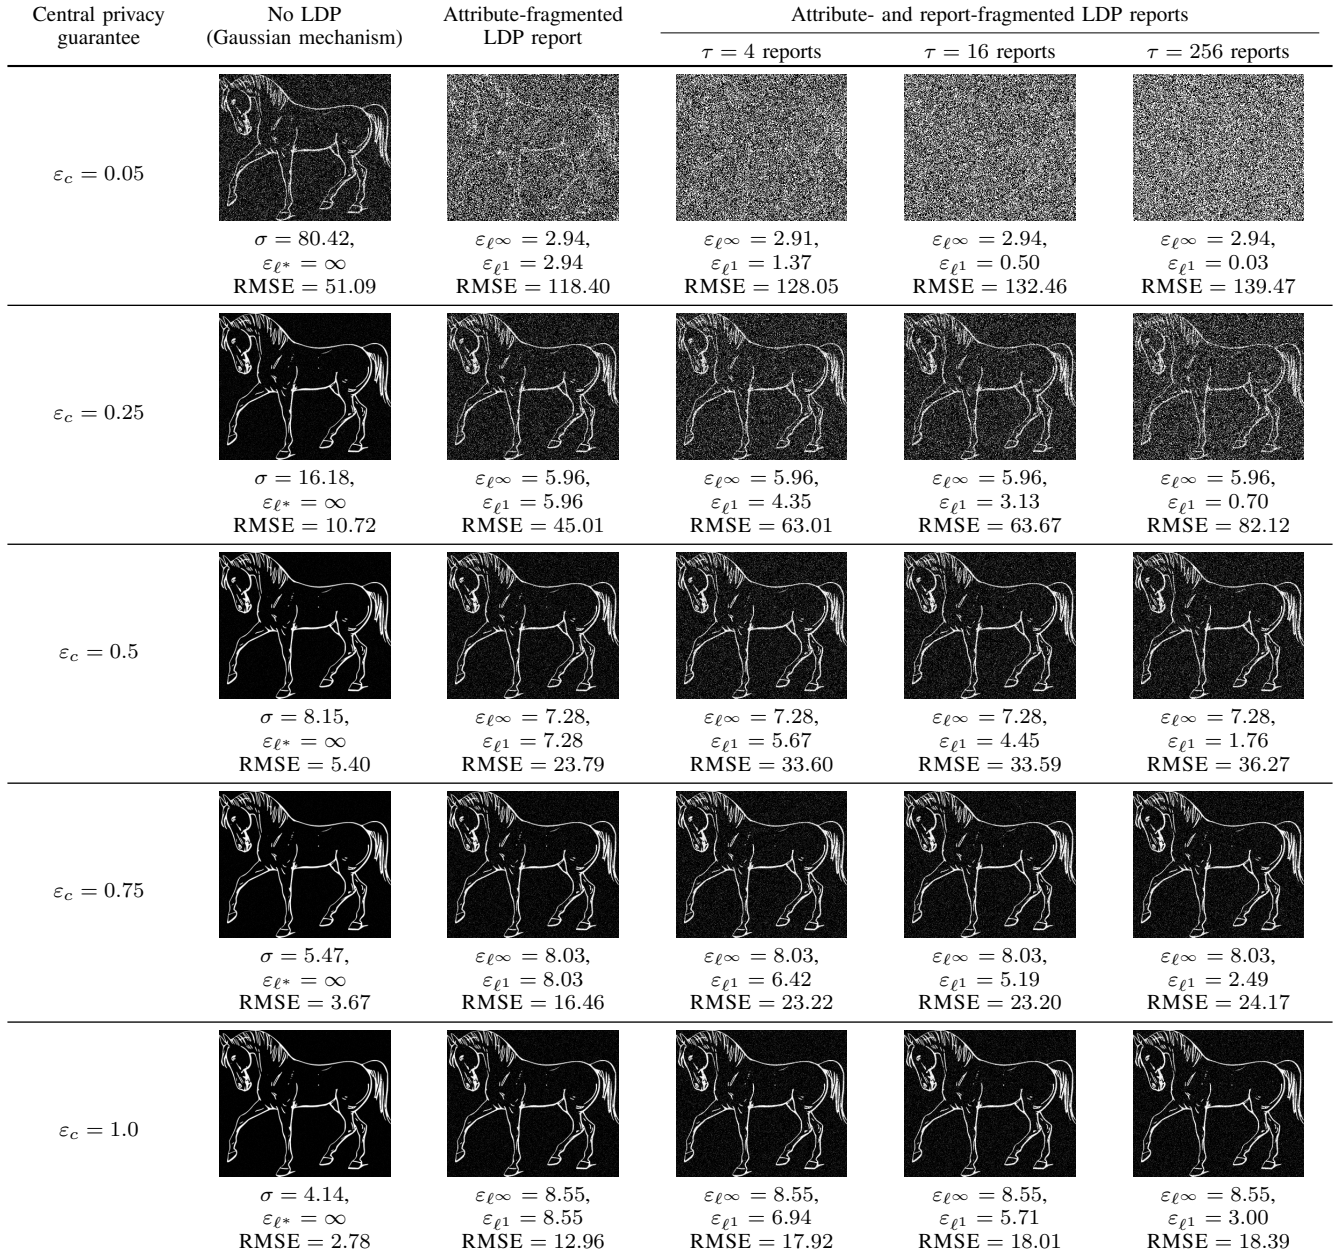<br>$\varepsilon_{\ell^\infty} = 8.55,$<br>$\varepsilon_{\ell^1} = 6.94$<br>RMSE = 17.92 | 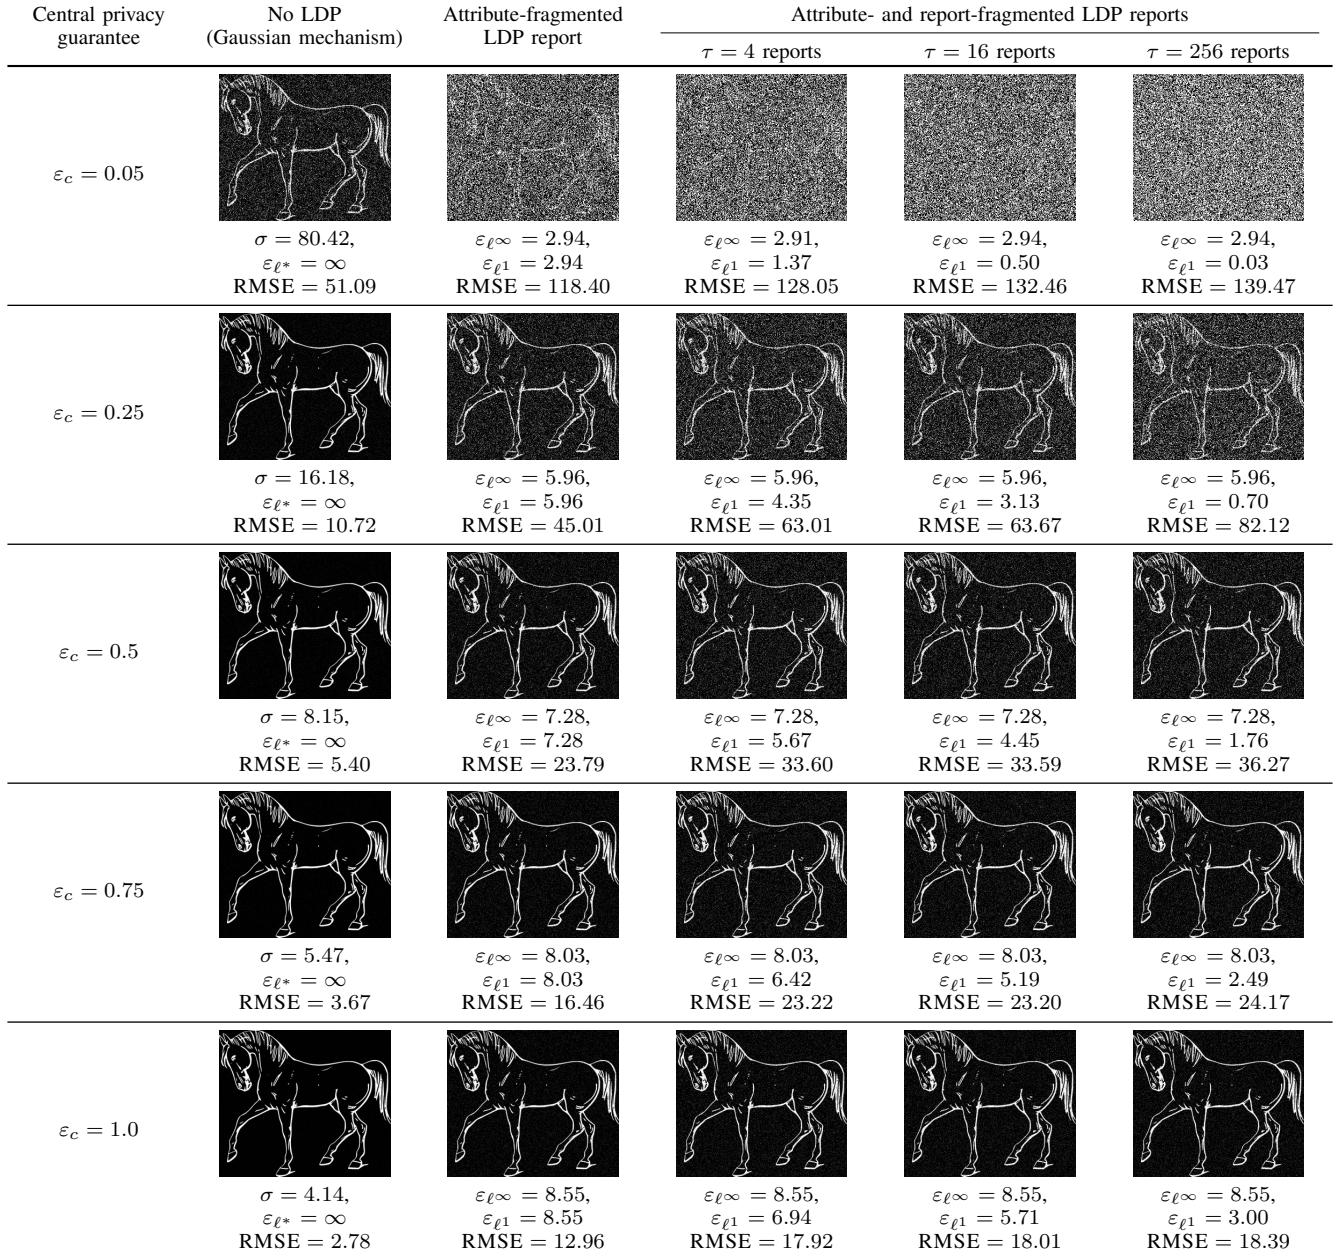<br>$\varepsilon_{\ell^\infty} = 8.55,$<br>$\varepsilon_{\ell^1} = 5.71$<br>RMSE = 18.01 | 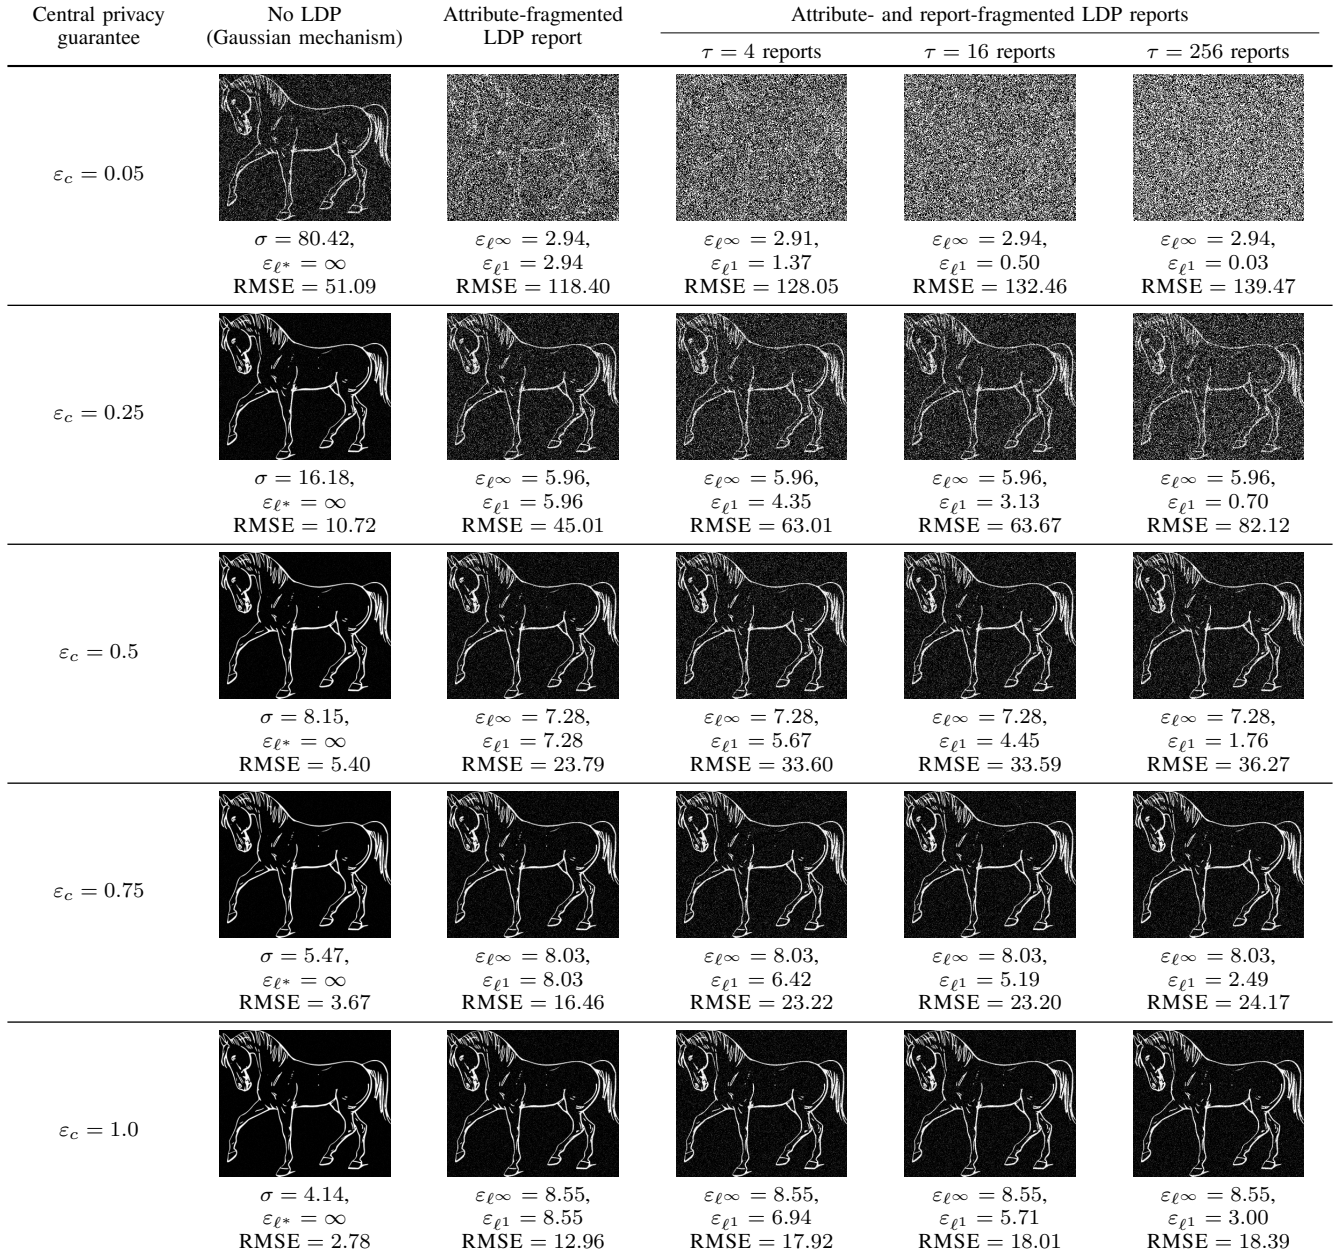<br>$\varepsilon_{\ell^\infty} = 8.55,$<br>$\varepsilon_{\ell^1} = 3.00$<br>RMSE = 18.39 |

TABLE V: Experimental results of reconstructing the Horse image dataset by varying  $\varepsilon_c$  and evaluating a central DP mechanism, attribute fragmenting, and both attribute and report fragmenting achieving  $(\varepsilon_c, \delta_c)$ -central DP with  $\delta_c = 5 \times 10^{-8}$ . Using count sketch with 1024 hash functions and sketch size 65536. In the last row, we present a non-private baseline to demonstrate the estimation error introduced by the sketching algorithm.

| Central privacy guarantee                               | Attribute-fragmented LDP report                                                                                                                                            | Attribute- and report-fragmented LDP reports                                                                                                                               |                                                                                                                                                                             |                                                                                                                                                                              |
|---------------------------------------------------------|----------------------------------------------------------------------------------------------------------------------------------------------------------------------------|----------------------------------------------------------------------------------------------------------------------------------------------------------------------------|-----------------------------------------------------------------------------------------------------------------------------------------------------------------------------|------------------------------------------------------------------------------------------------------------------------------------------------------------------------------|
|                                                         |                                                                                                                                                                            | $\tau = 4$ reports                                                                                                                                                         | $\tau = 16$ reports                                                                                                                                                         | $\tau = 256$ reports                                                                                                                                                         |
| $0.05 \leq \varepsilon_c \leq \varepsilon_{\ell\infty}$ | 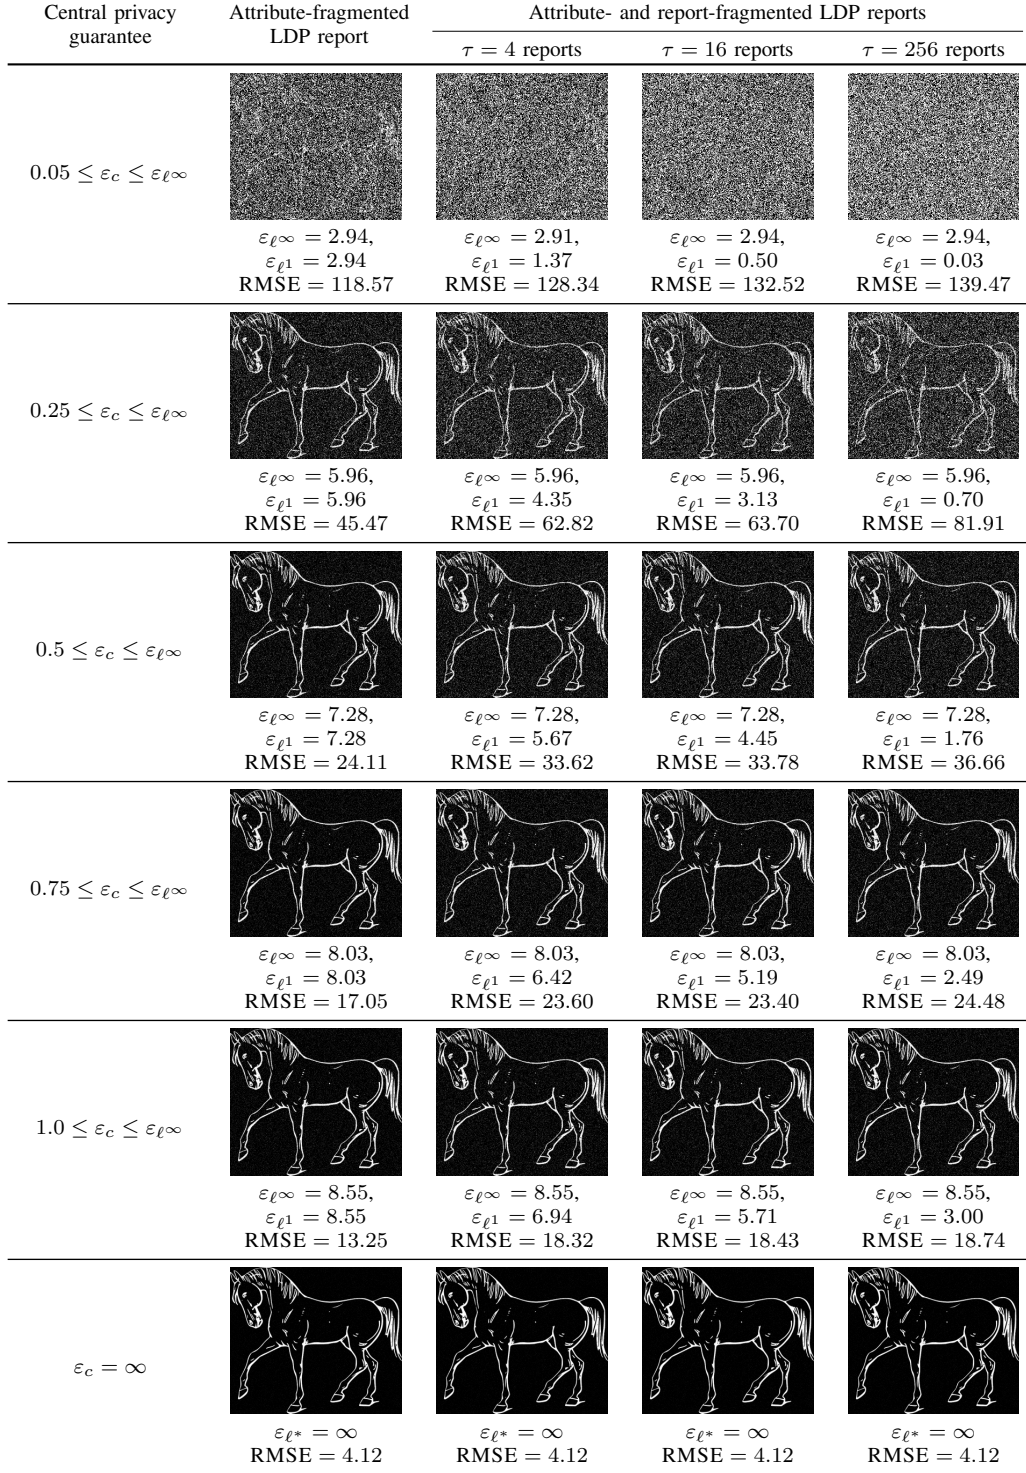<br>$\varepsilon_{\ell\infty} = 2.94,$<br>$\varepsilon_{\ell 1} = 2.94$<br>RMSE = 118.57  | 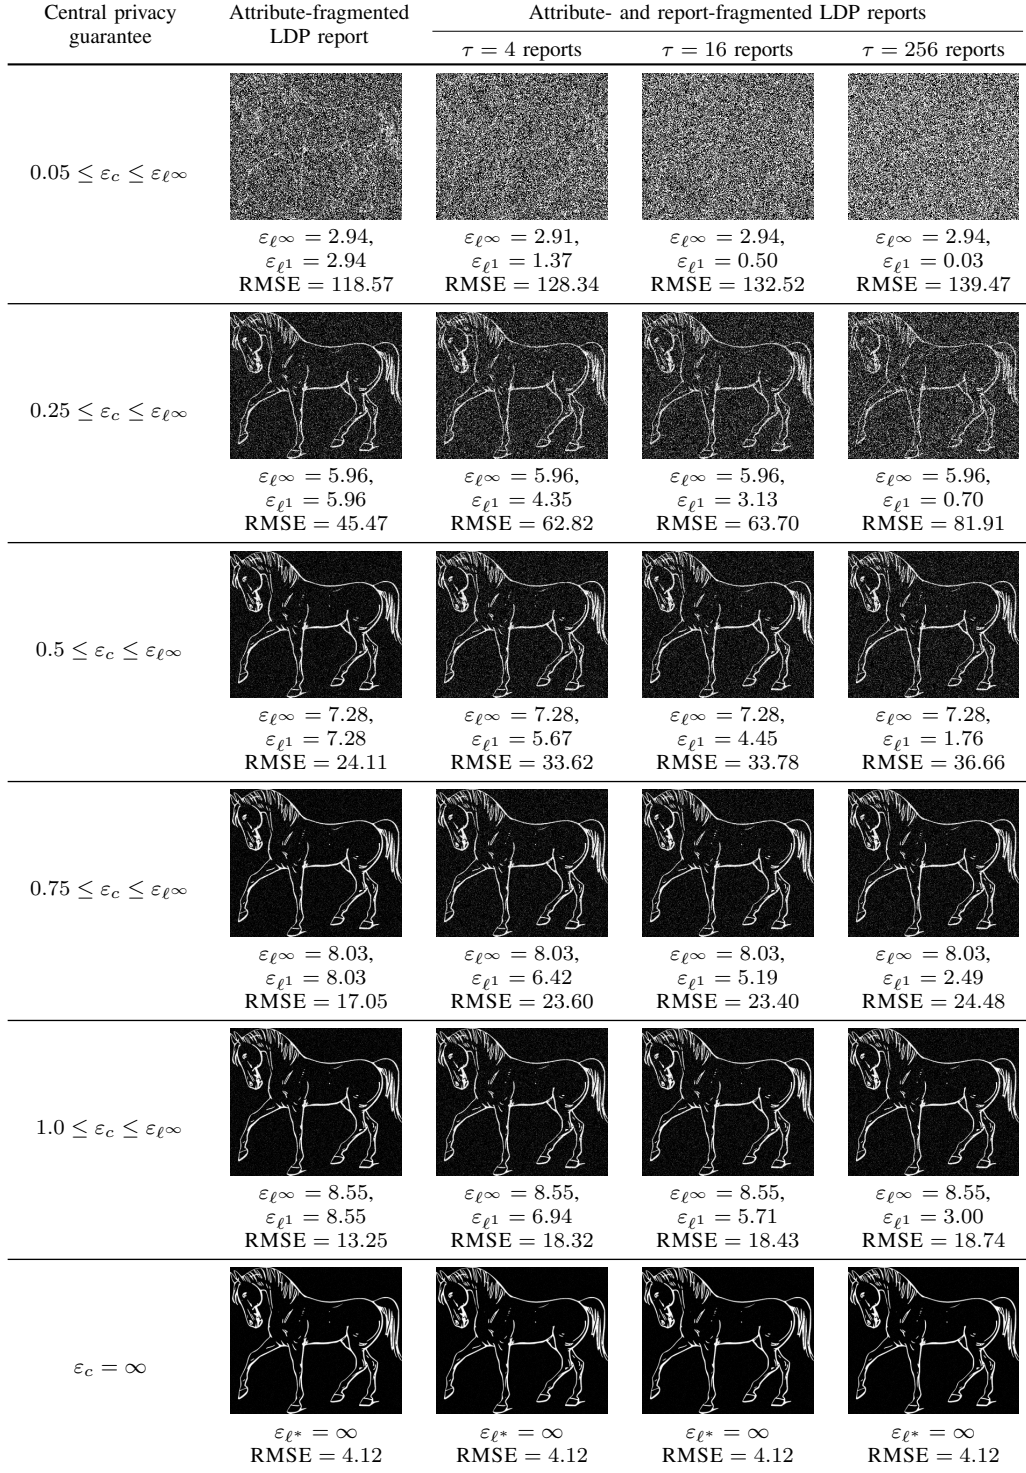<br>$\varepsilon_{\ell\infty} = 2.91,$<br>$\varepsilon_{\ell 1} = 1.37$<br>RMSE = 128.34  | 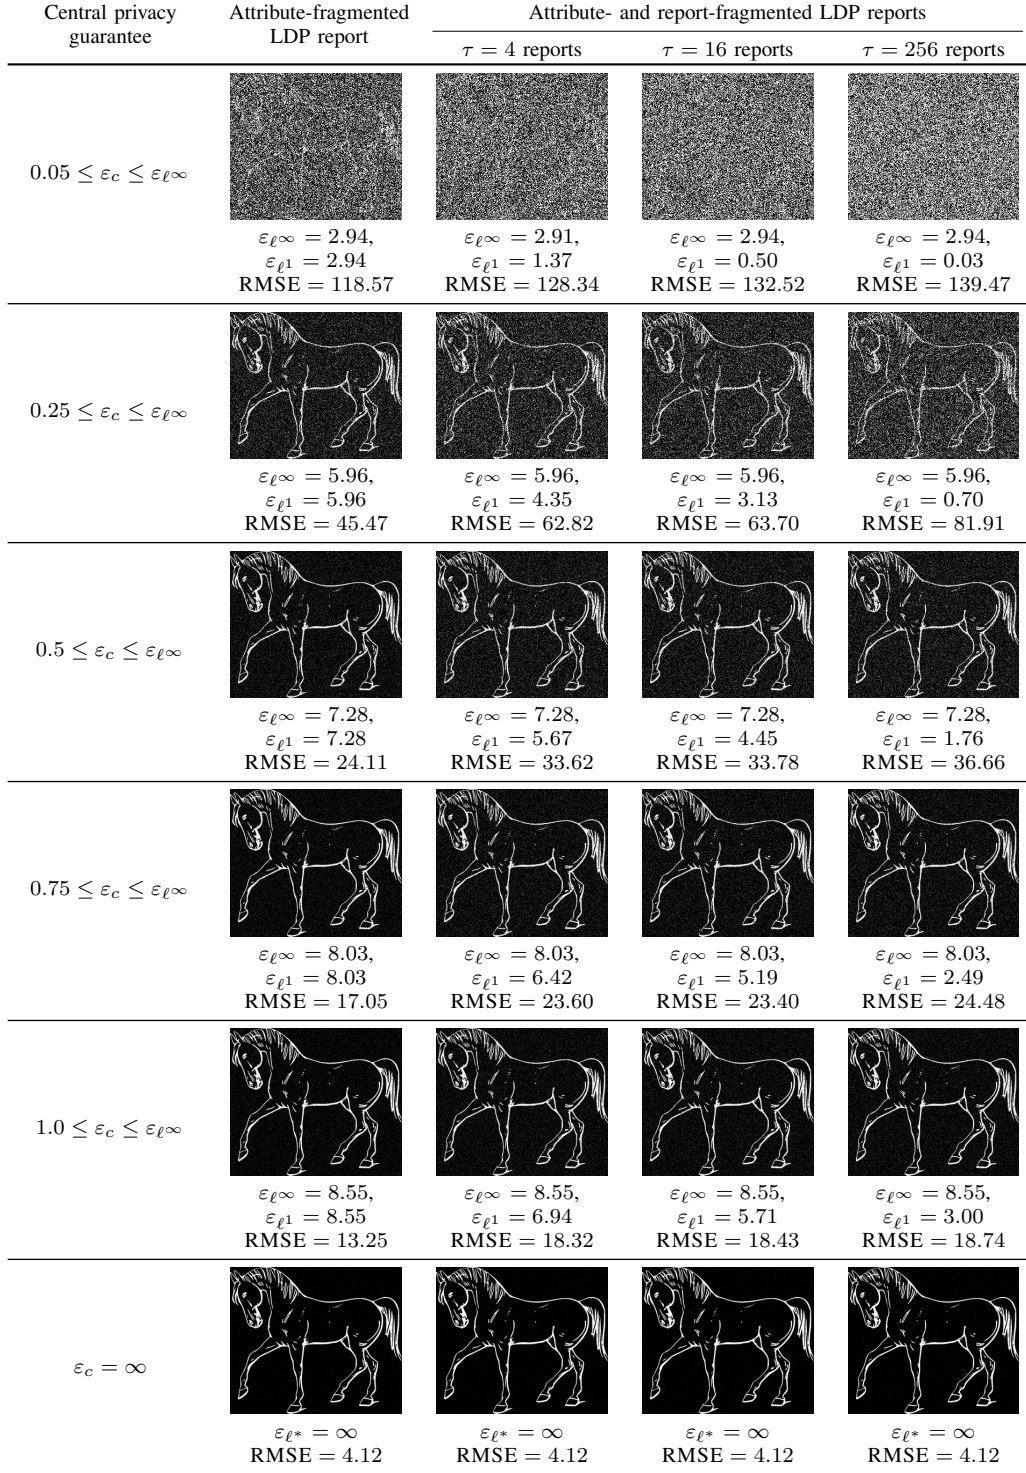<br>$\varepsilon_{\ell\infty} = 2.94,$<br>$\varepsilon_{\ell 1} = 0.50$<br>RMSE = 132.52  | 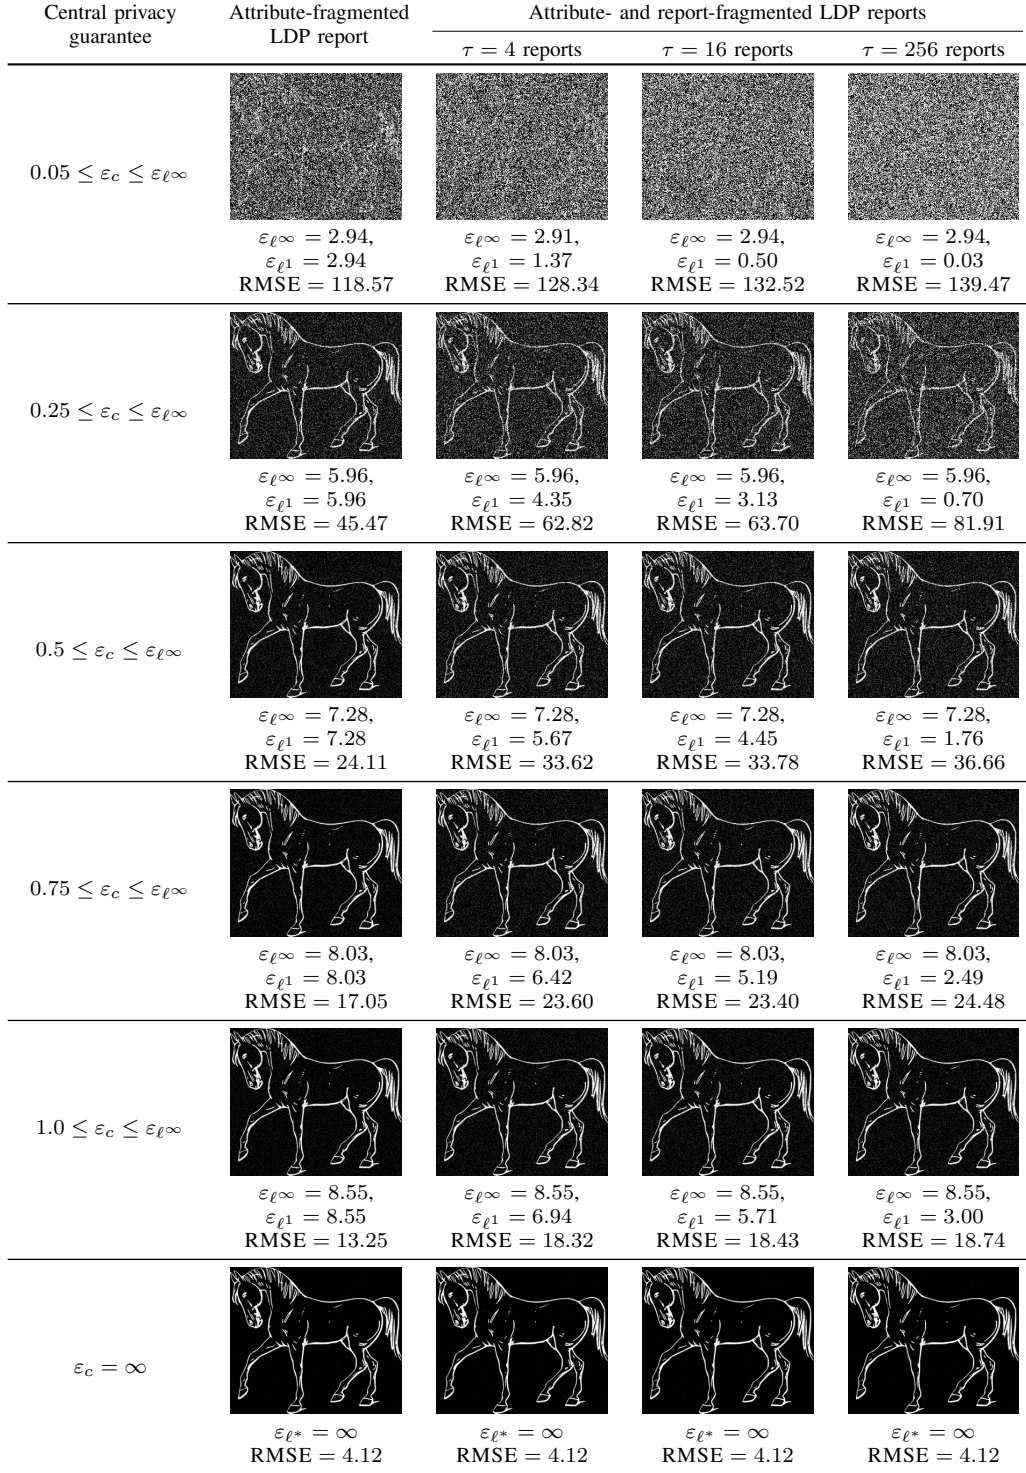<br>$\varepsilon_{\ell\infty} = 2.94,$<br>$\varepsilon_{\ell 1} = 0.03$<br>RMSE = 139.47  |
| $0.25 \leq \varepsilon_c \leq \varepsilon_{\ell\infty}$ | 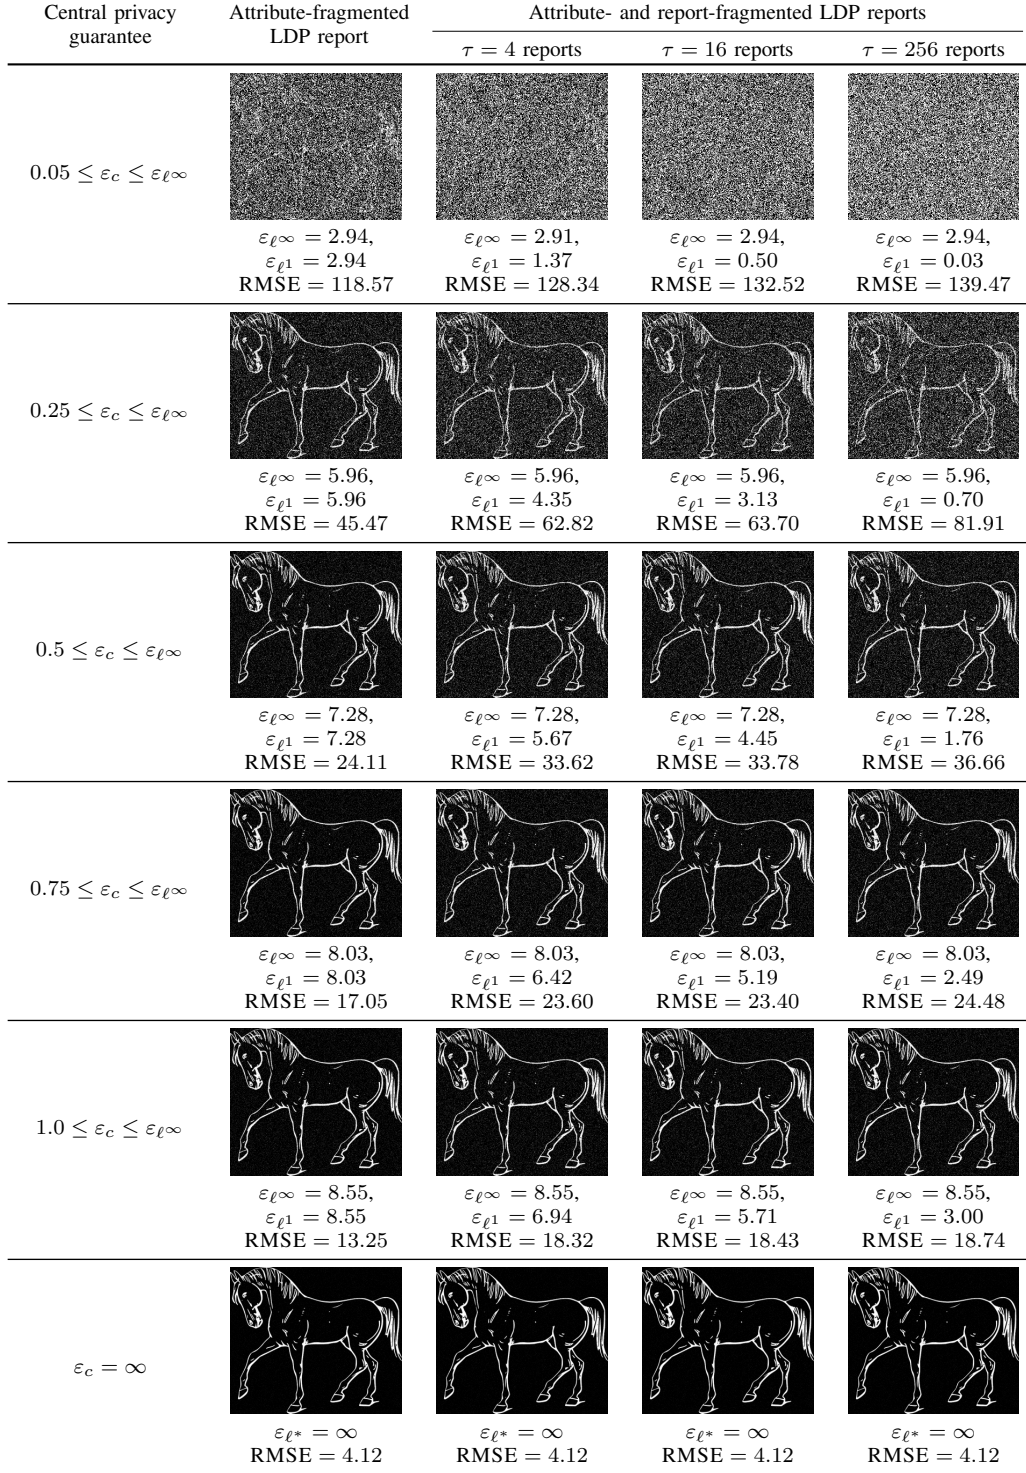<br>$\varepsilon_{\ell\infty} = 5.96,$<br>$\varepsilon_{\ell 1} = 5.96$<br>RMSE = 45.47   | 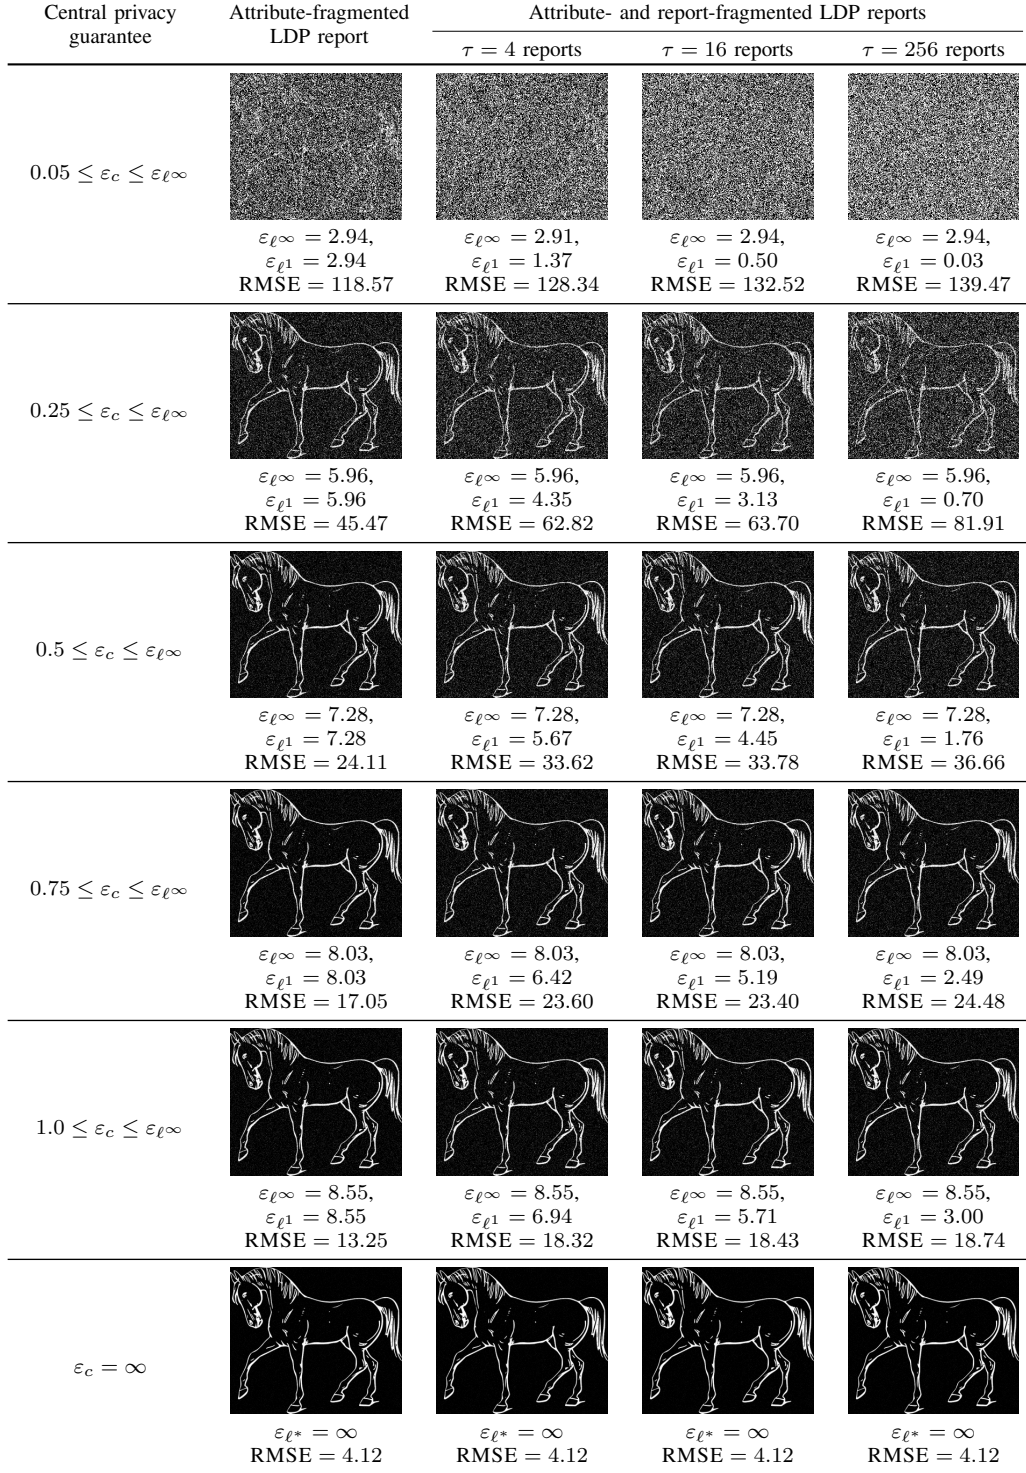<br>$\varepsilon_{\ell\infty} = 5.96,$<br>$\varepsilon_{\ell 1} = 4.35$<br>RMSE = 62.82   | 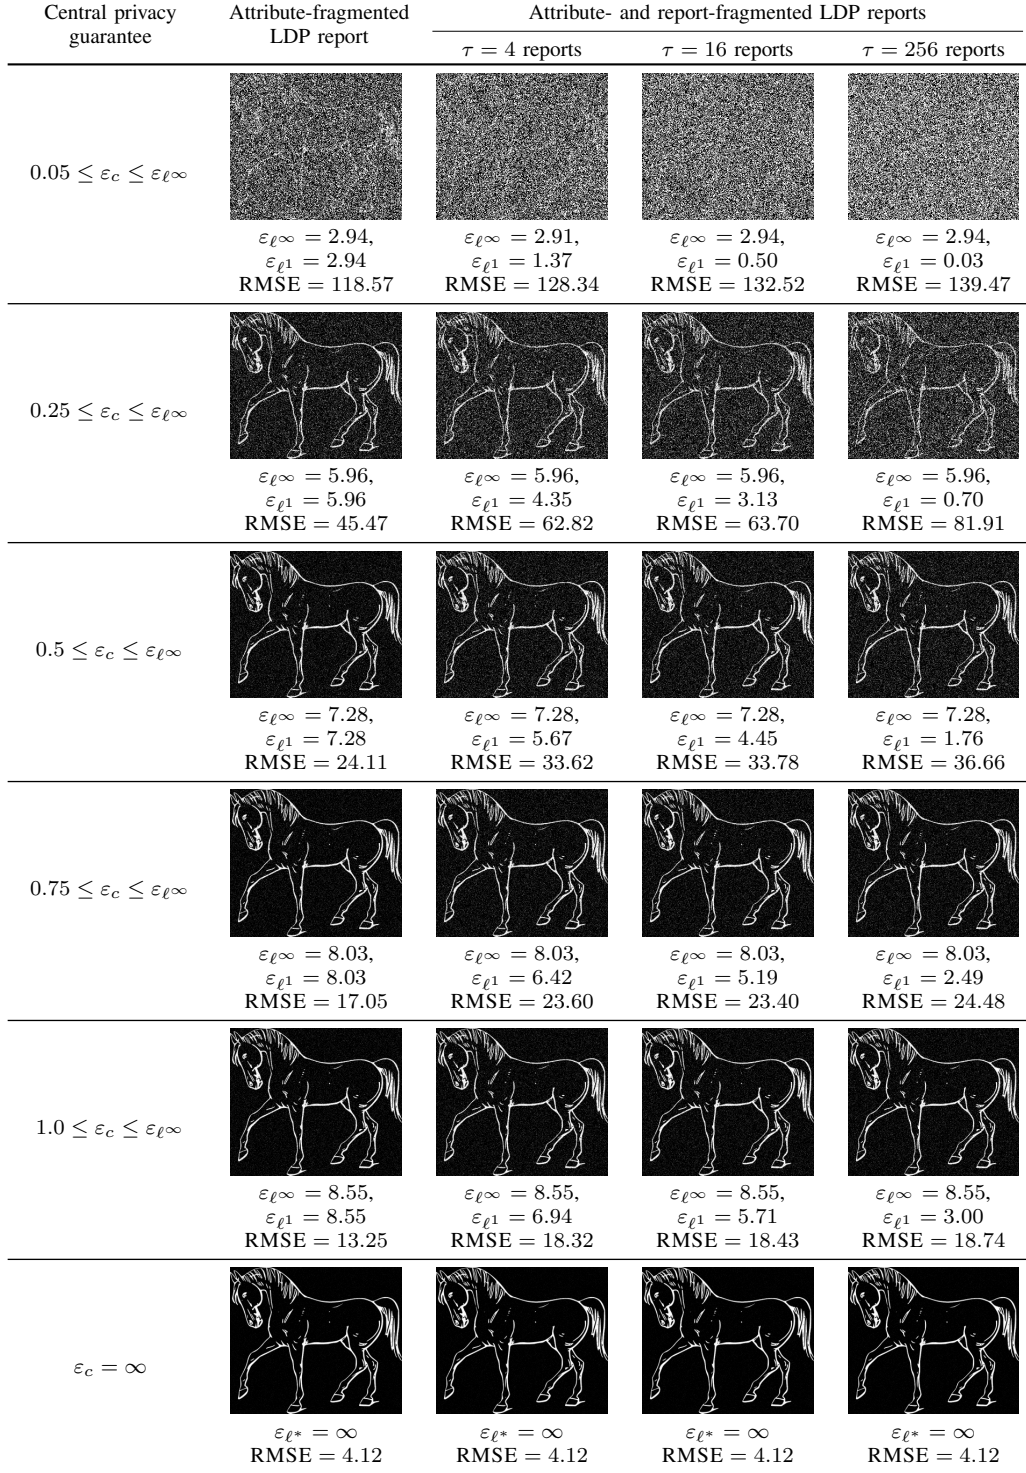<br>$\varepsilon_{\ell\infty} = 5.96,$<br>$\varepsilon_{\ell 1} = 3.13$<br>RMSE = 63.70   | 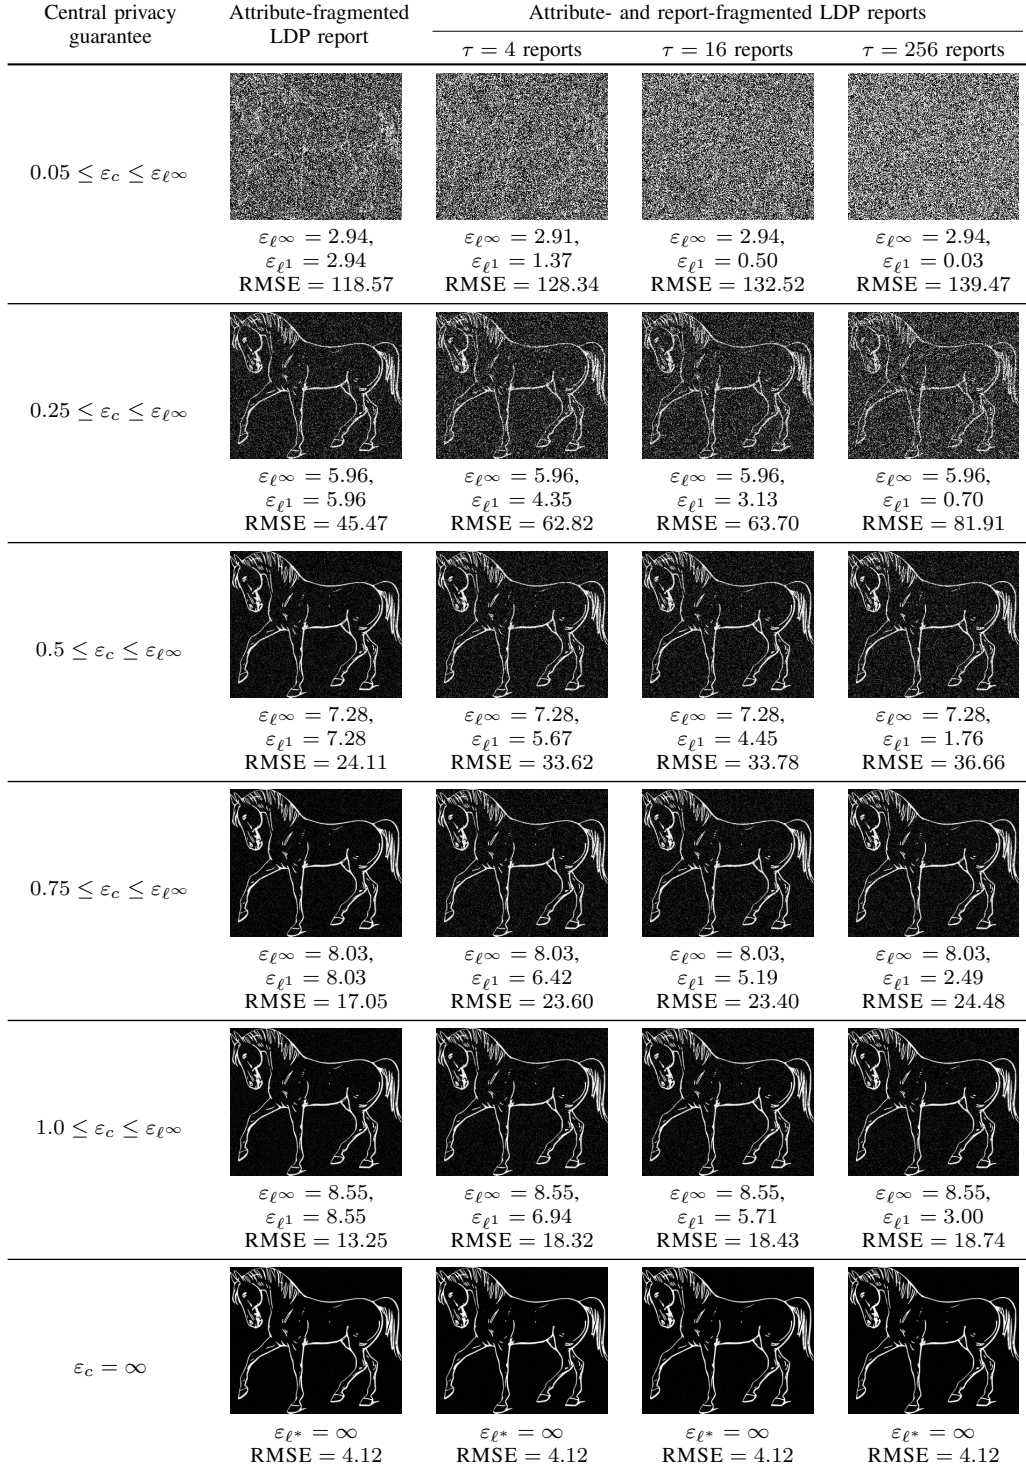<br>$\varepsilon_{\ell\infty} = 5.96,$<br>$\varepsilon_{\ell 1} = 0.70$<br>RMSE = 81.91   |
| $0.5 \leq \varepsilon_c \leq \varepsilon_{\ell\infty}$  | 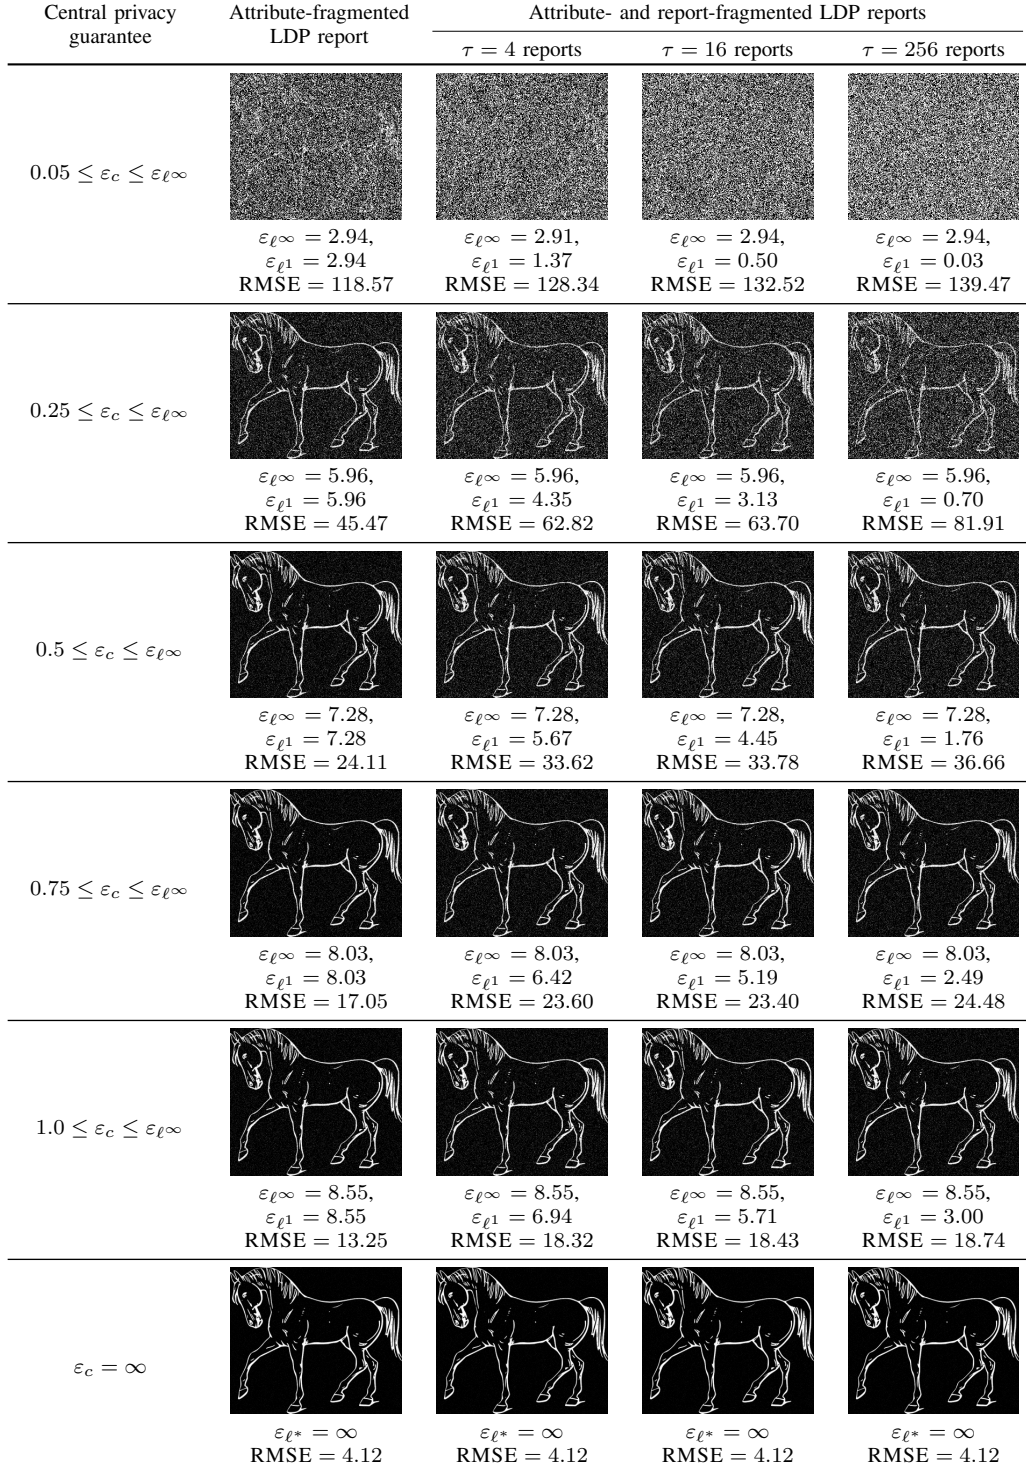<br>$\varepsilon_{\ell\infty} = 7.28,$<br>$\varepsilon_{\ell 1} = 7.28$<br>RMSE = 24.11  | 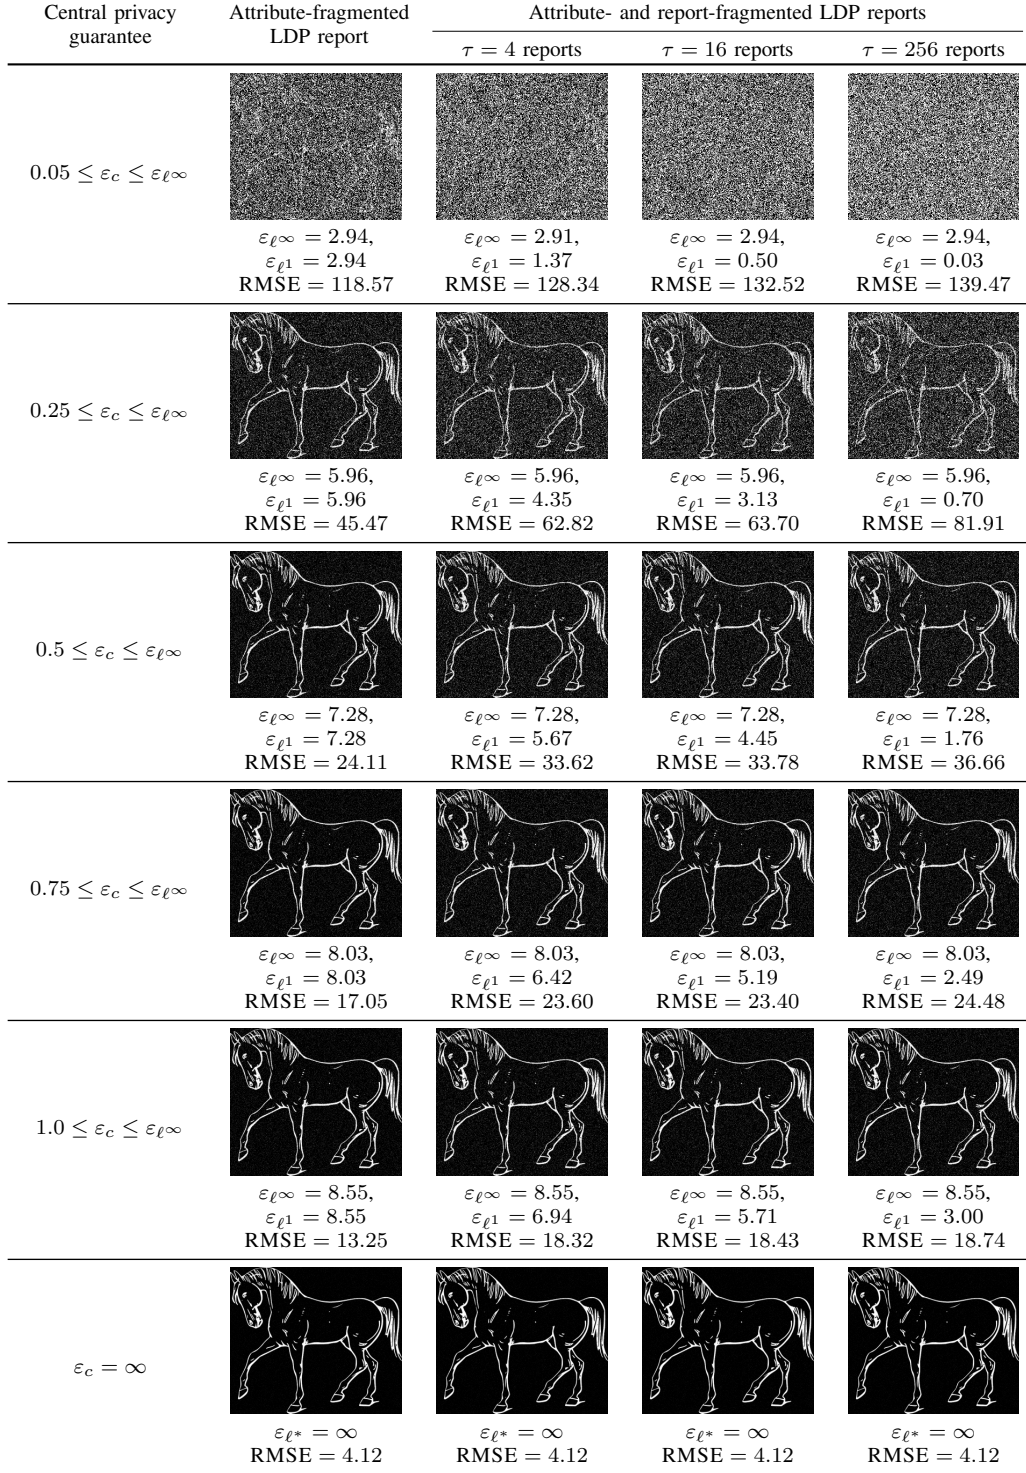<br>$\varepsilon_{\ell\infty} = 7.28,$<br>$\varepsilon_{\ell 1} = 5.67$<br>RMSE = 33.62  | 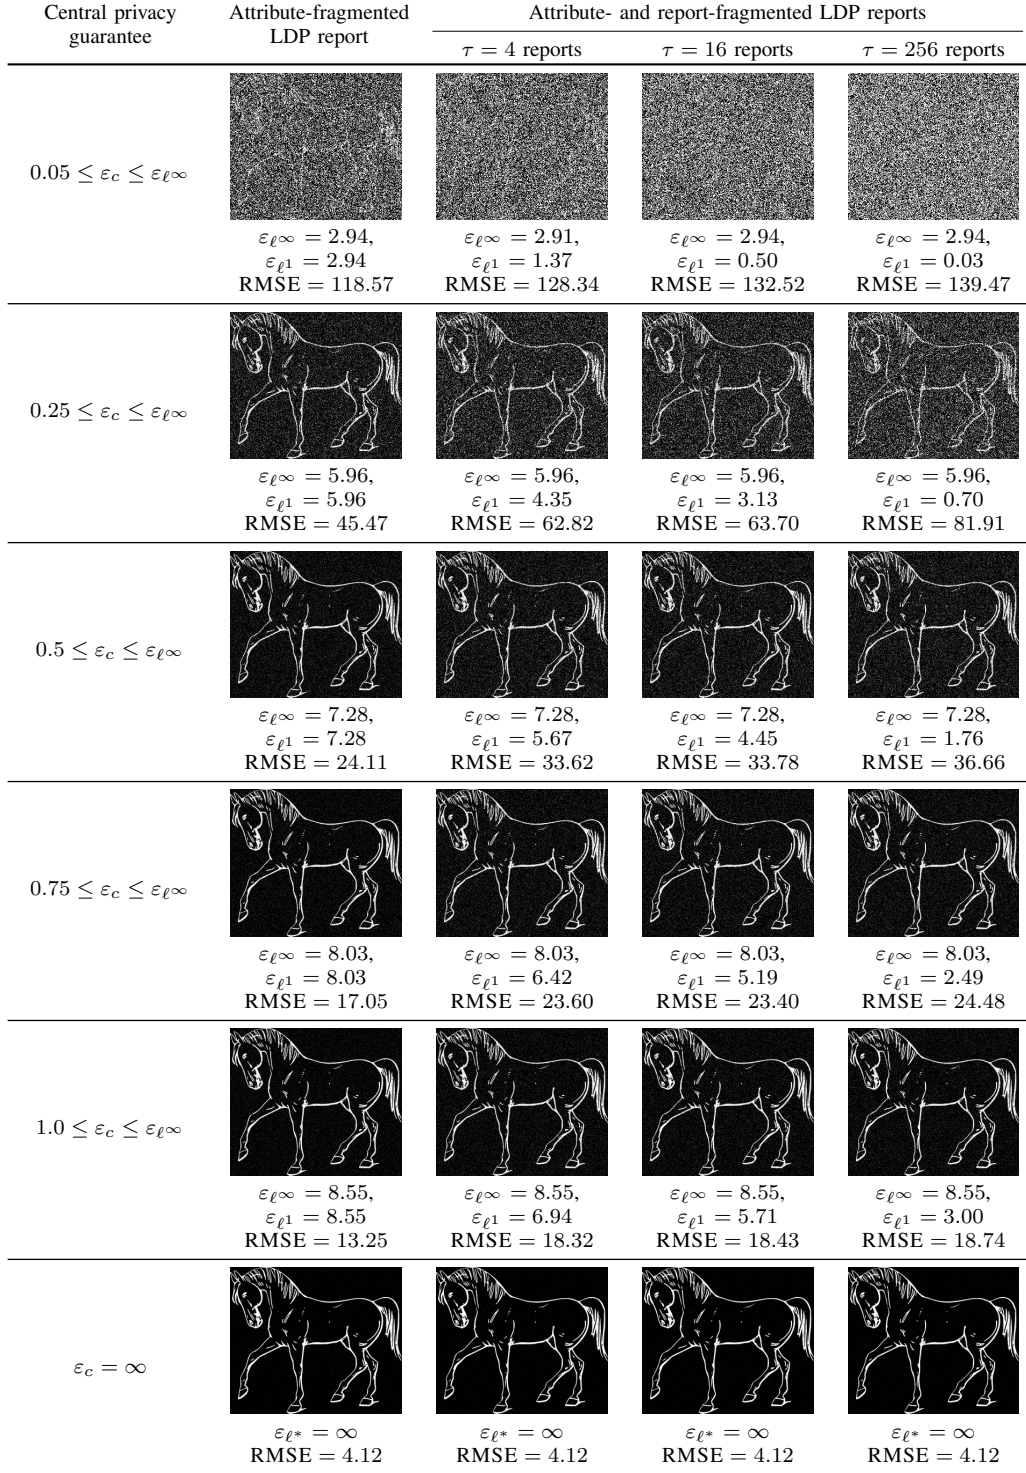<br>$\varepsilon_{\ell\infty} = 7.28,$<br>$\varepsilon_{\ell 1} = 4.45$<br>RMSE = 33.78  | 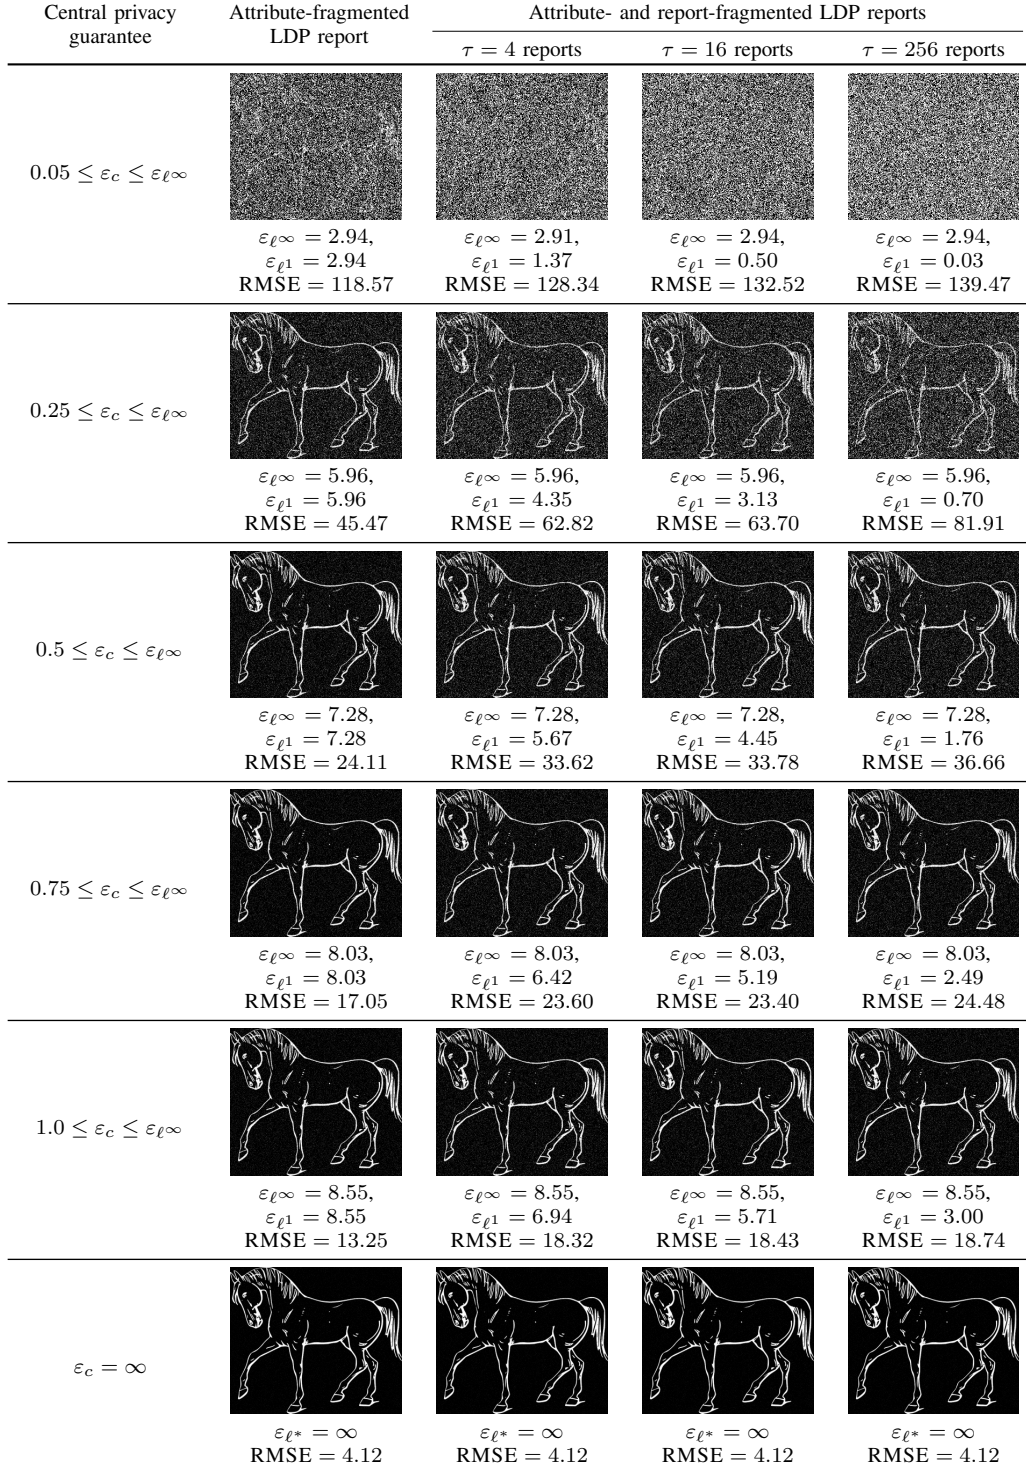<br>$\varepsilon_{\ell\infty} = 7.28,$<br>$\varepsilon_{\ell 1} = 1.76$<br>RMSE = 36.66  |
| $0.75 \leq \varepsilon_c \leq \varepsilon_{\ell\infty}$ | 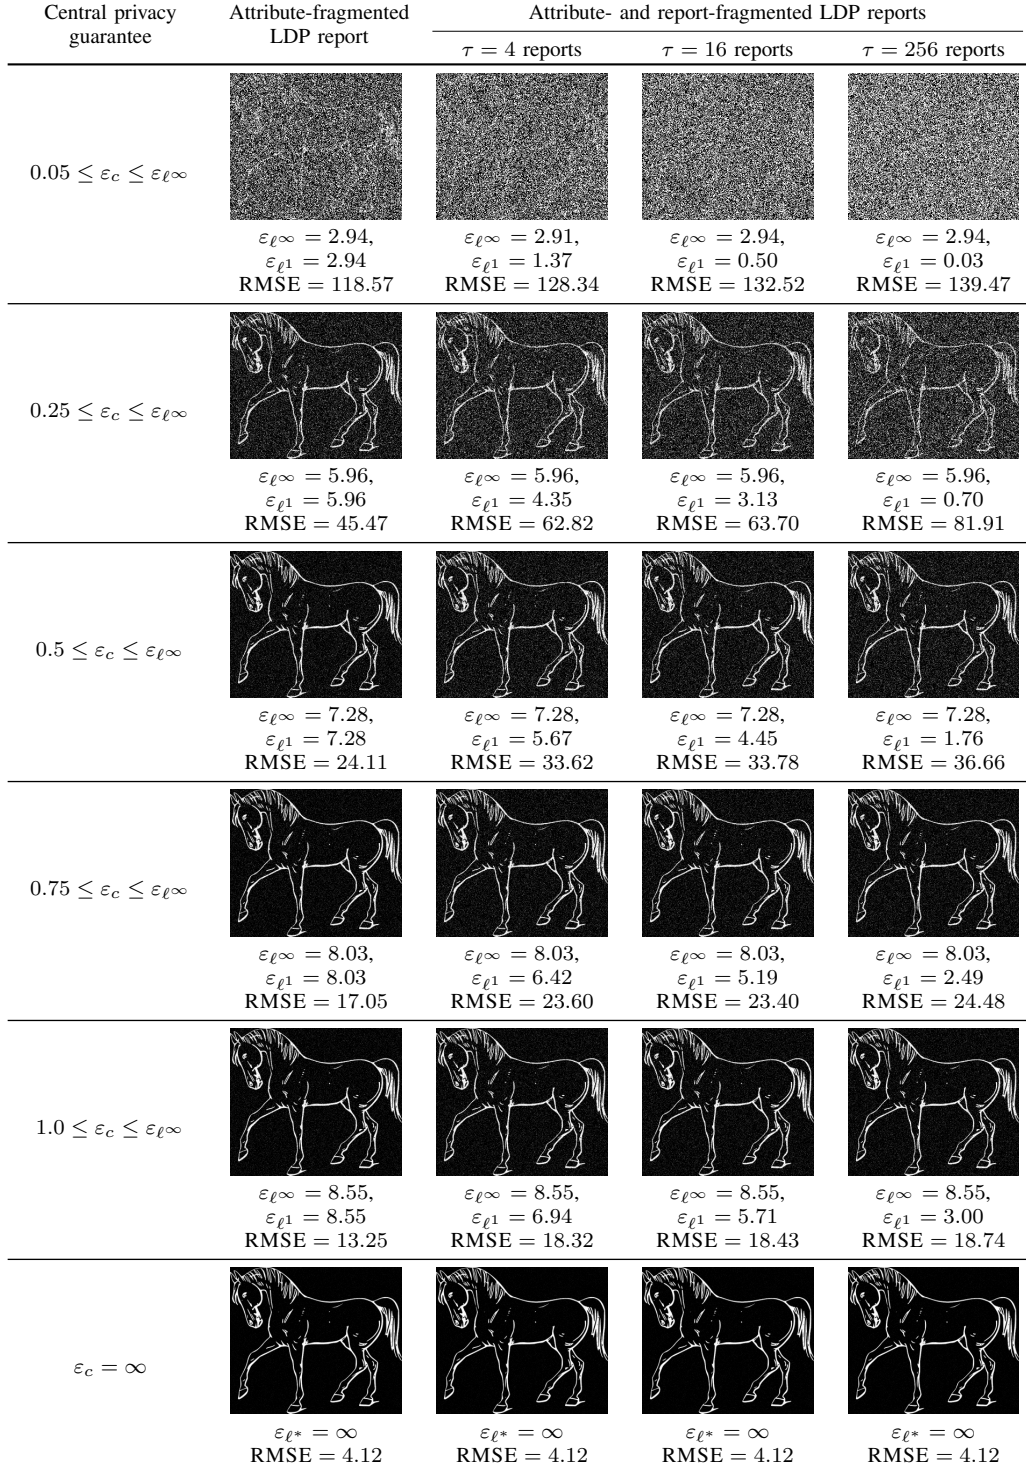<br>$\varepsilon_{\ell\infty} = 8.03,$<br>$\varepsilon_{\ell 1} = 8.03$<br>RMSE = 17.05 | 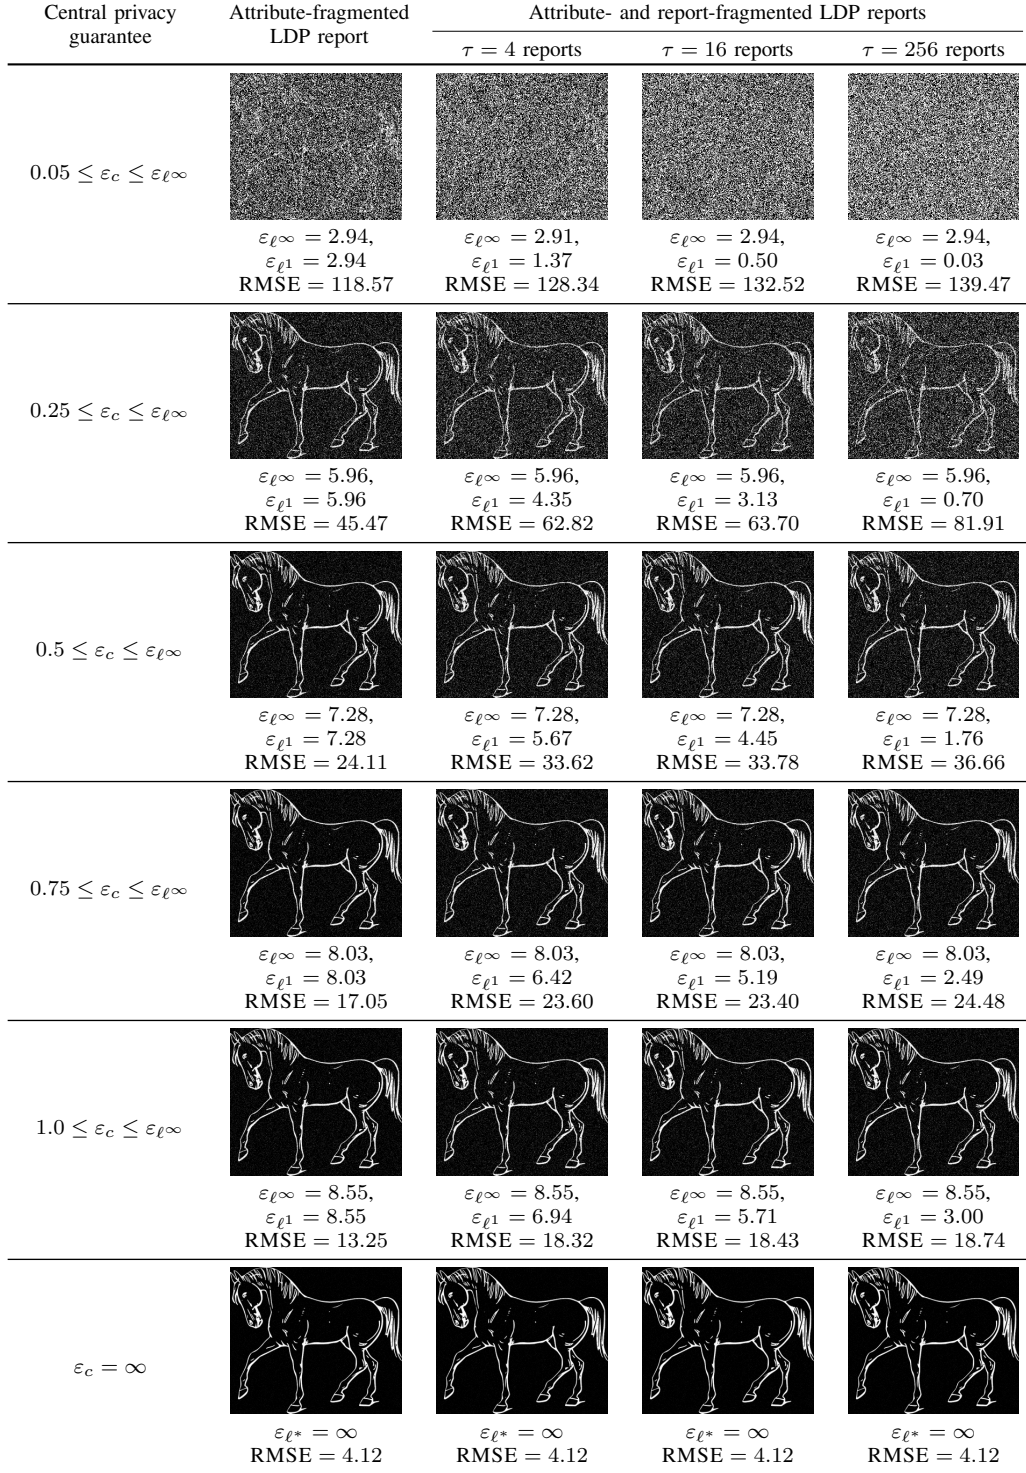<br>$\varepsilon_{\ell\infty} = 8.03,$<br>$\varepsilon_{\ell 1} = 6.42$<br>RMSE = 23.60 | 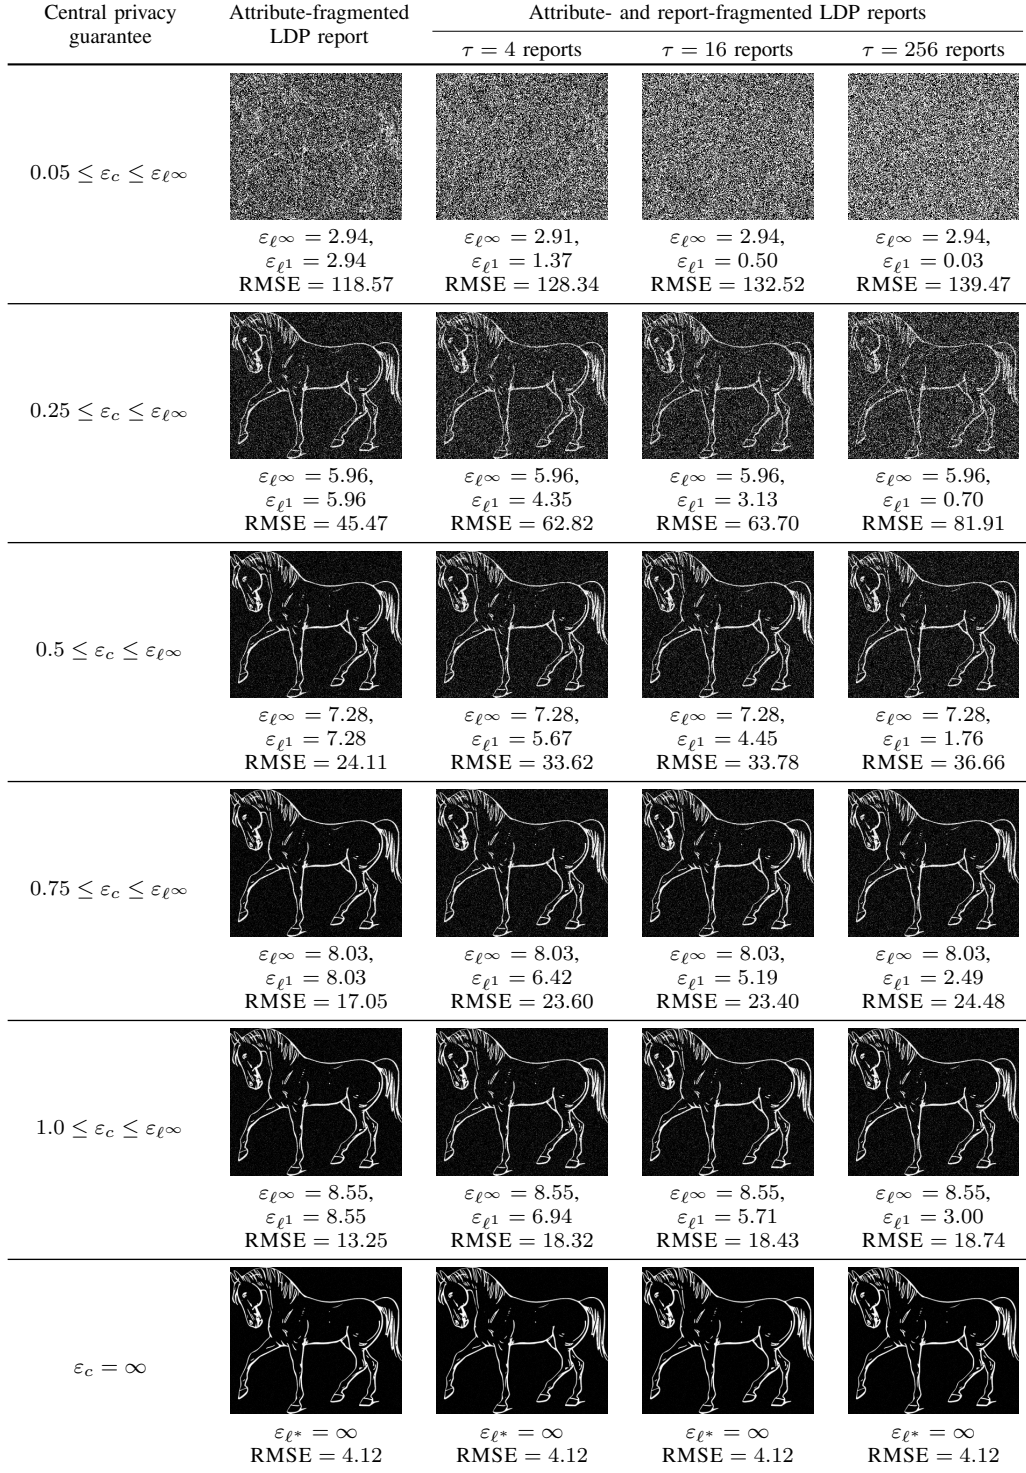<br>$\varepsilon_{\ell\infty} = 8.03,$<br>$\varepsilon_{\ell 1} = 5.19$<br>RMSE = 23.40 | 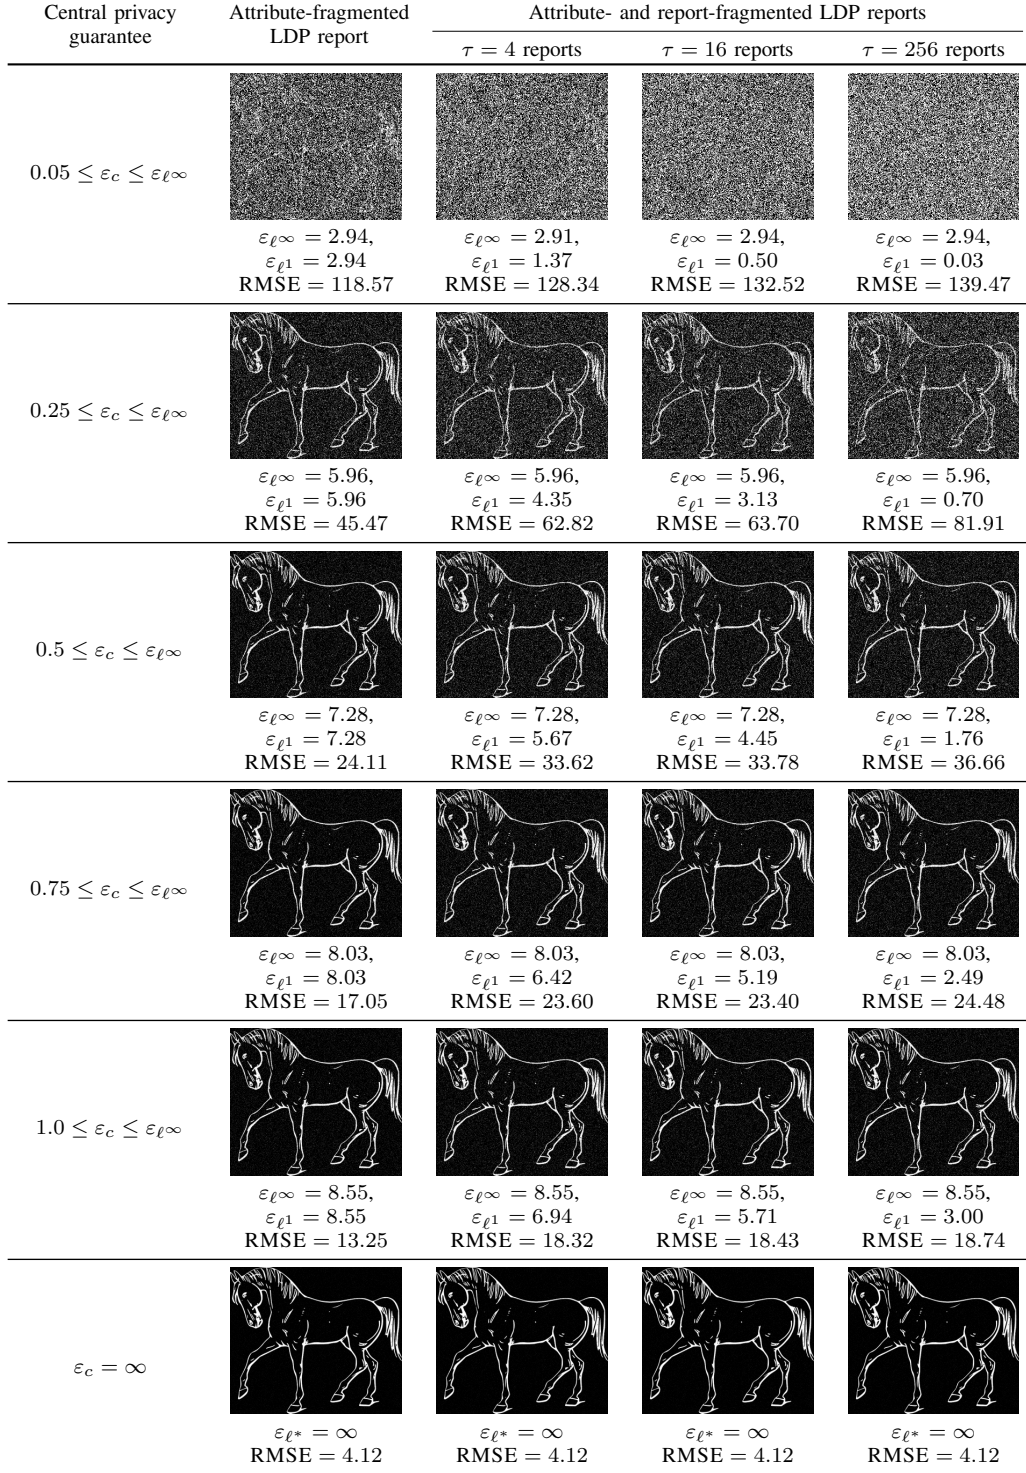<br>$\varepsilon_{\ell\infty} = 8.03,$<br>$\varepsilon_{\ell 1} = 2.49$<br>RMSE = 24.48 |
| $1.0 \leq \varepsilon_c \leq \varepsilon_{\ell\infty}$  | 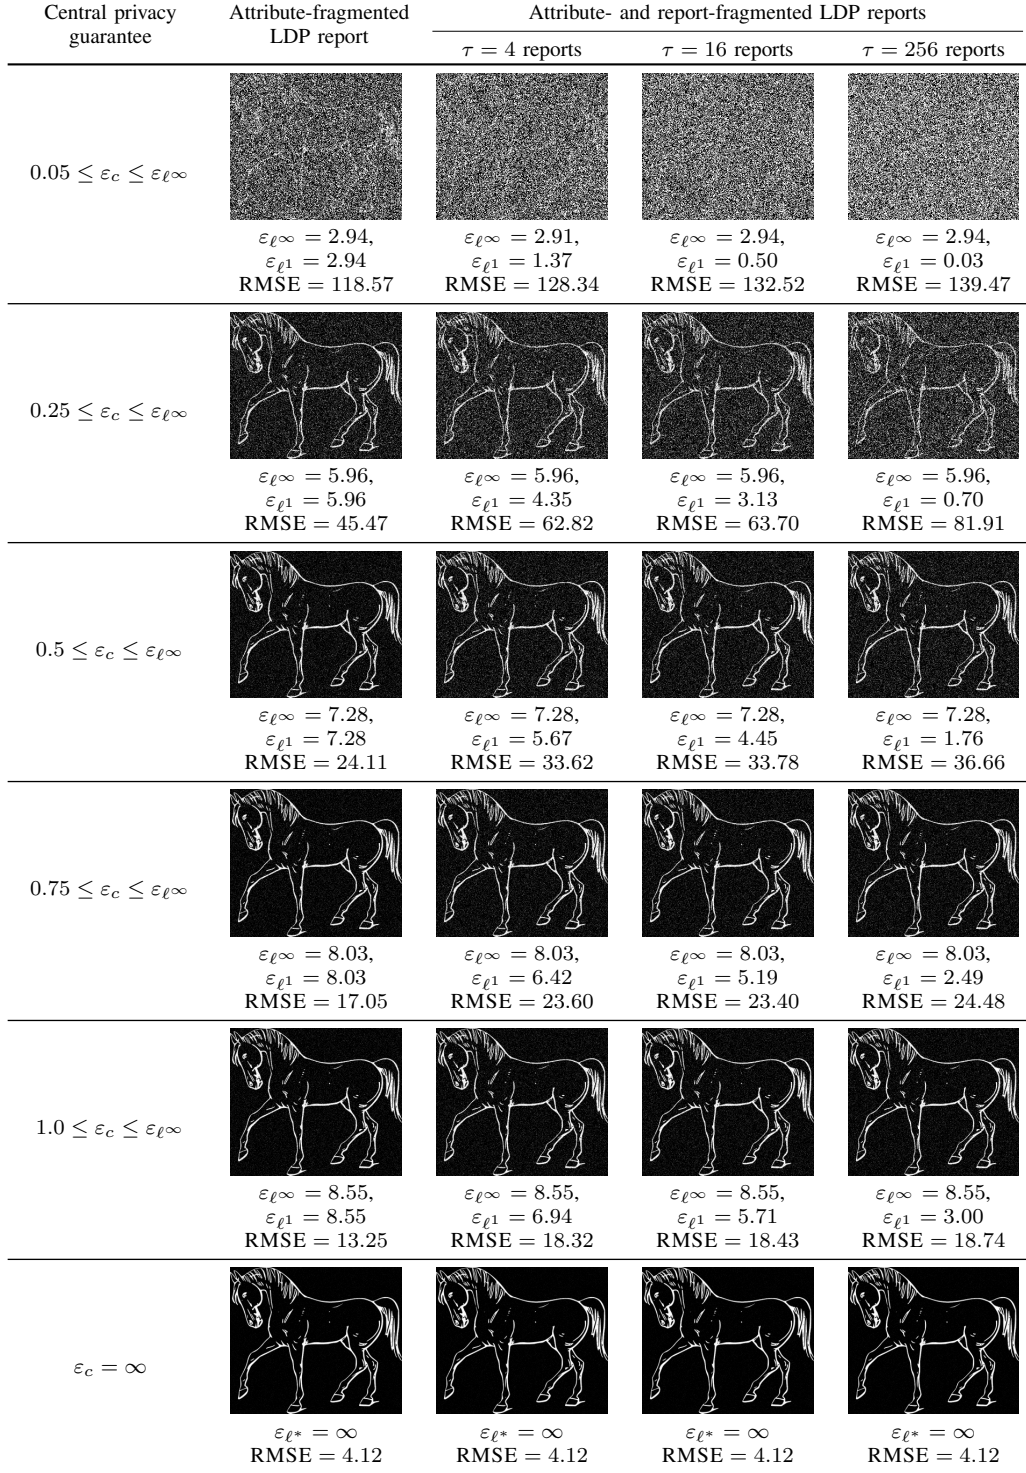<br>$\varepsilon_{\ell\infty} = 8.55,$<br>$\varepsilon_{\ell 1} = 8.55$<br>RMSE = 13.25 | 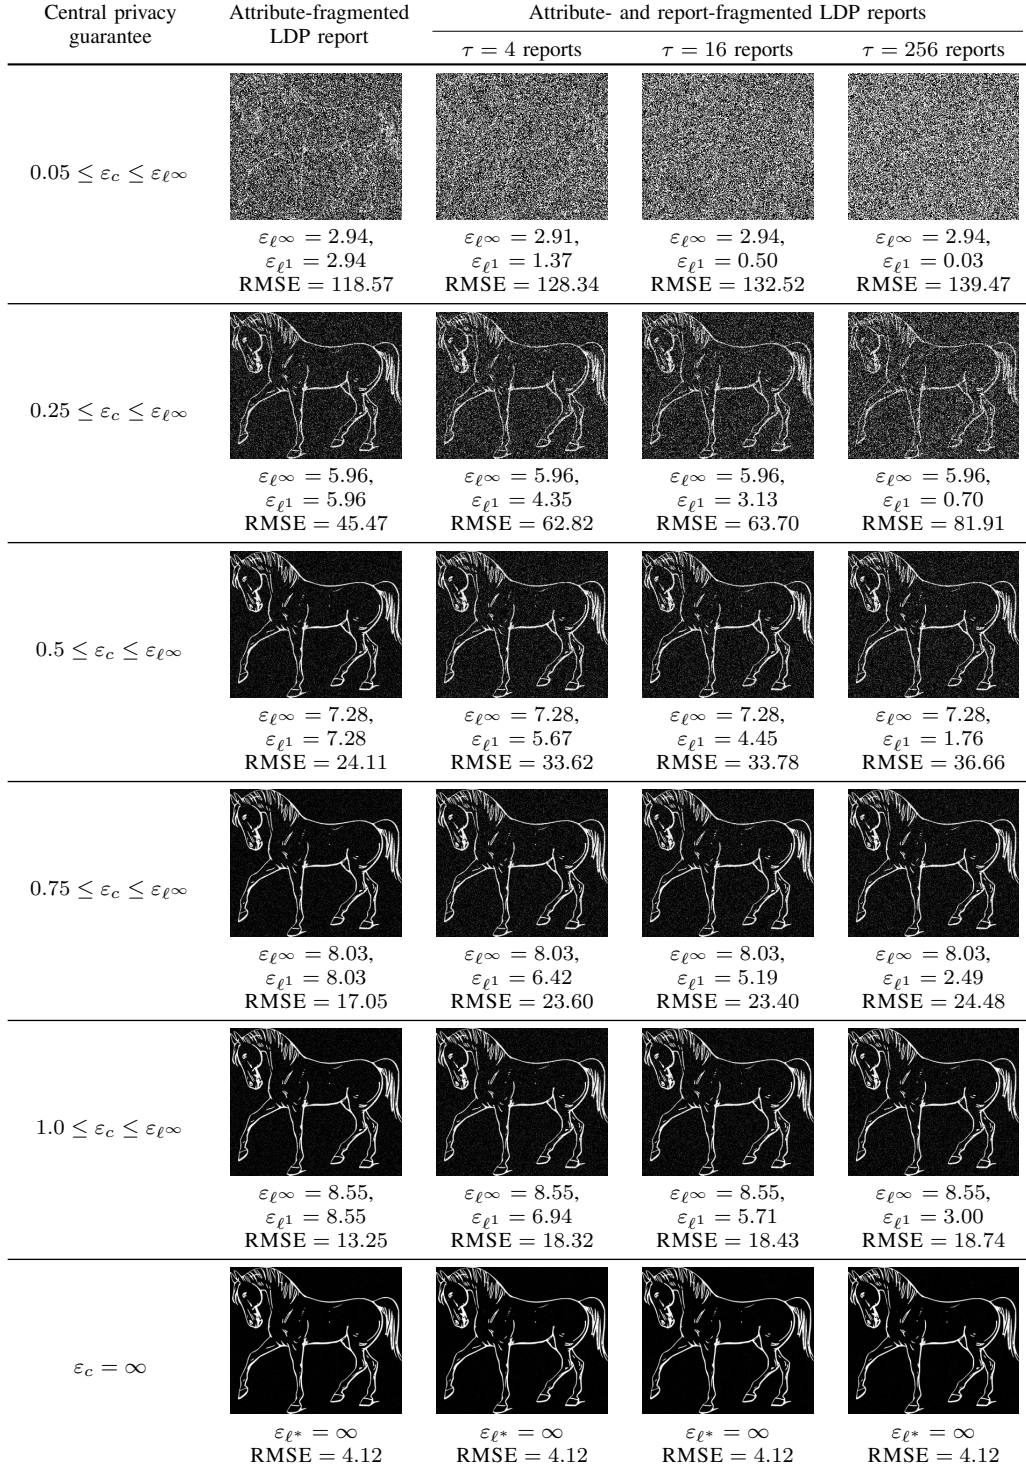<br>$\varepsilon_{\ell\infty} = 8.55,$<br>$\varepsilon_{\ell 1} = 6.94$<br>RMSE = 18.32 | 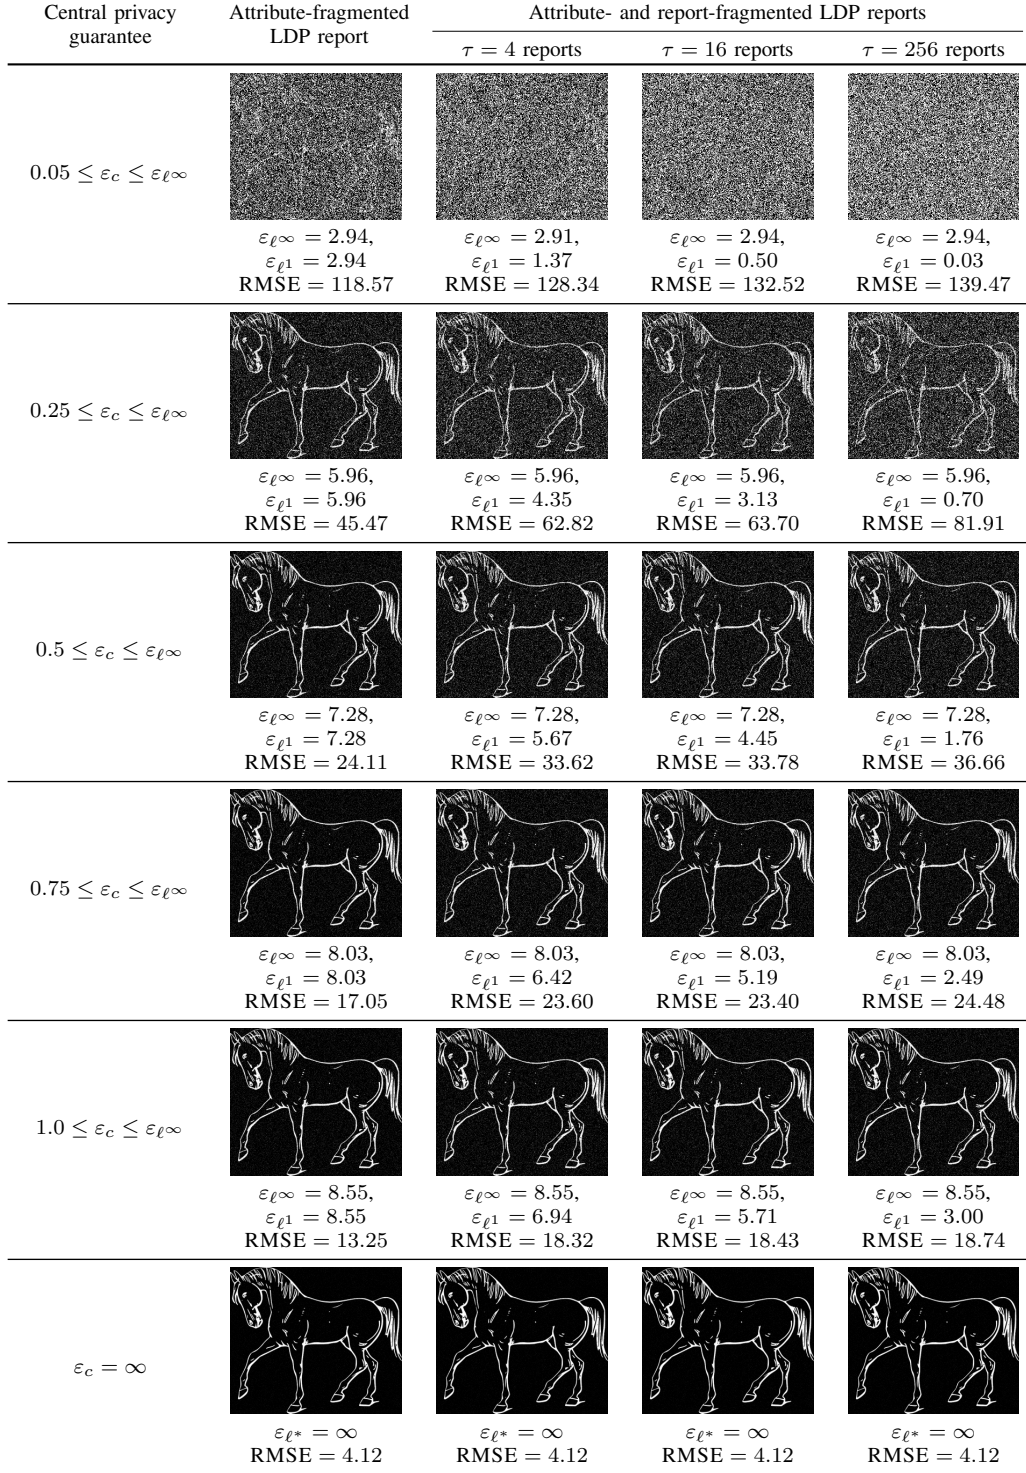<br>$\varepsilon_{\ell\infty} = 8.55,$<br>$\varepsilon_{\ell 1} = 5.71$<br>RMSE = 18.43 | 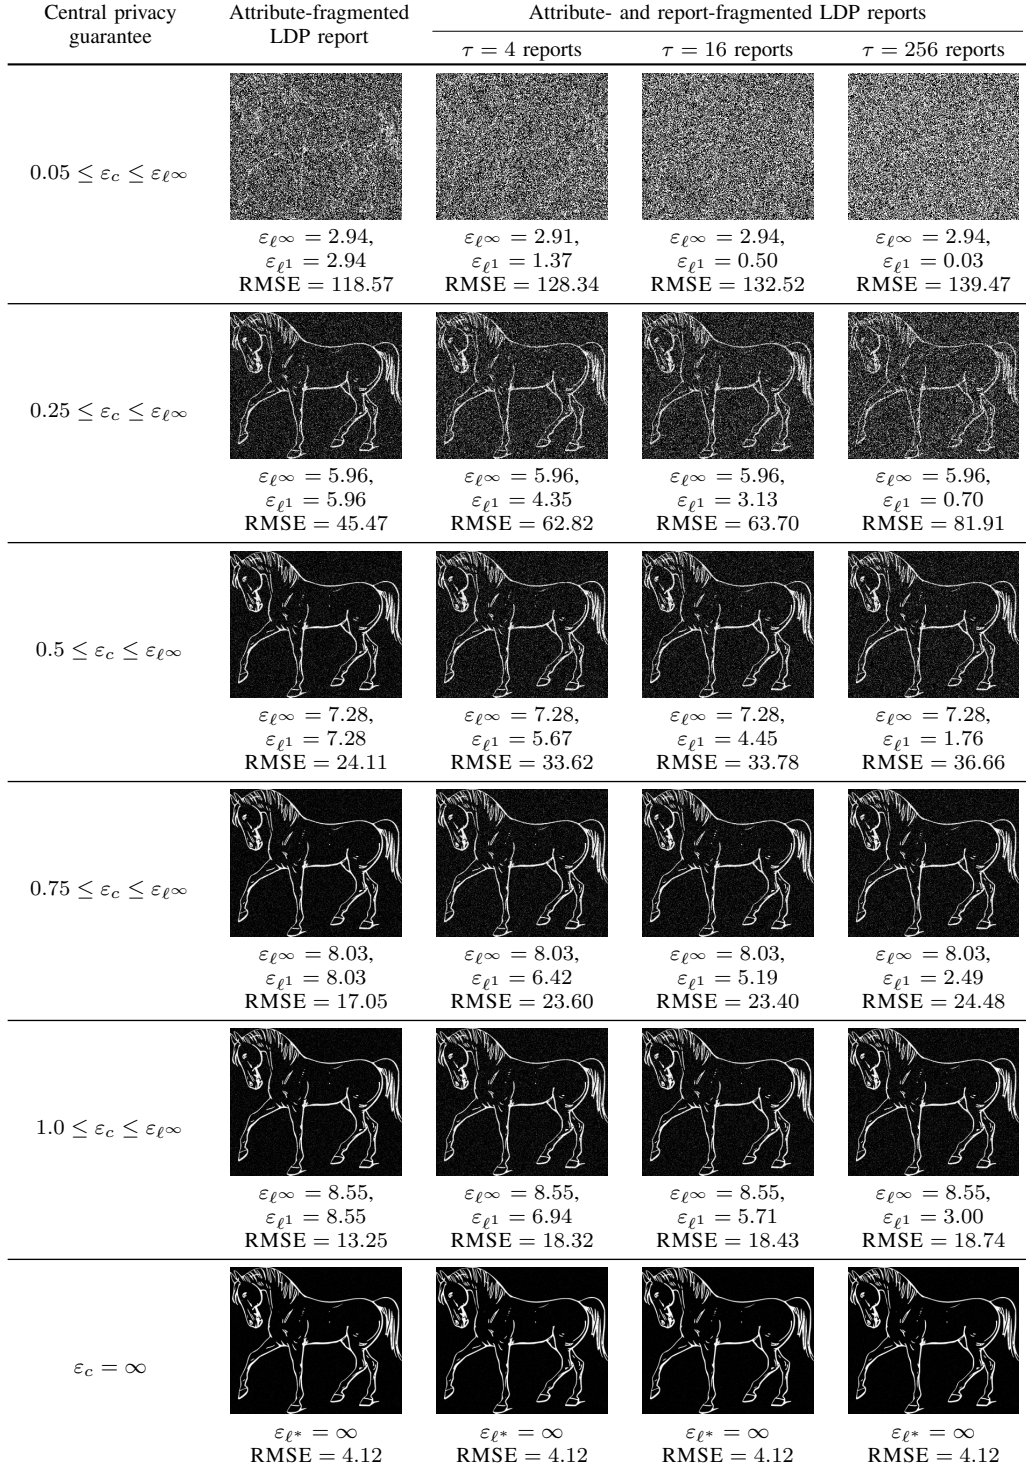<br>$\varepsilon_{\ell\infty} = 8.55,$<br>$\varepsilon_{\ell 1} = 3.00$<br>RMSE = 18.74 |
| $\varepsilon_c = \infty$                                | 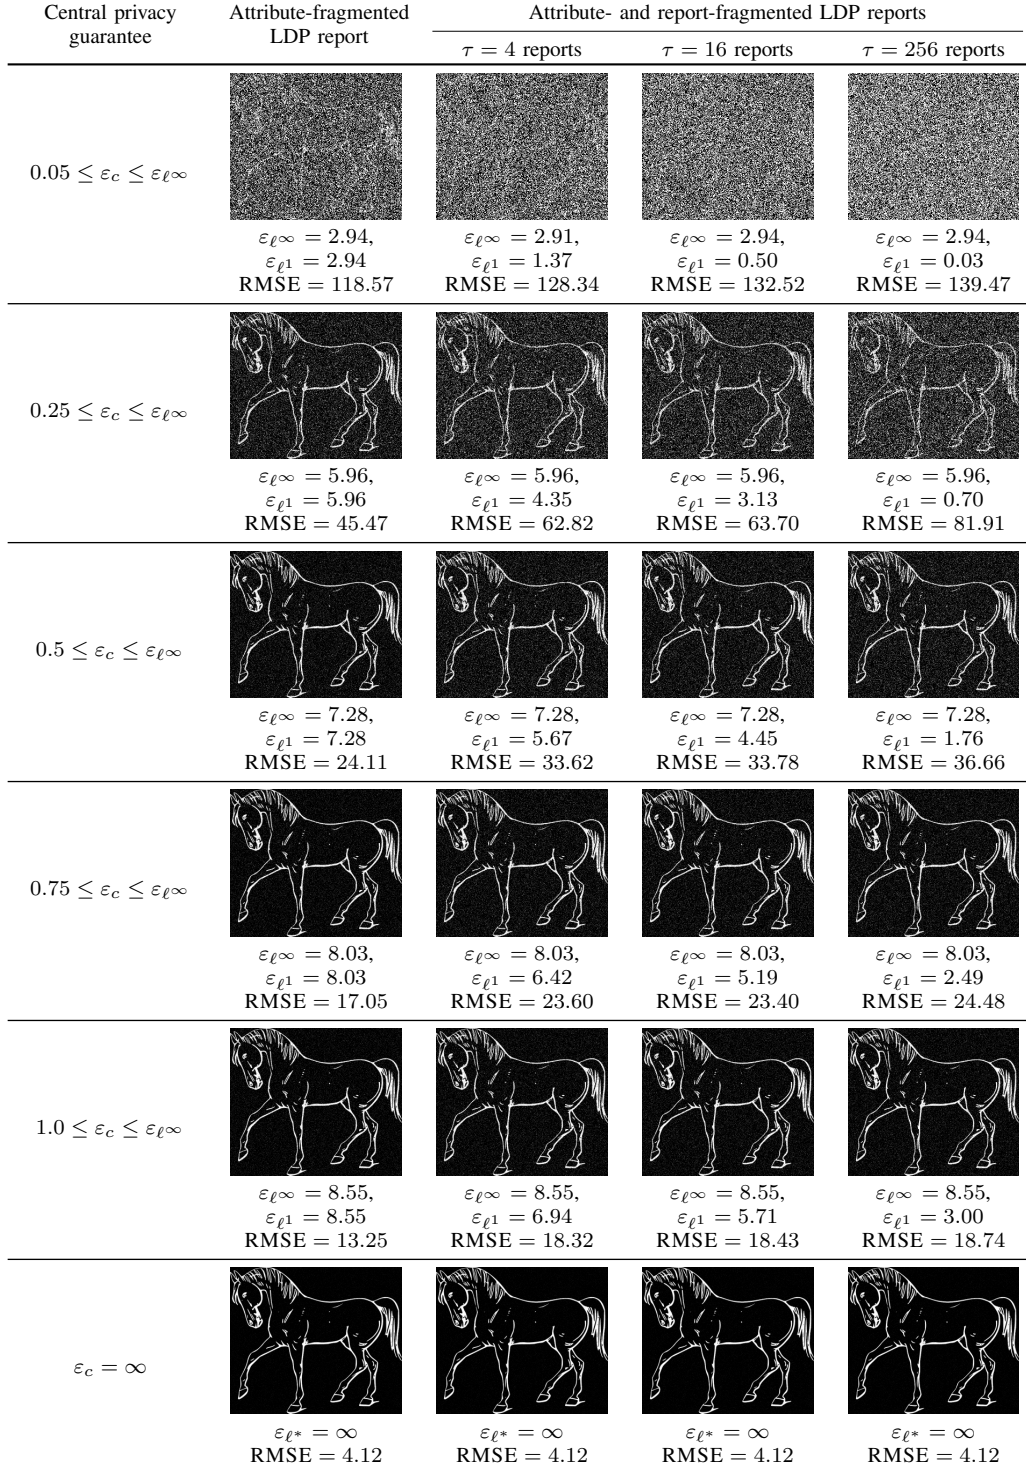<br>$\varepsilon_{\ell*} = \infty$<br>RMSE = 4.12                                       | 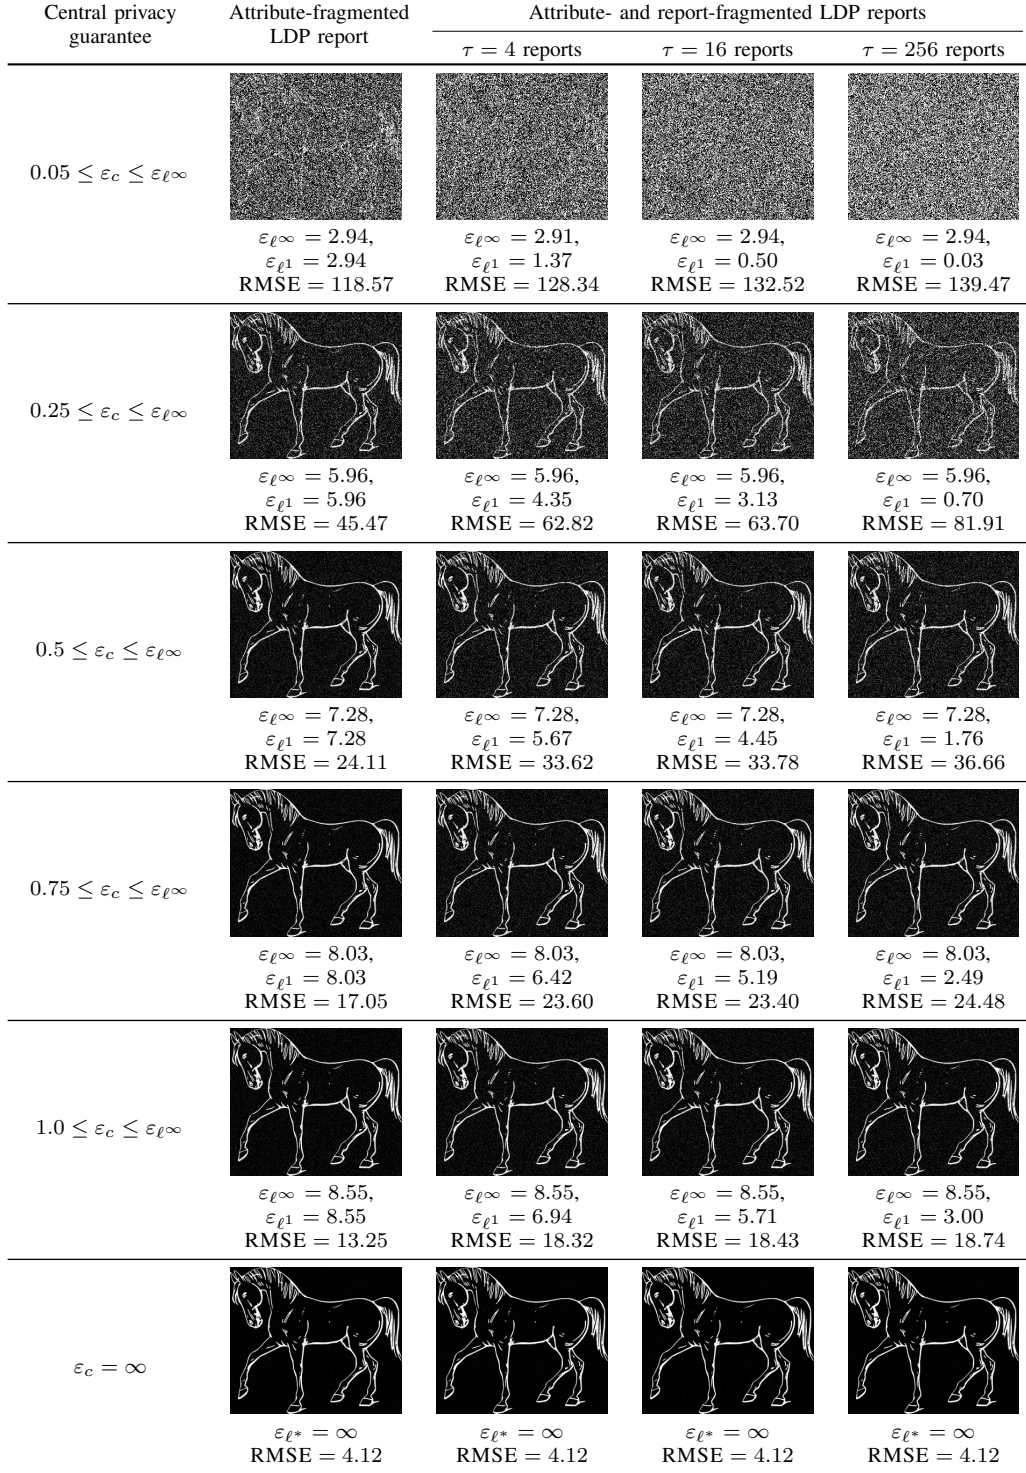<br>$\varepsilon_{\ell*} = \infty$<br>RMSE = 4.12                                       | 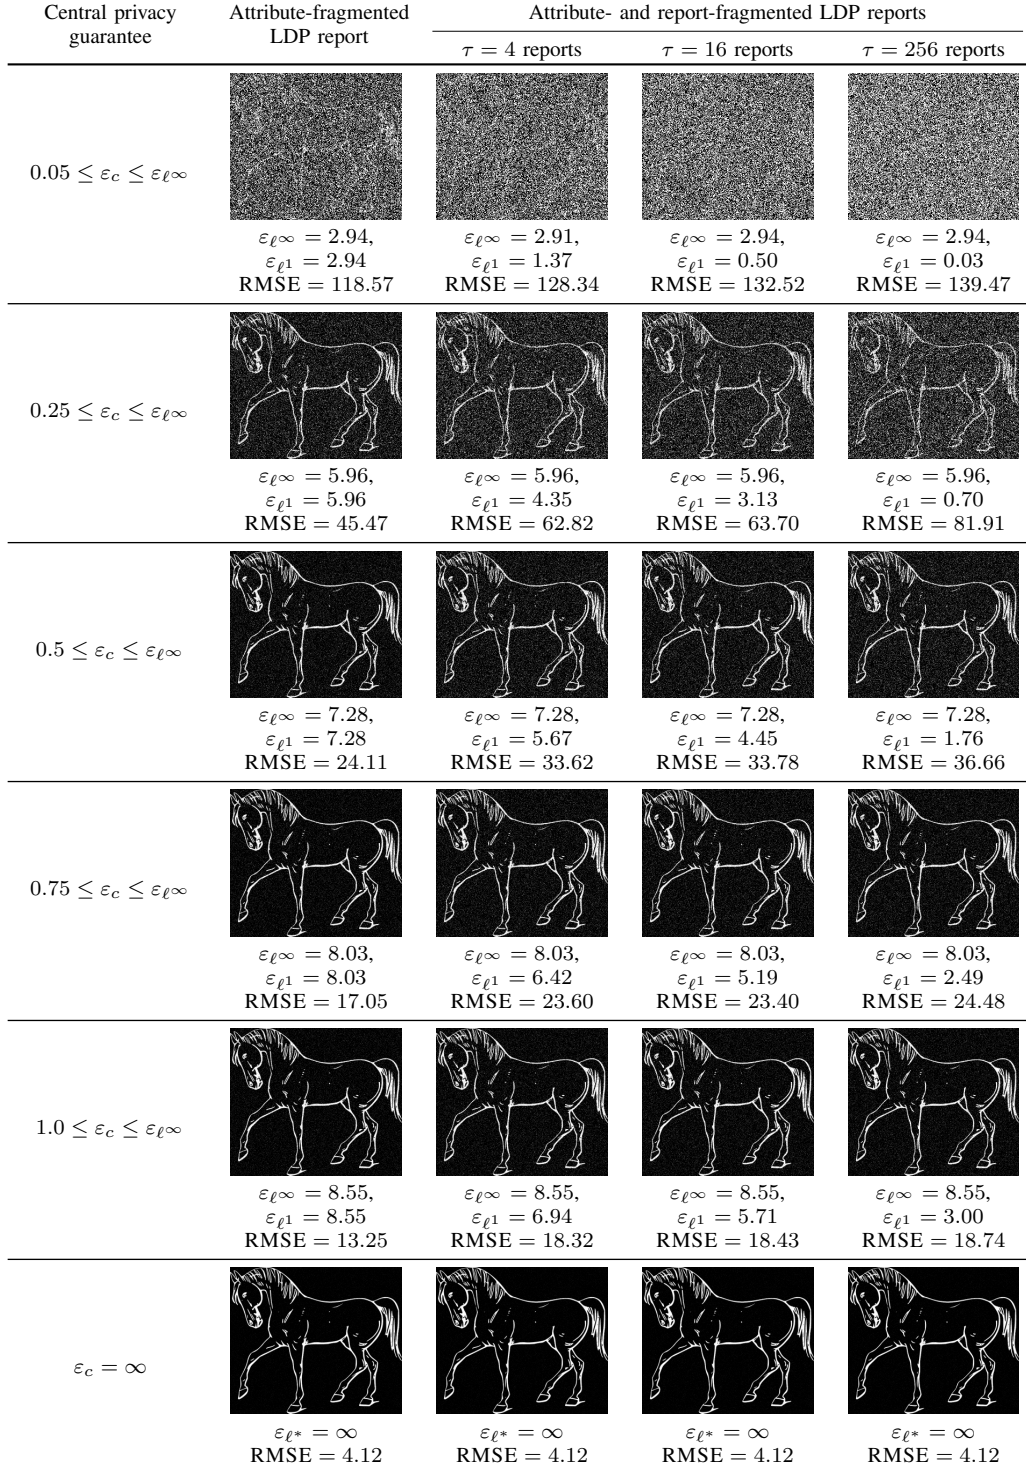<br>$\varepsilon_{\ell*} = \infty$<br>RMSE = 4.12                                       | 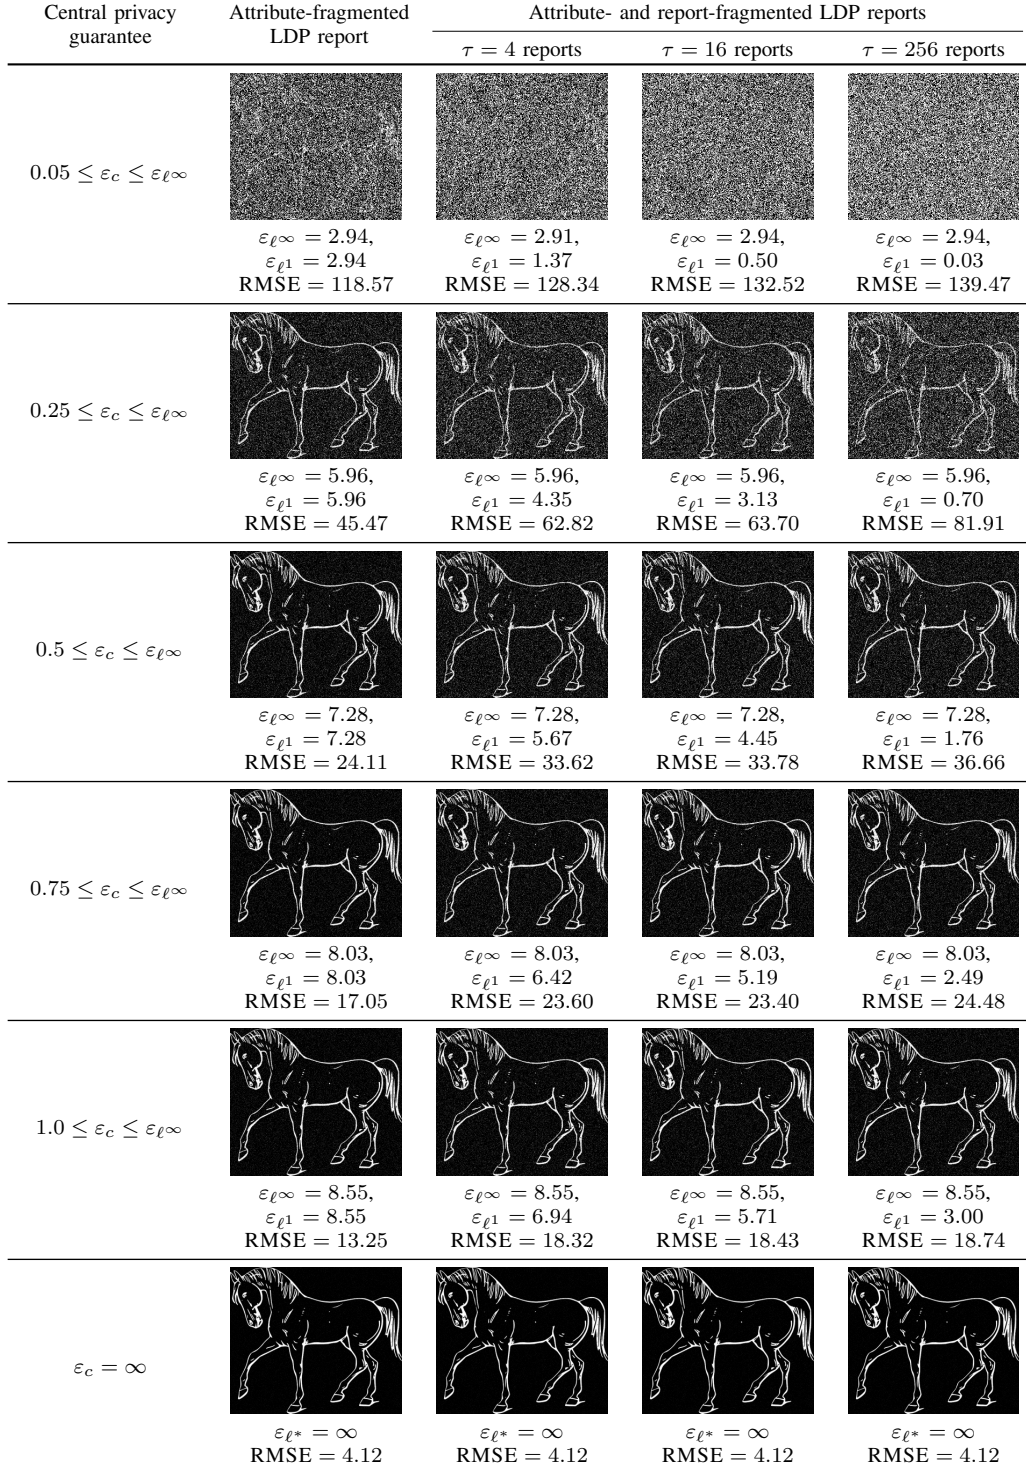<br>$\varepsilon_{\ell*} = \infty$<br>RMSE = 4.12                                       |

TABLE VI: Experimental results of reconstructing the Horse image dataset from a collection of anonymous reports that result from running the LDP reporting protocol one, two, or five times for every single respondent, using all, half, or a fifth of each respondent’s  $\varepsilon_\ell$  privacy budget, respectively. (In all cases, the LDP reports also utilize attribute fragmenting.) In all experiments, the best utility is achieved when the entire  $\varepsilon_\ell$  privacy budget is used to construct LDP reports in a single run.

| Local privacy guarantee       | Single LDP run                                                                                      | Two LDP runs                                                                                         | Five LDP runs                                                                                          |
|-------------------------------|-----------------------------------------------------------------------------------------------------|------------------------------------------------------------------------------------------------------|--------------------------------------------------------------------------------------------------------|
| Total $\varepsilon_\ell=2.94$ | 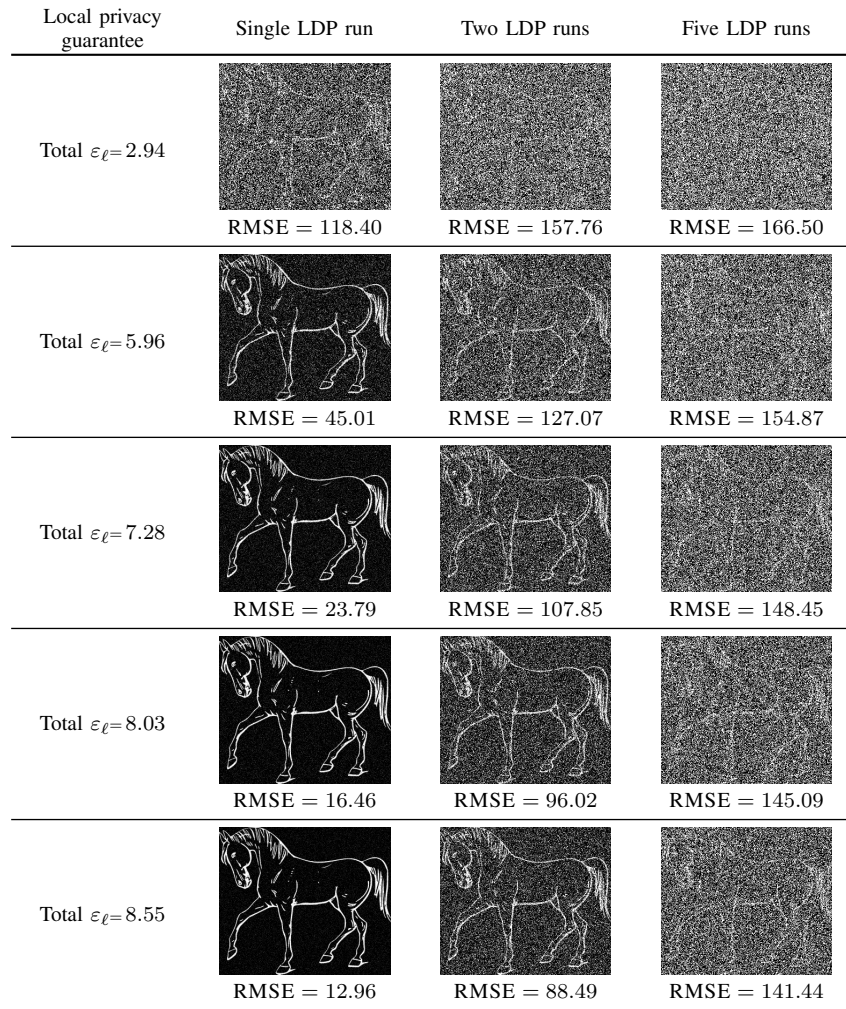<br>RMSE = 118.40  | 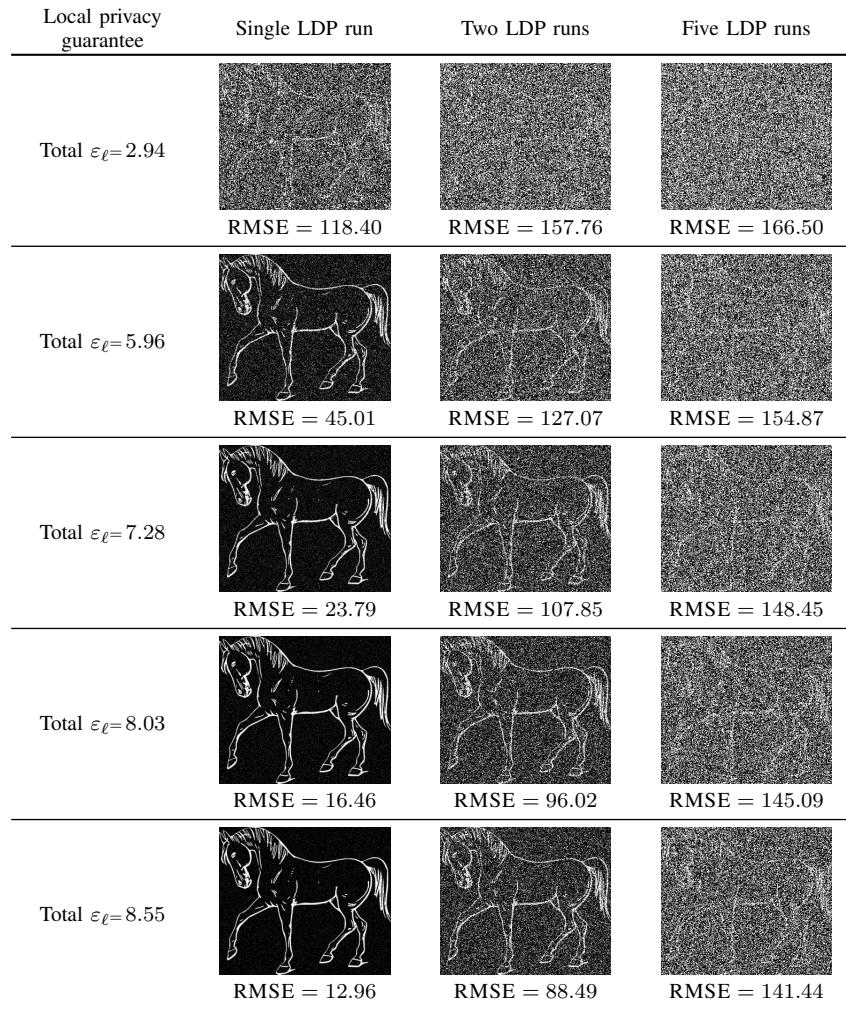<br>RMSE = 157.76   | 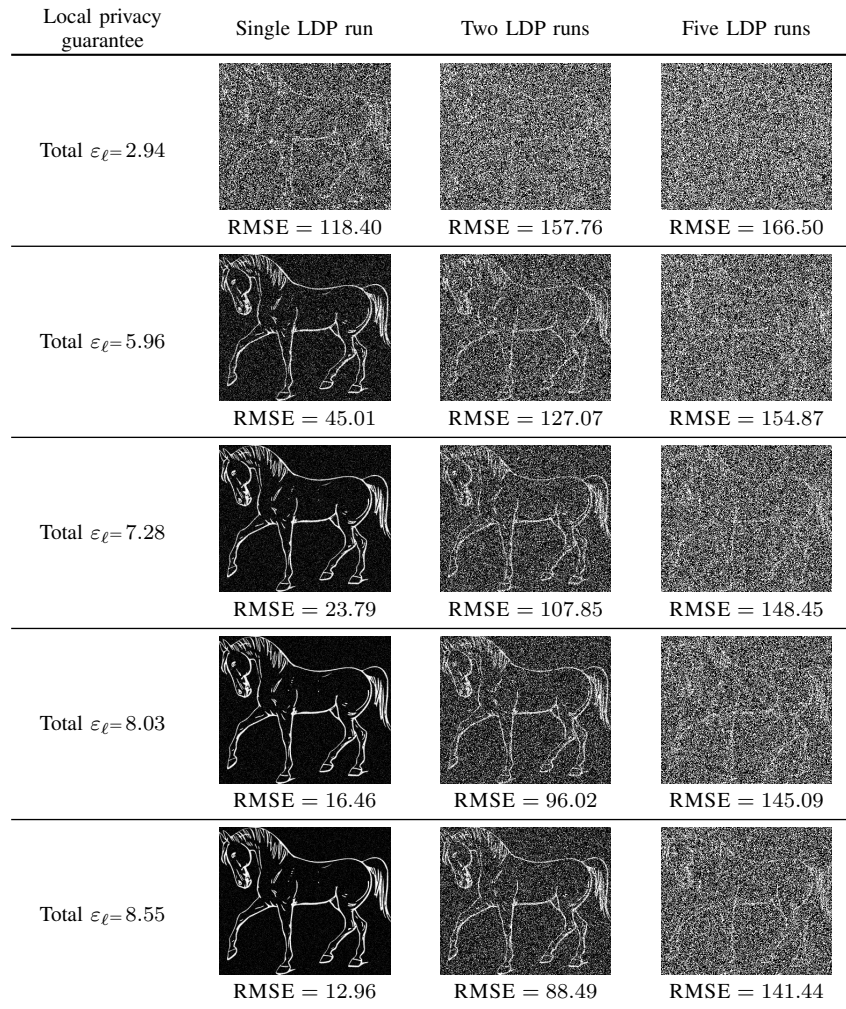<br>RMSE = 166.50   |
| Total $\varepsilon_\ell=5.96$ | 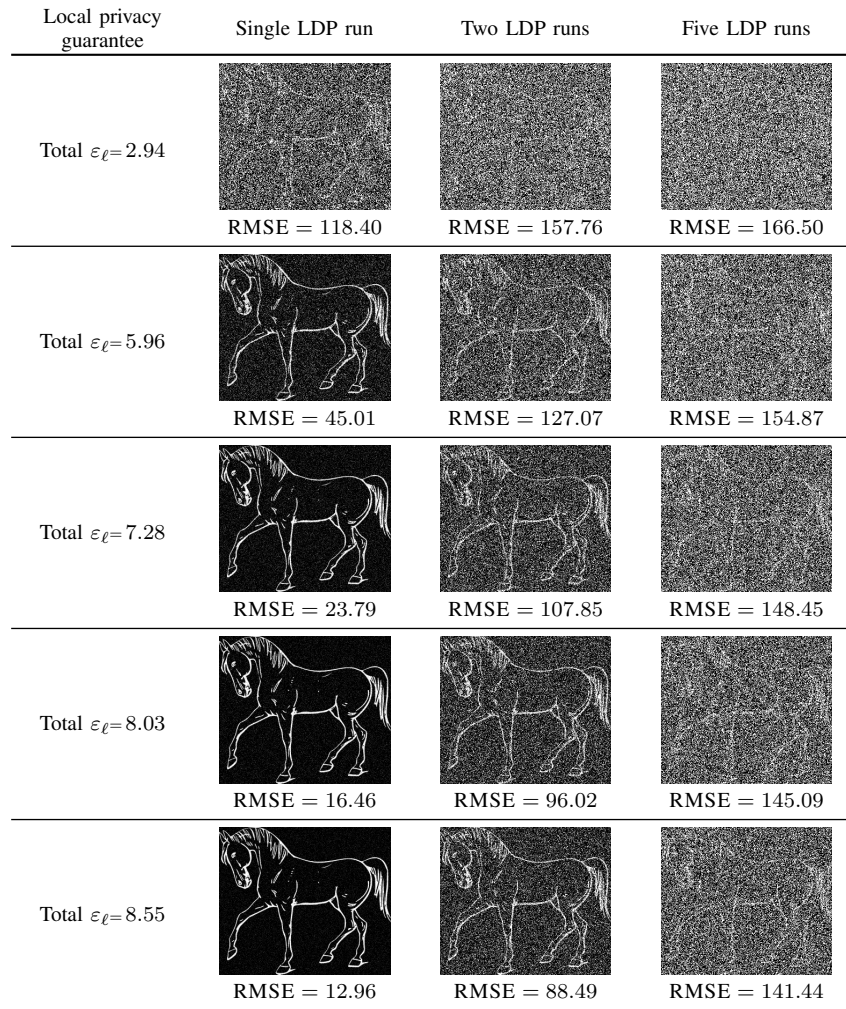<br>RMSE = 45.01  | 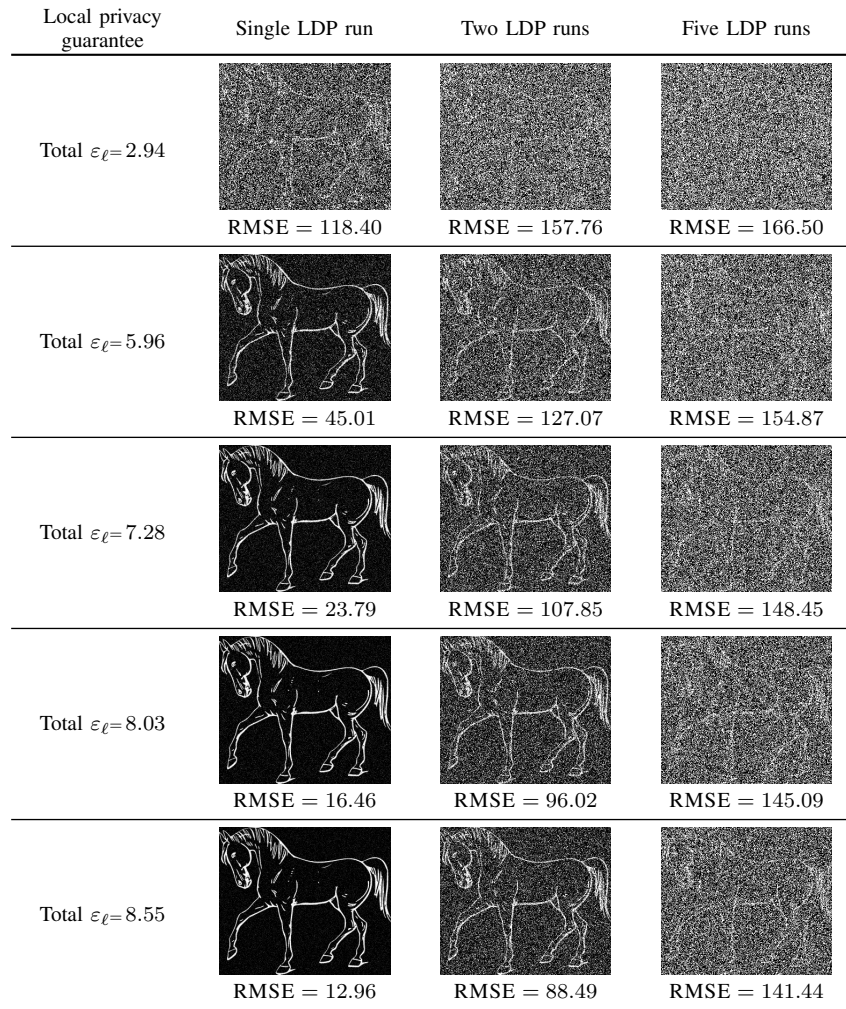<br>RMSE = 127.07  | 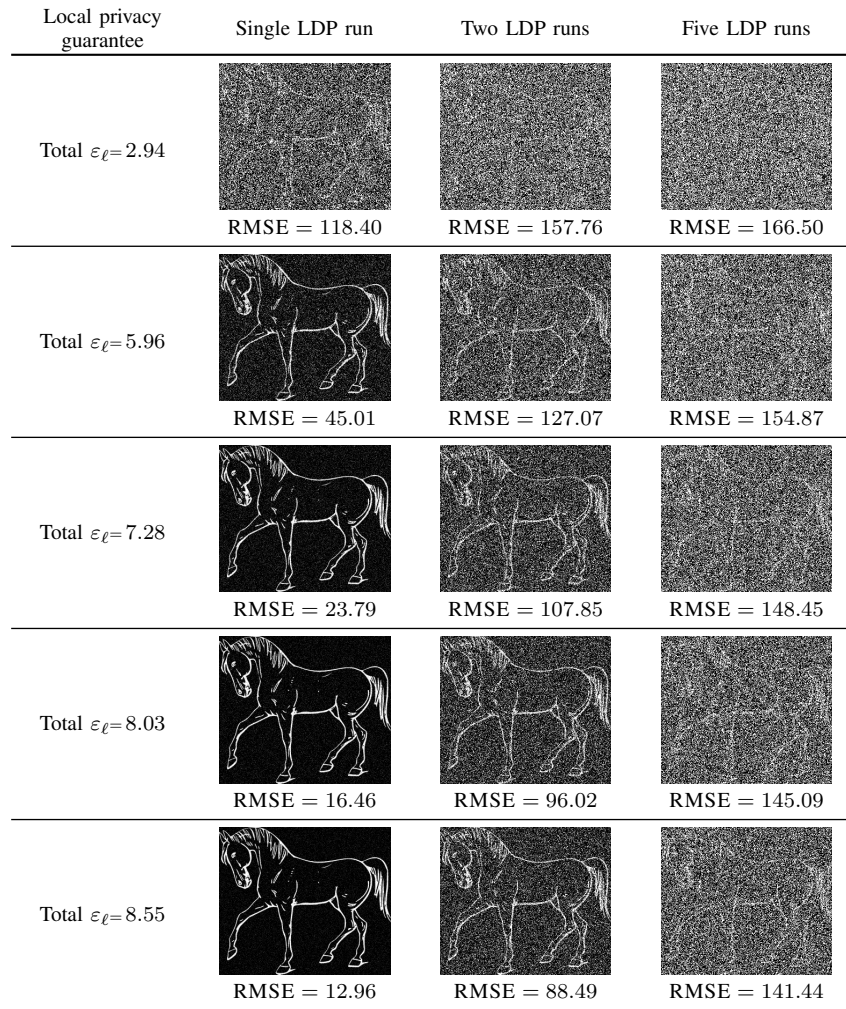<br>RMSE = 154.87  |
| Total $\varepsilon_\ell=7.28$ | 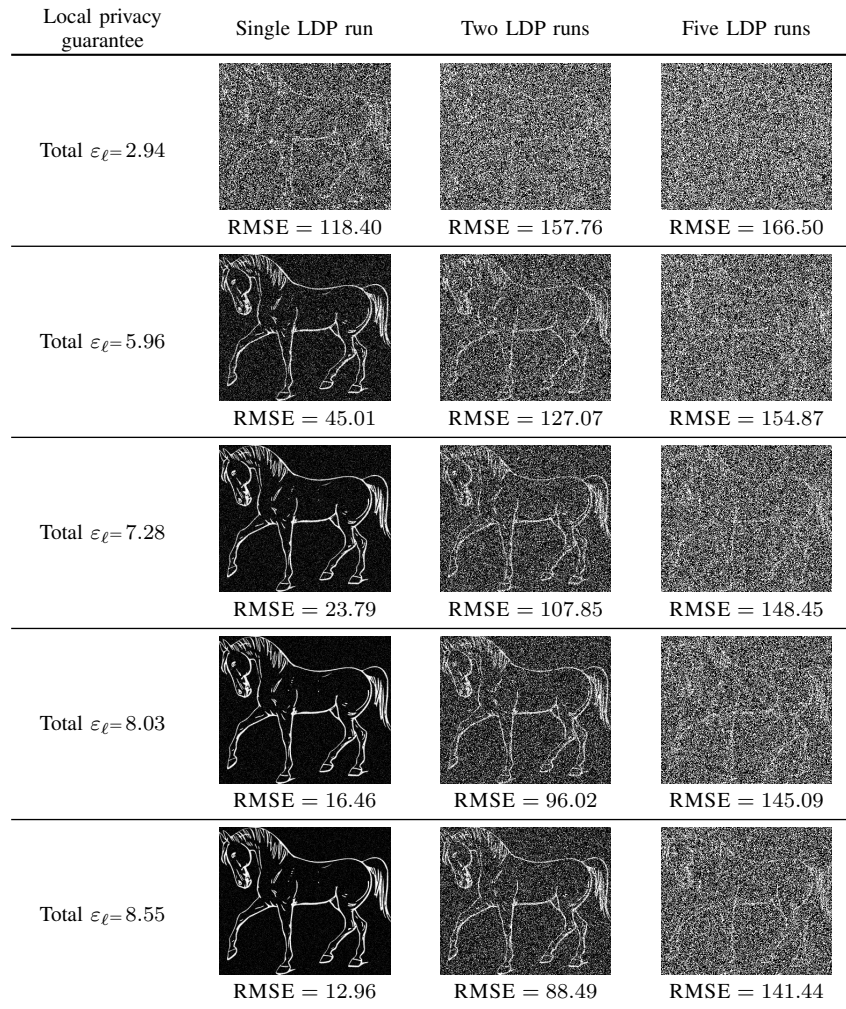<br>RMSE = 23.79 | 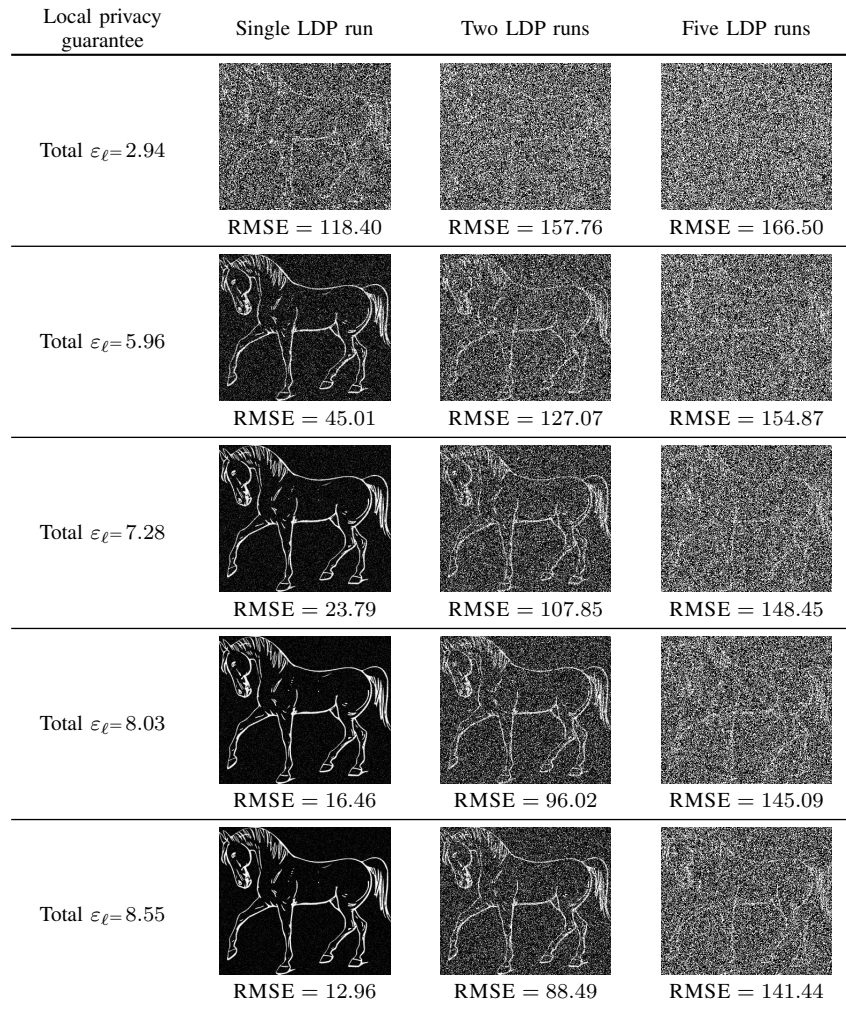<br>RMSE = 107.85 | 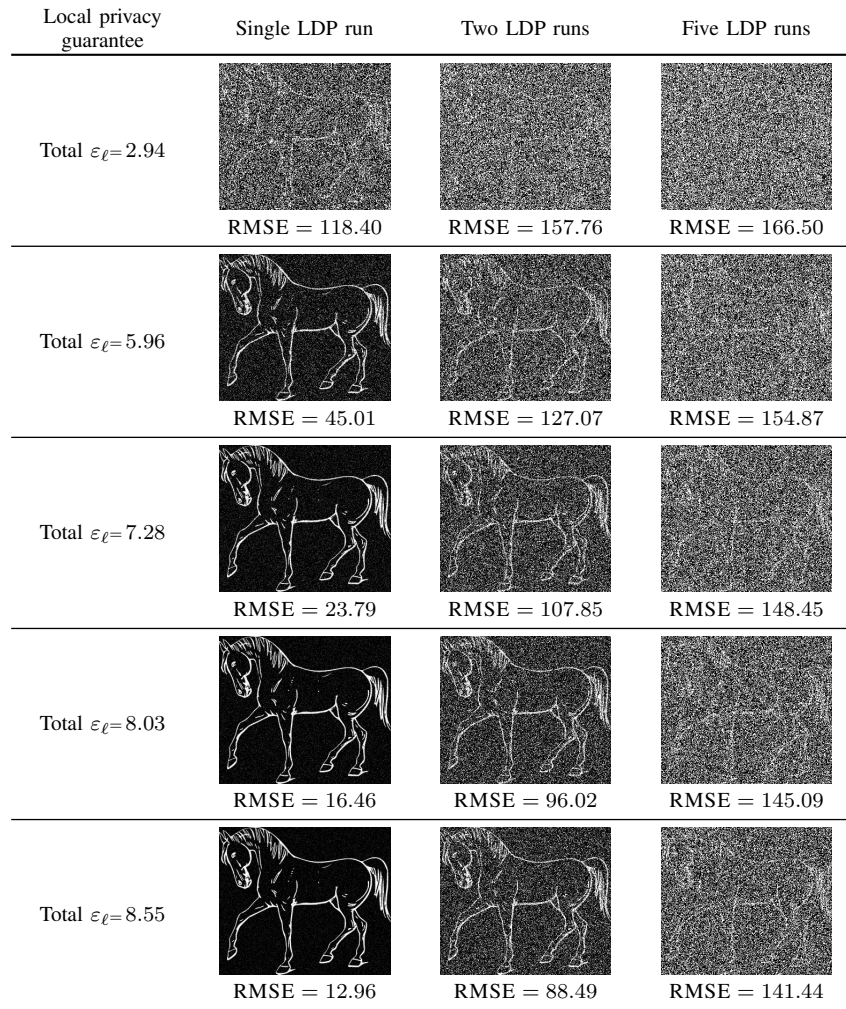<br>RMSE = 148.45 |
| Total $\varepsilon_\ell=8.03$ | 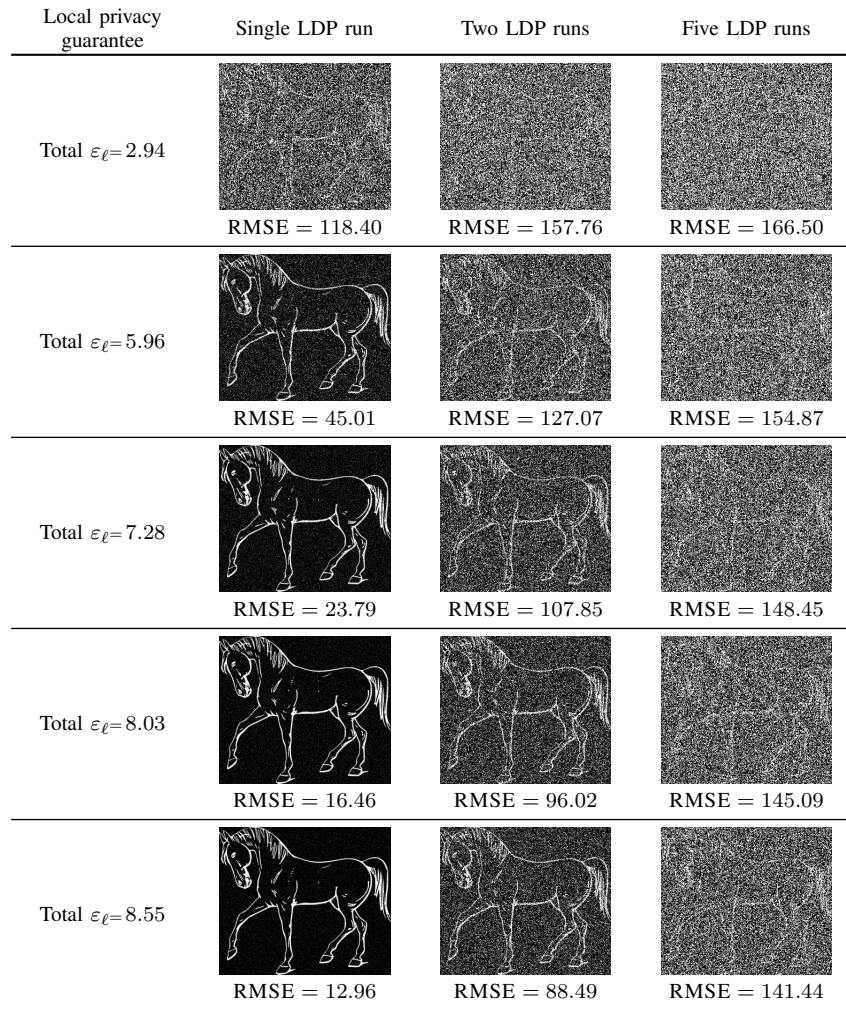<br>RMSE = 16.46 | 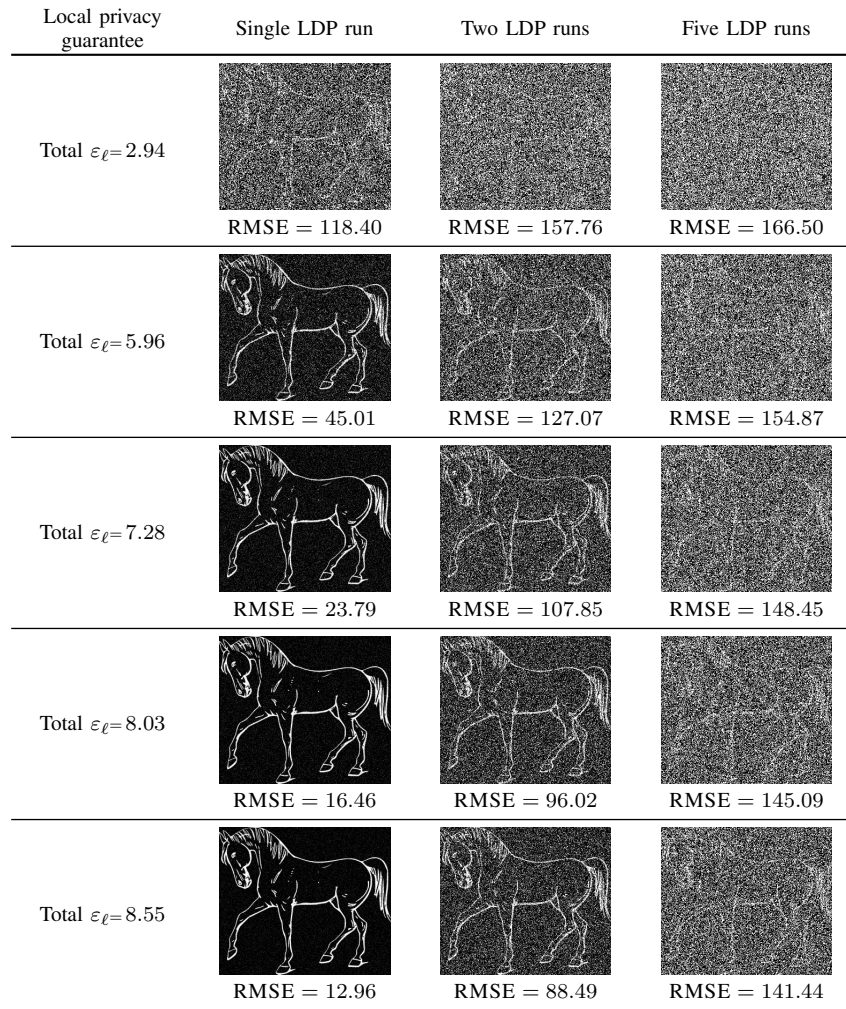<br>RMSE = 96.02  | 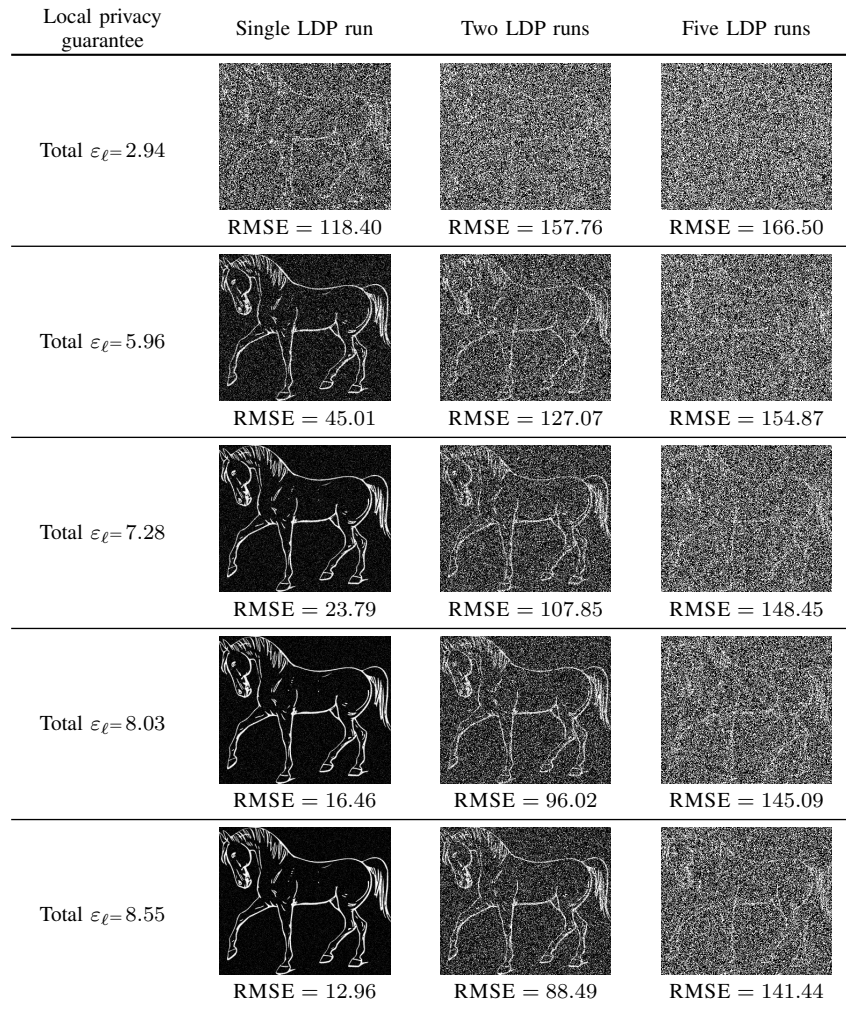<br>RMSE = 145.09 |
| Total $\varepsilon_\ell=8.55$ | 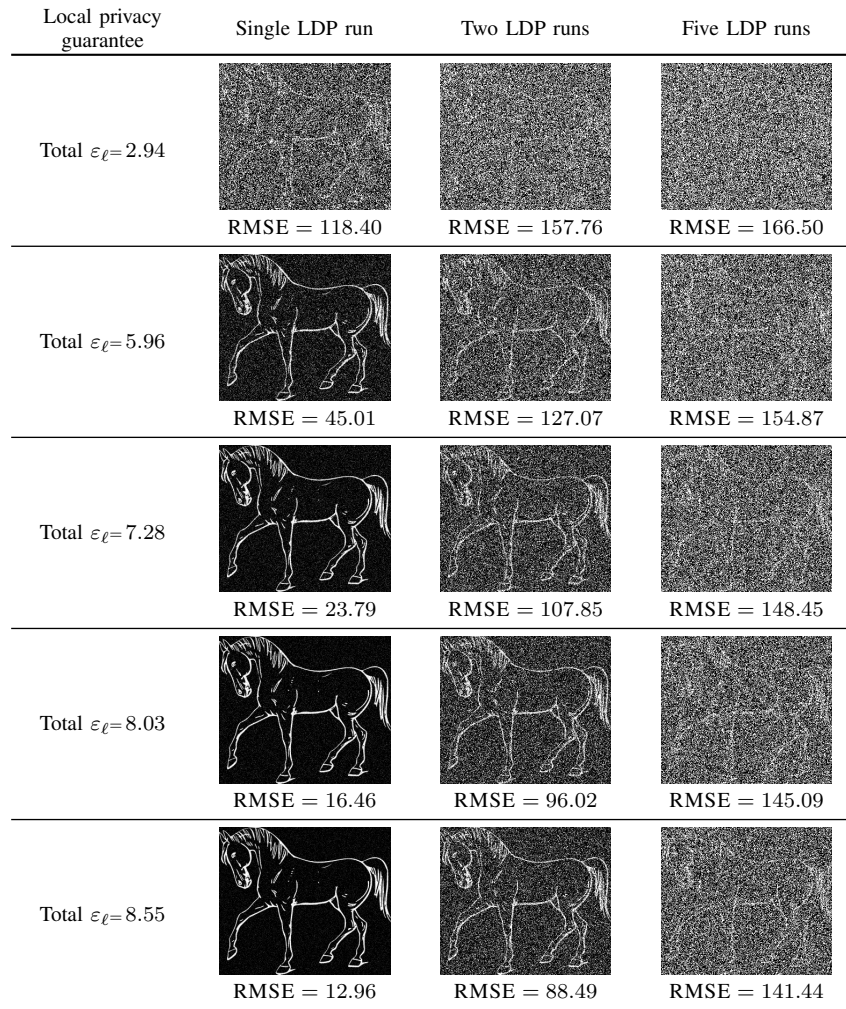<br>RMSE = 12.96 | 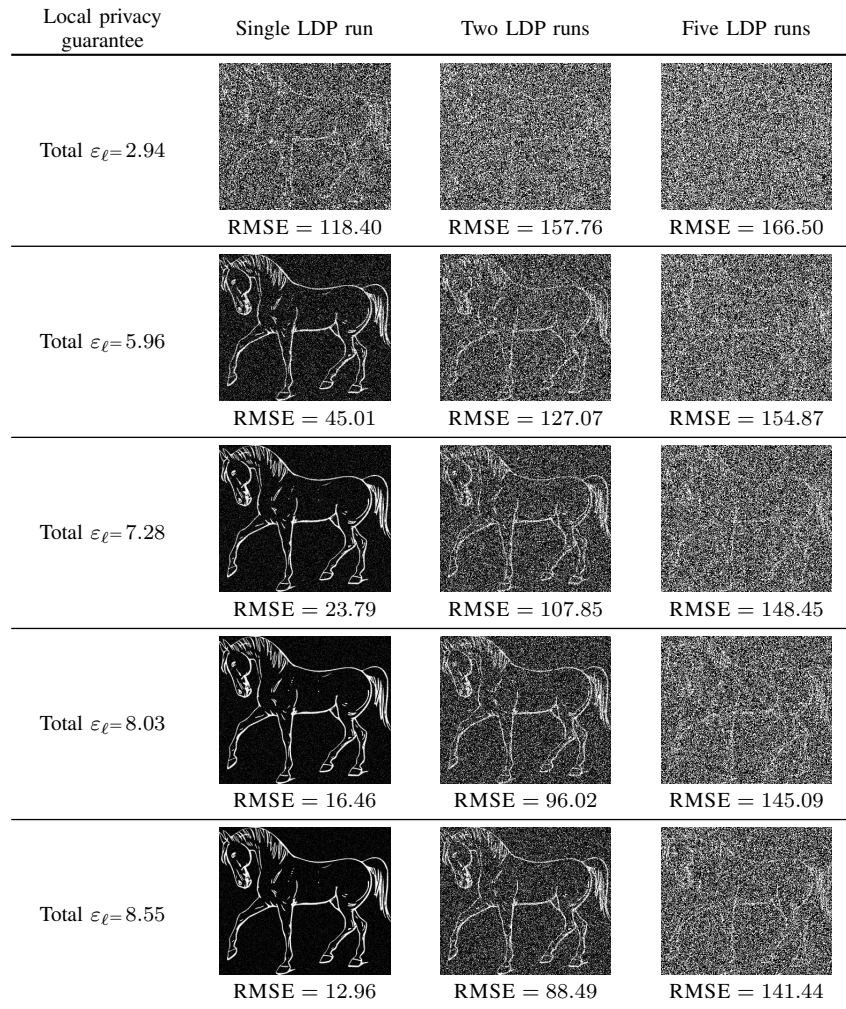<br>RMSE = 88.49  | 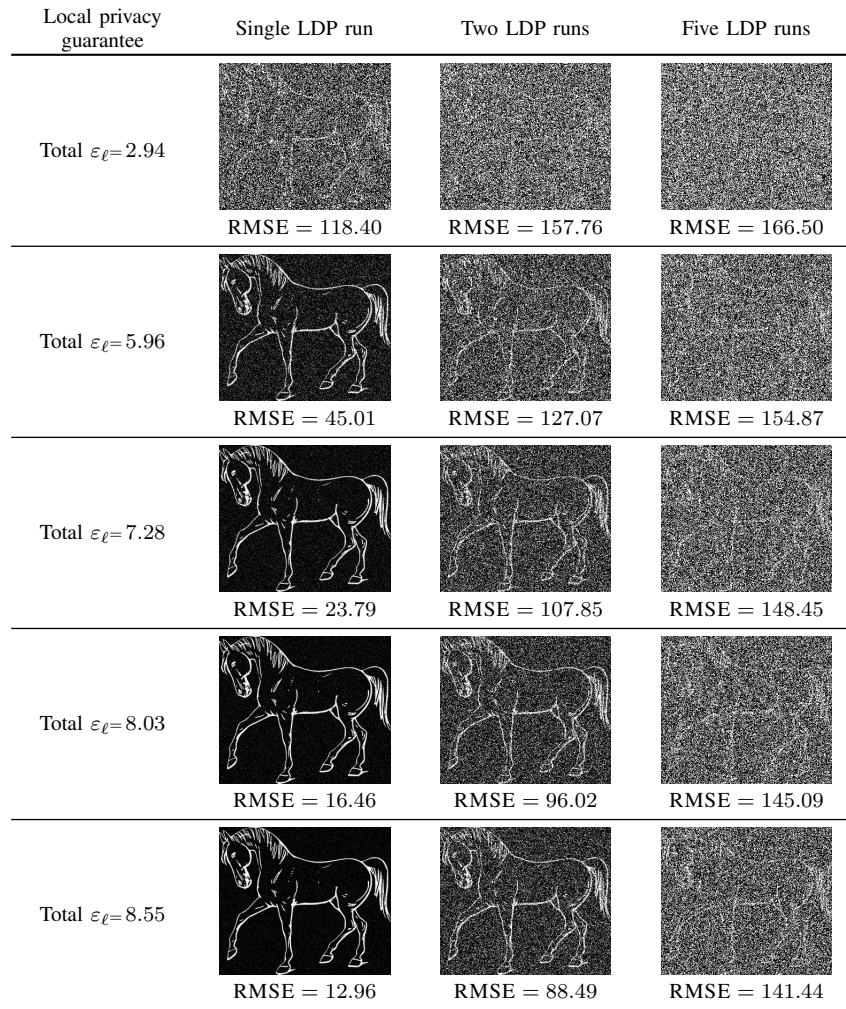<br>RMSE = 141.44 |

TABLE VII: Experimental results of reconstructing the Horse image dataset from LDP reports about the results of one, two, or five sketching hash functions, based on count sketching with 1,024 hash functions and sketch size 65,536. (In each case, the LDP reports also utilize attribute fragmenting.) In all experiments, the best utility is achieved when LDP reports use the entire  $\varepsilon_\ell$  privacy budget to report on the result of a single hash function.

| Local privacy guarantee       | One hash function                                                                                   | Two hash functions                                                                                  | Five hash functions                                                                                    |
|-------------------------------|-----------------------------------------------------------------------------------------------------|-----------------------------------------------------------------------------------------------------|--------------------------------------------------------------------------------------------------------|
| Total $\varepsilon_\ell=2.94$ | 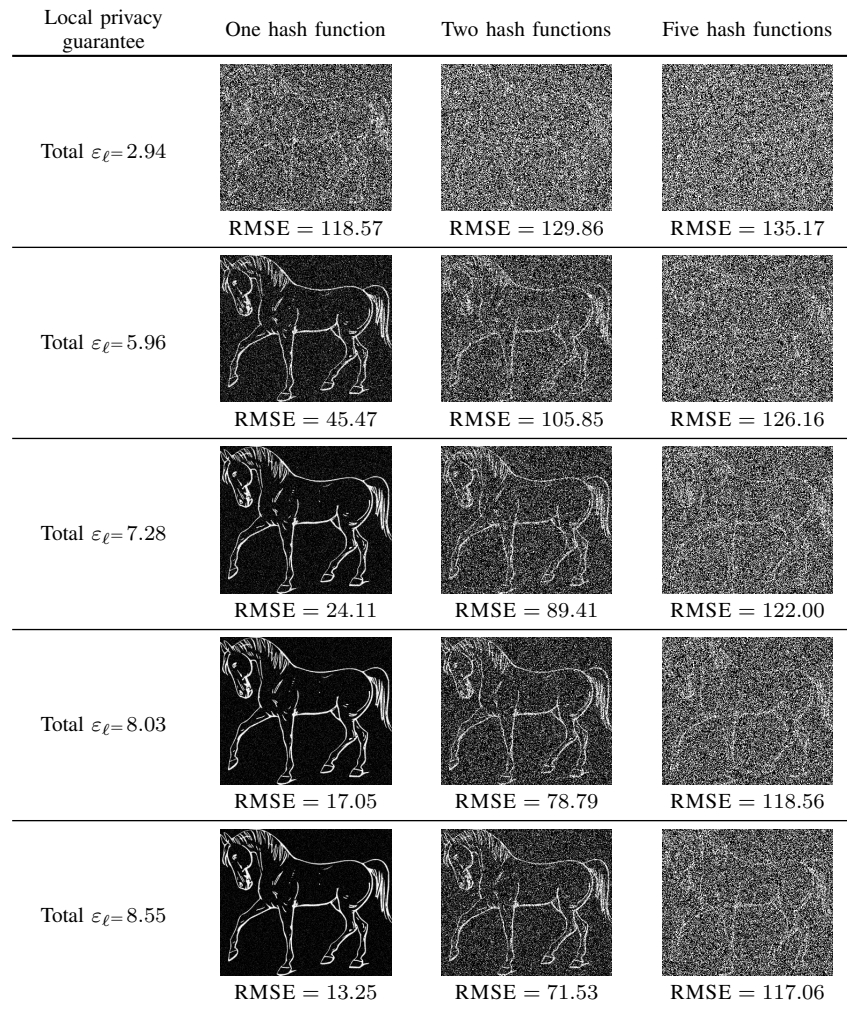<br>RMSE = 118.57  | 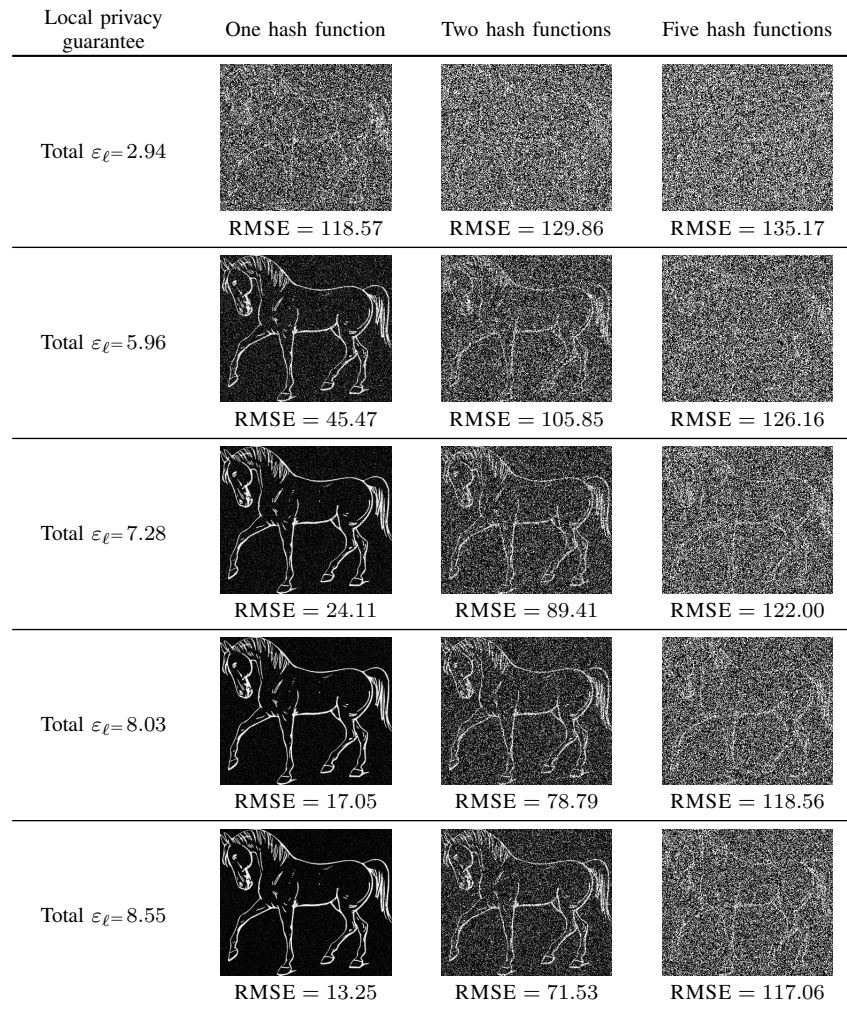<br>RMSE = 129.86  | 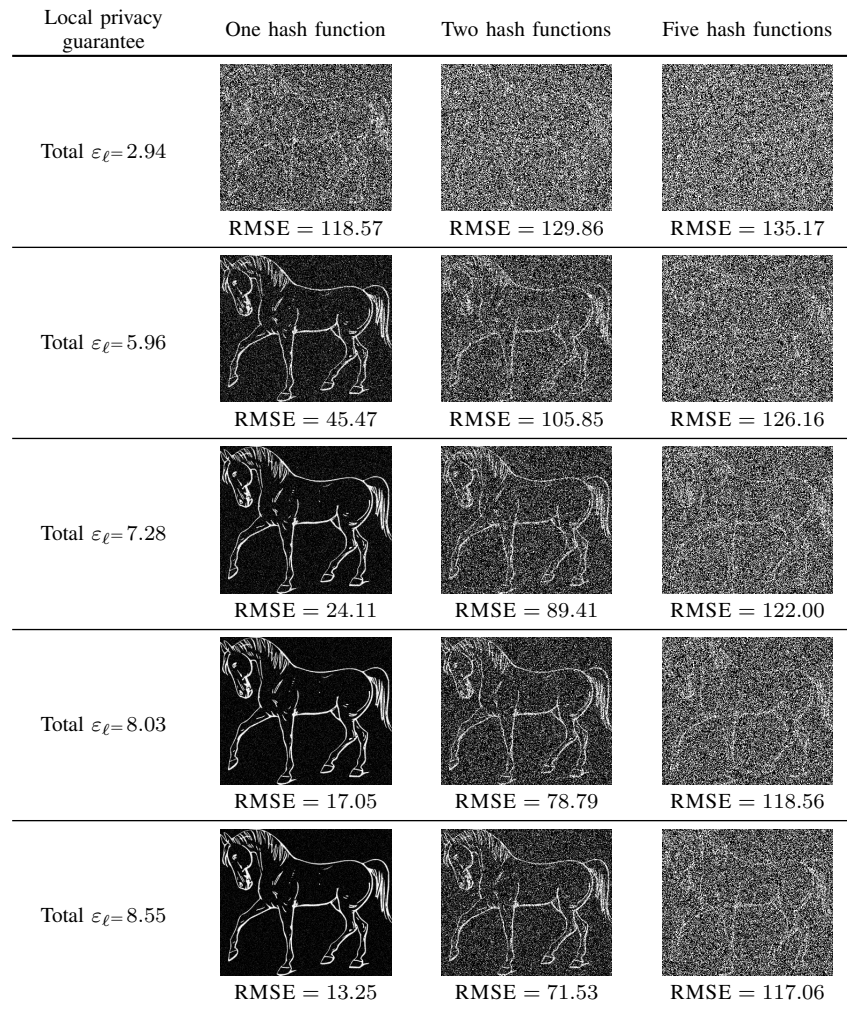<br>RMSE = 135.17   |
| Total $\varepsilon_\ell=5.96$ | 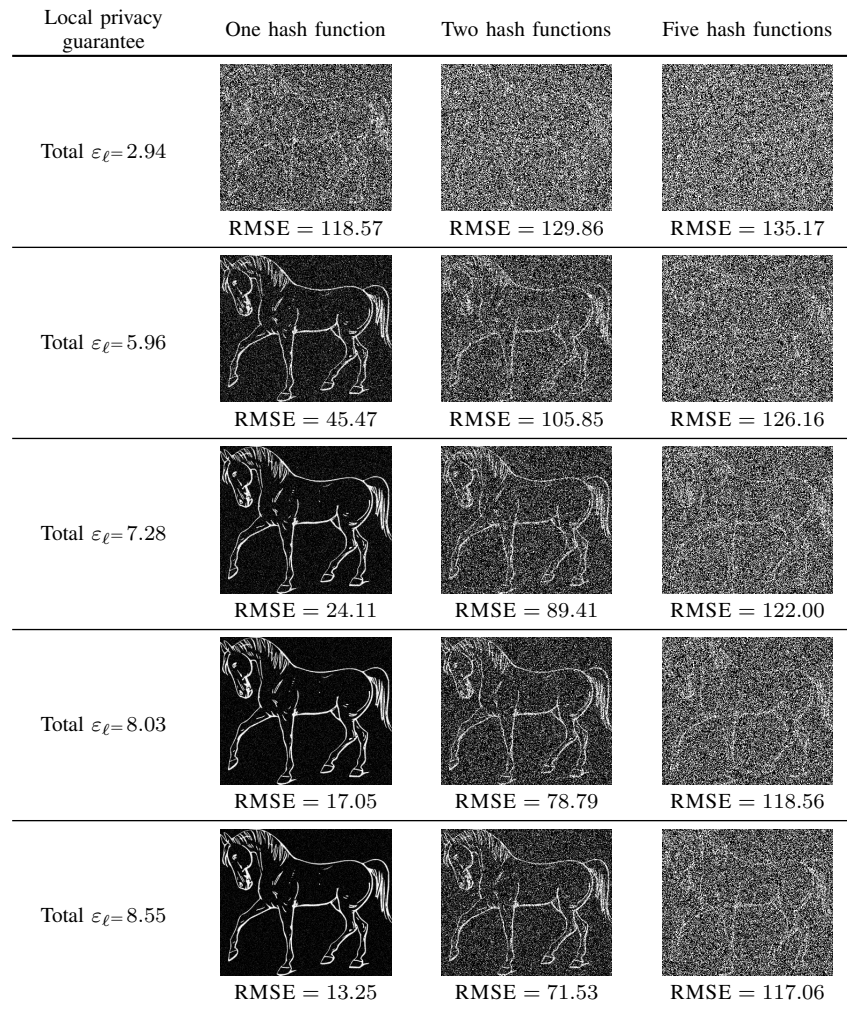<br>RMSE = 45.47   | 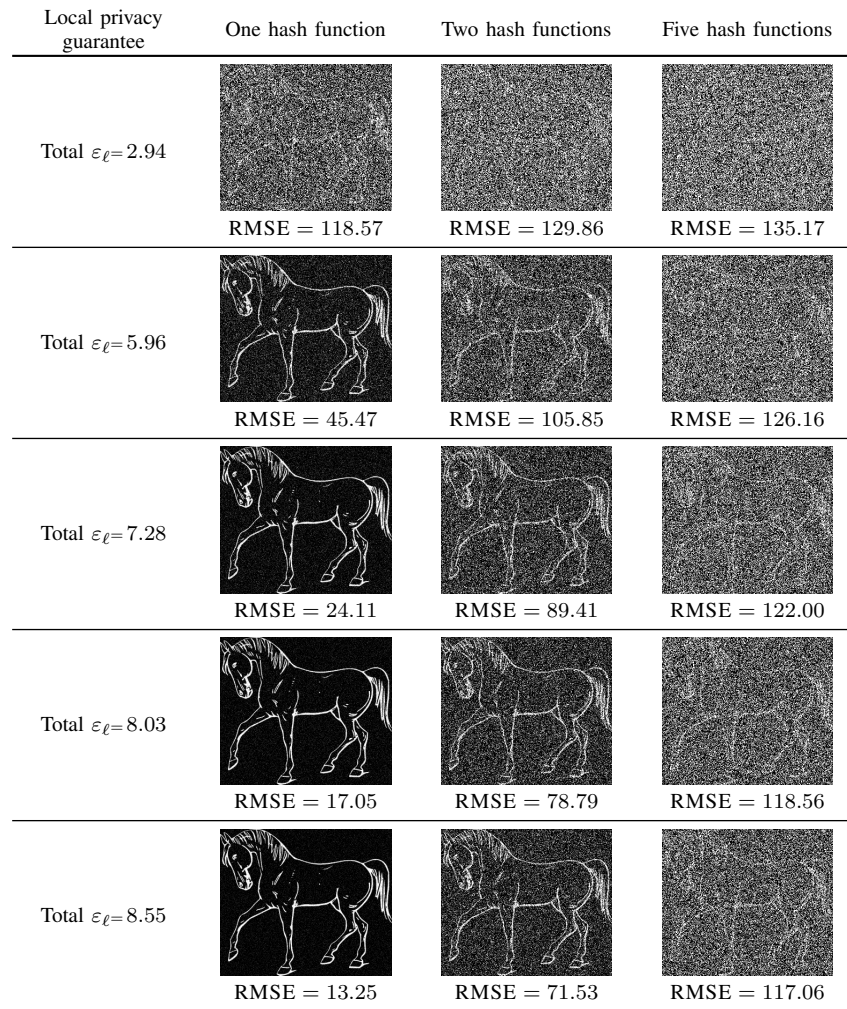<br>RMSE = 105.85  | 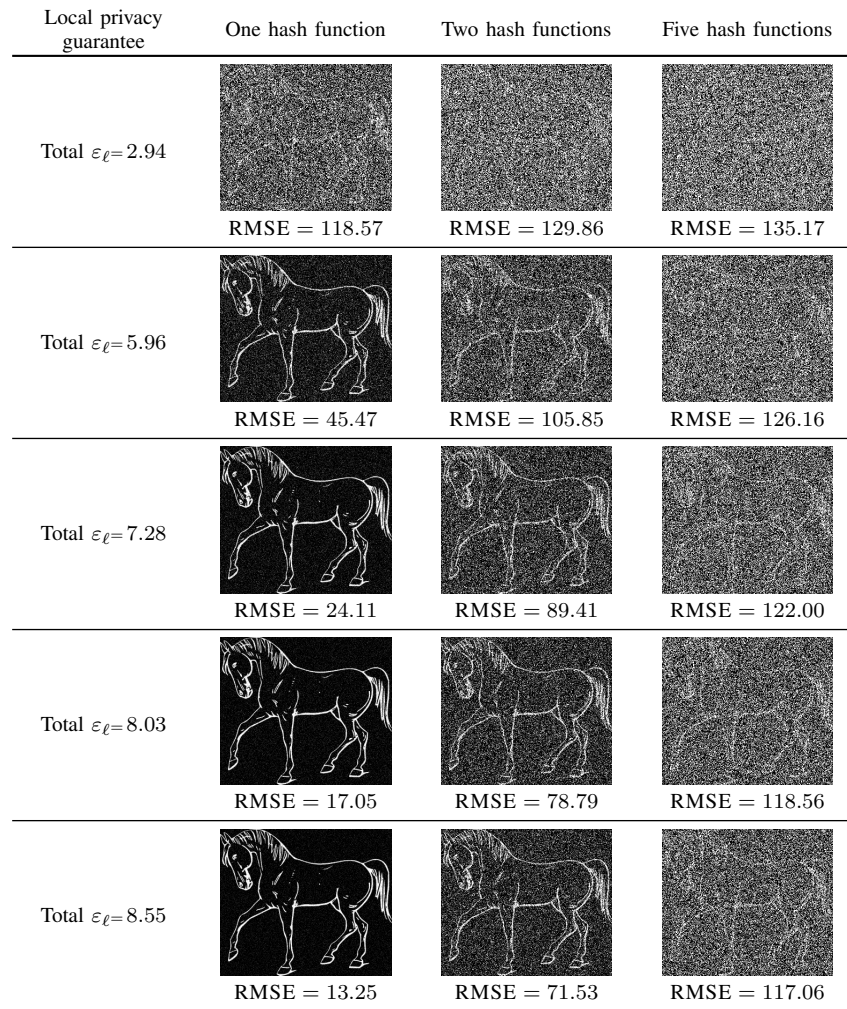<br>RMSE = 126.16   |
| Total $\varepsilon_\ell=7.28$ | 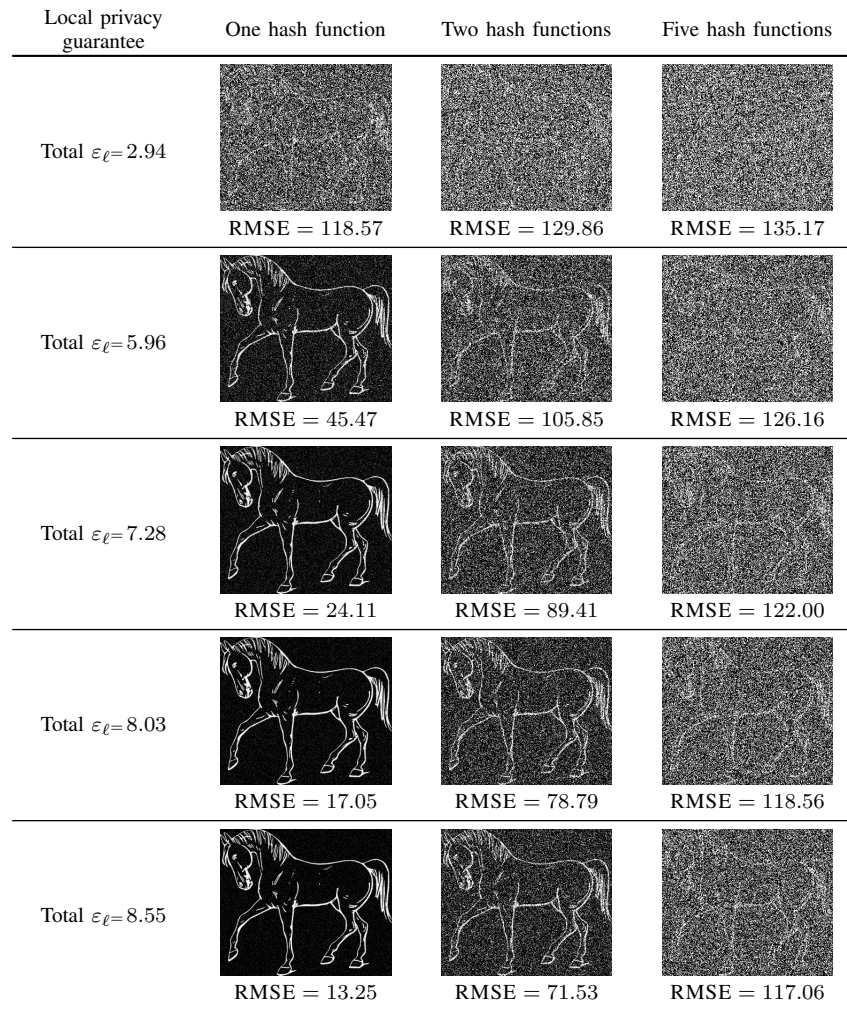<br>RMSE = 24.11 | 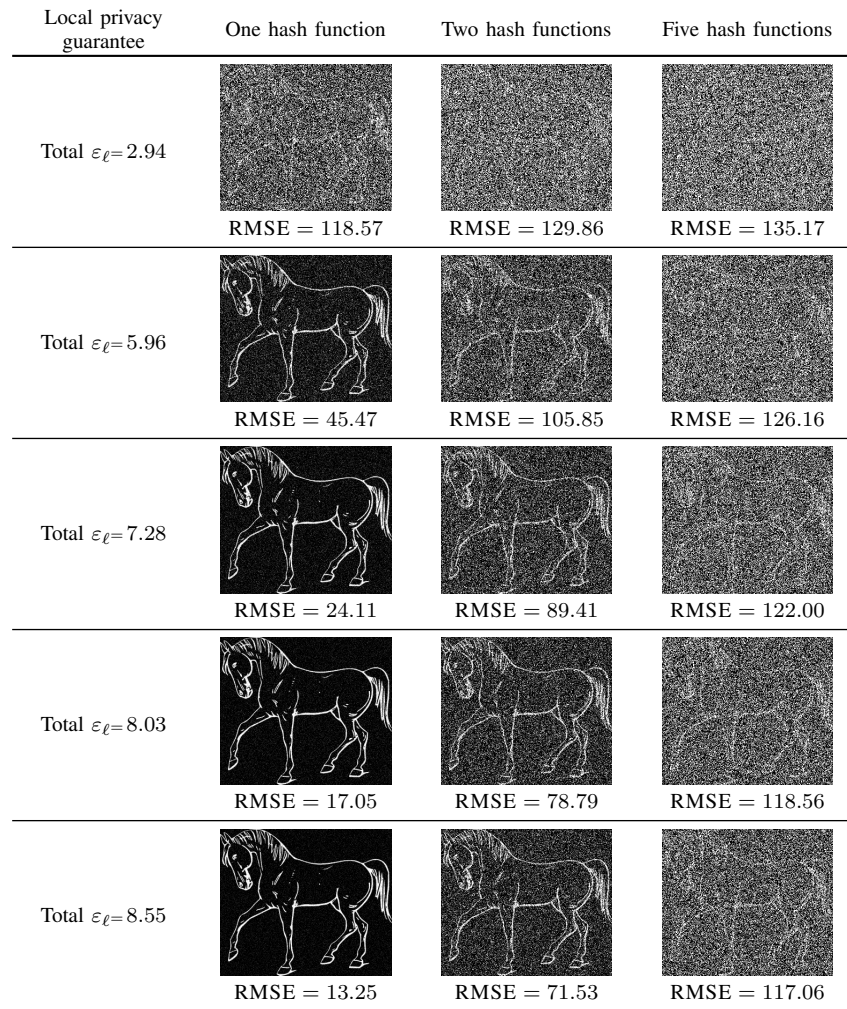<br>RMSE = 89.41 | 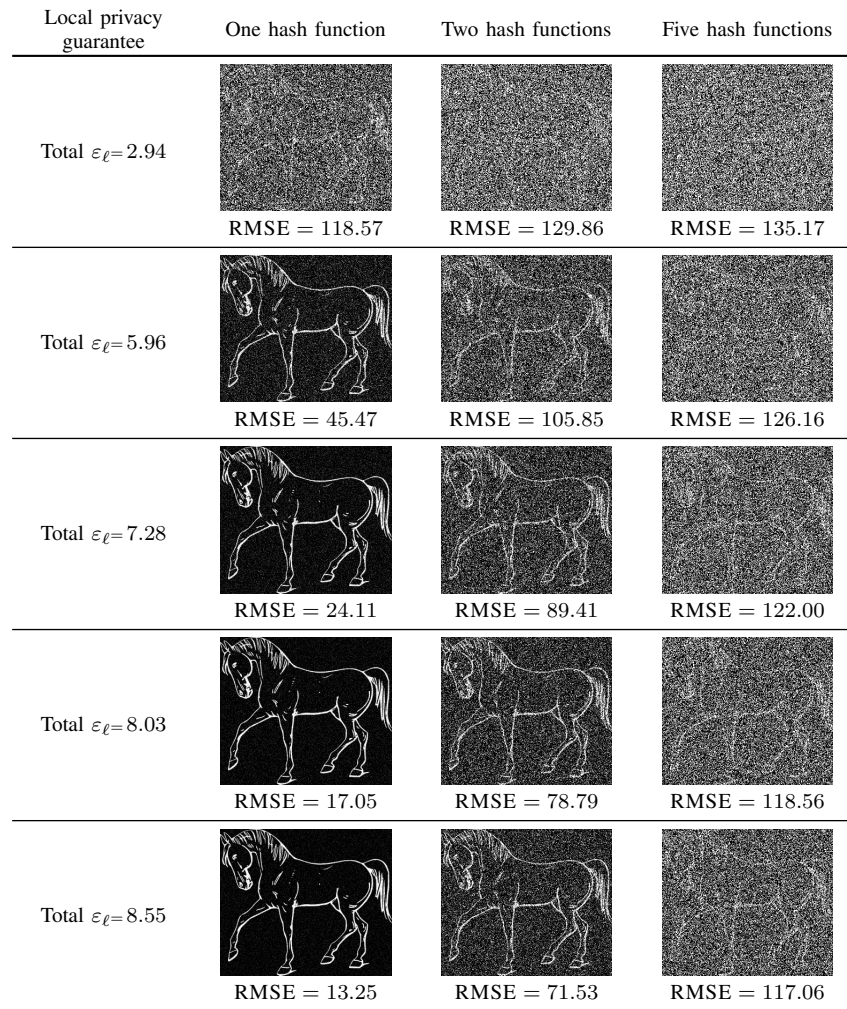<br>RMSE = 122.00 |
| Total $\varepsilon_\ell=8.03$ | 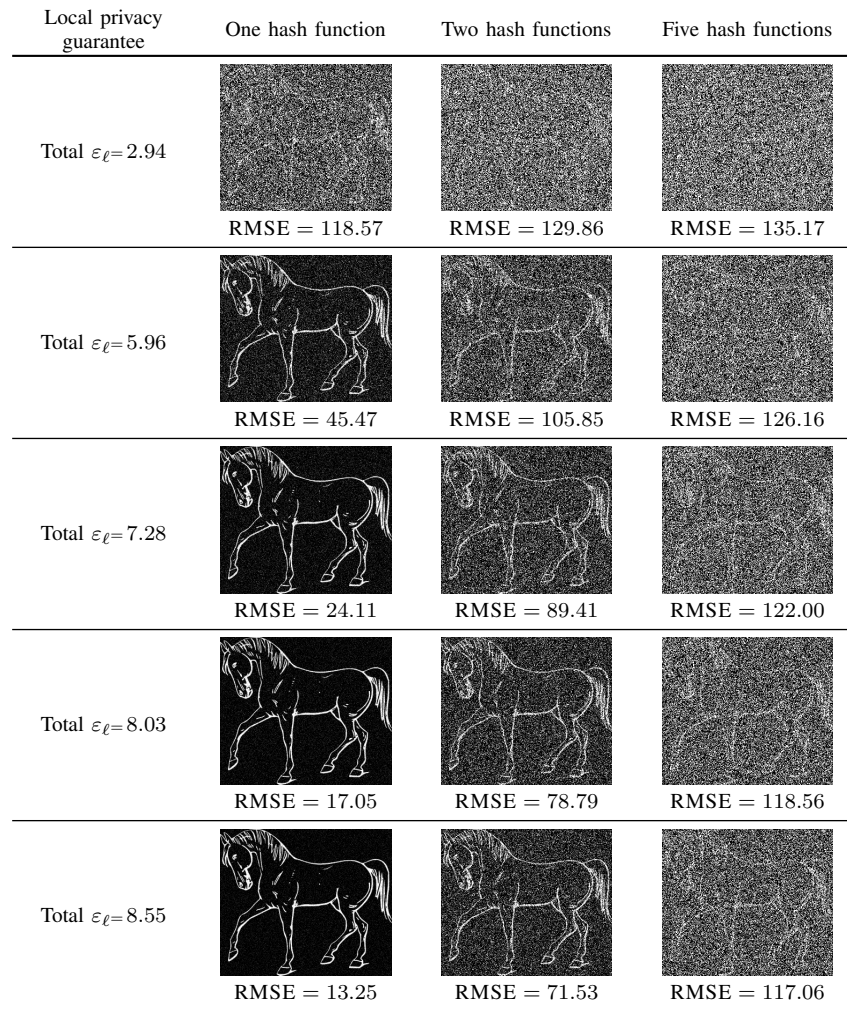<br>RMSE = 17.05 | 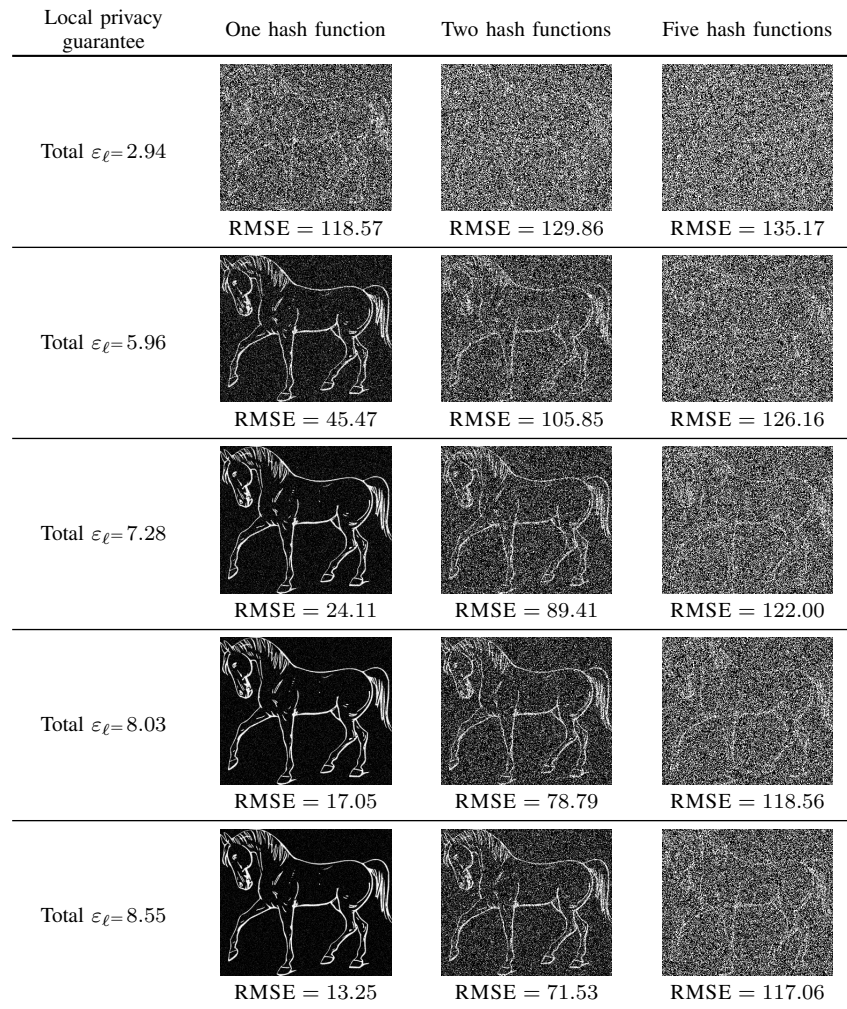<br>RMSE = 78.79 | 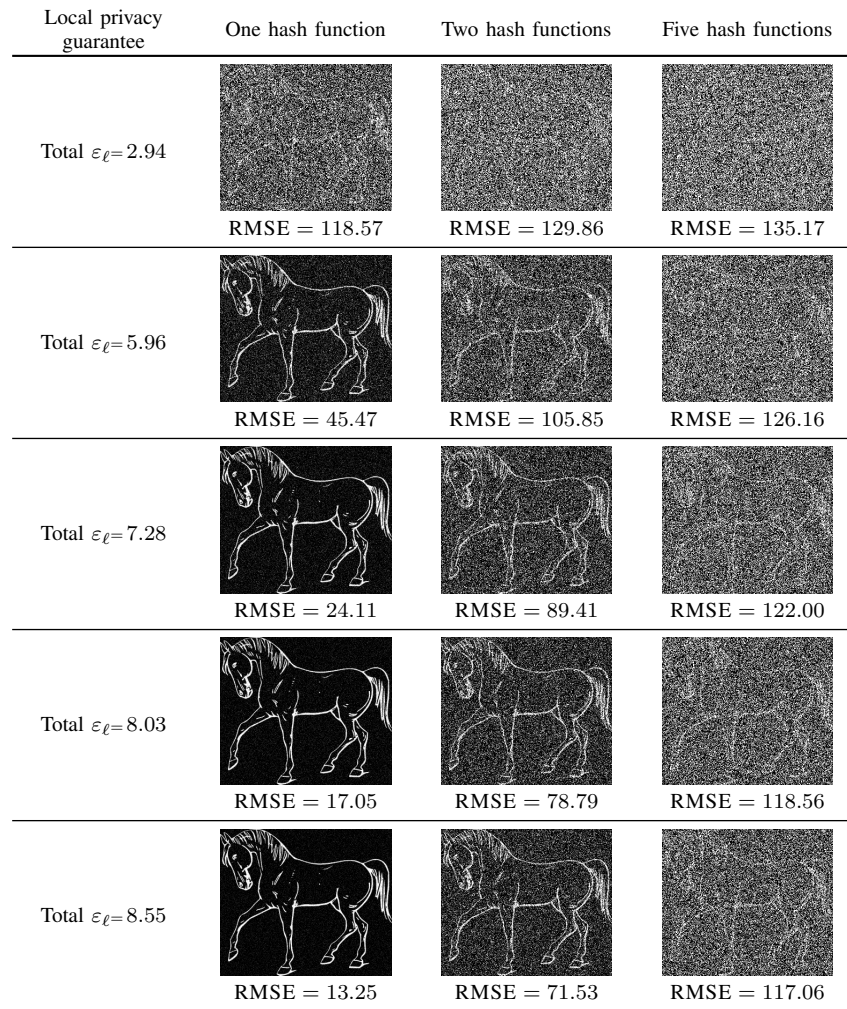<br>RMSE = 118.56 |
| Total $\varepsilon_\ell=8.55$ | 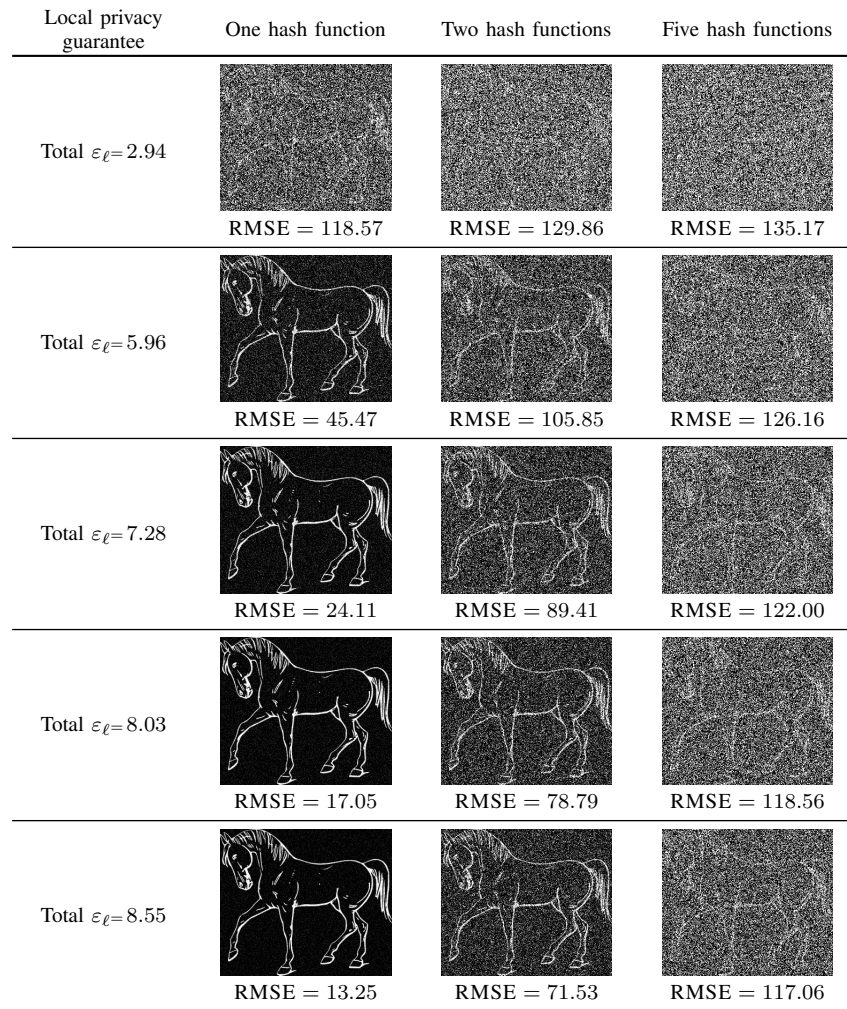<br>RMSE = 13.25 | 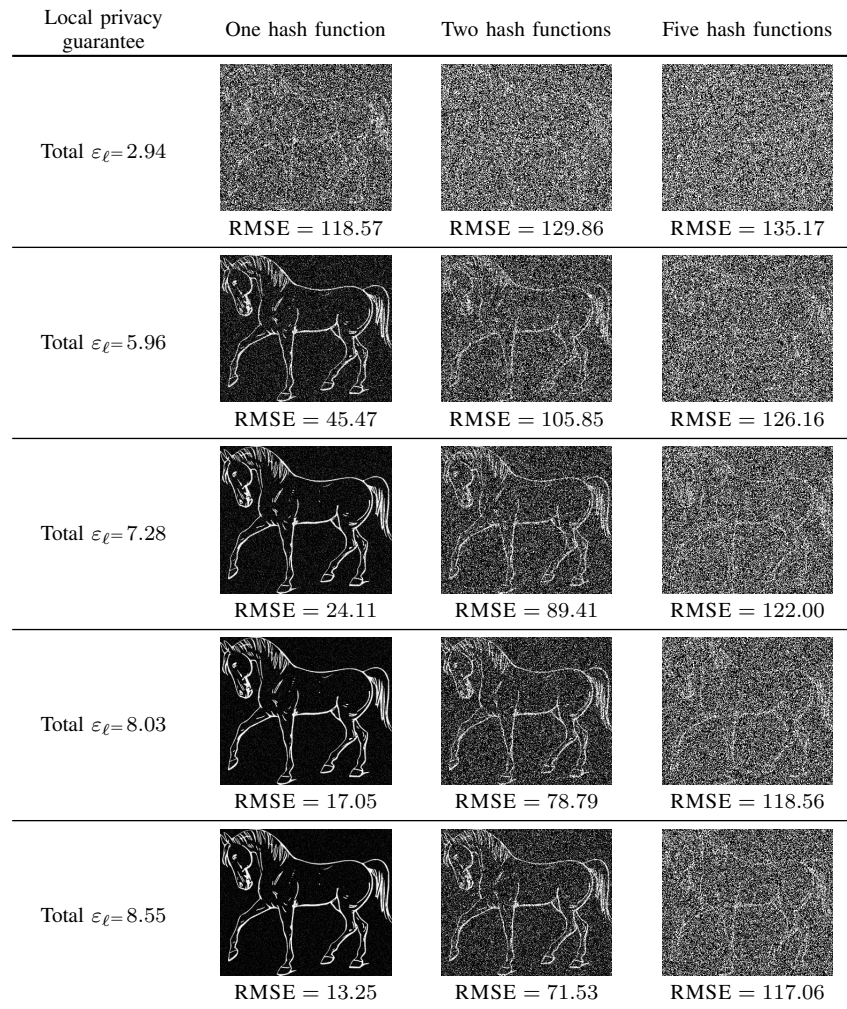<br>RMSE = 71.53 | 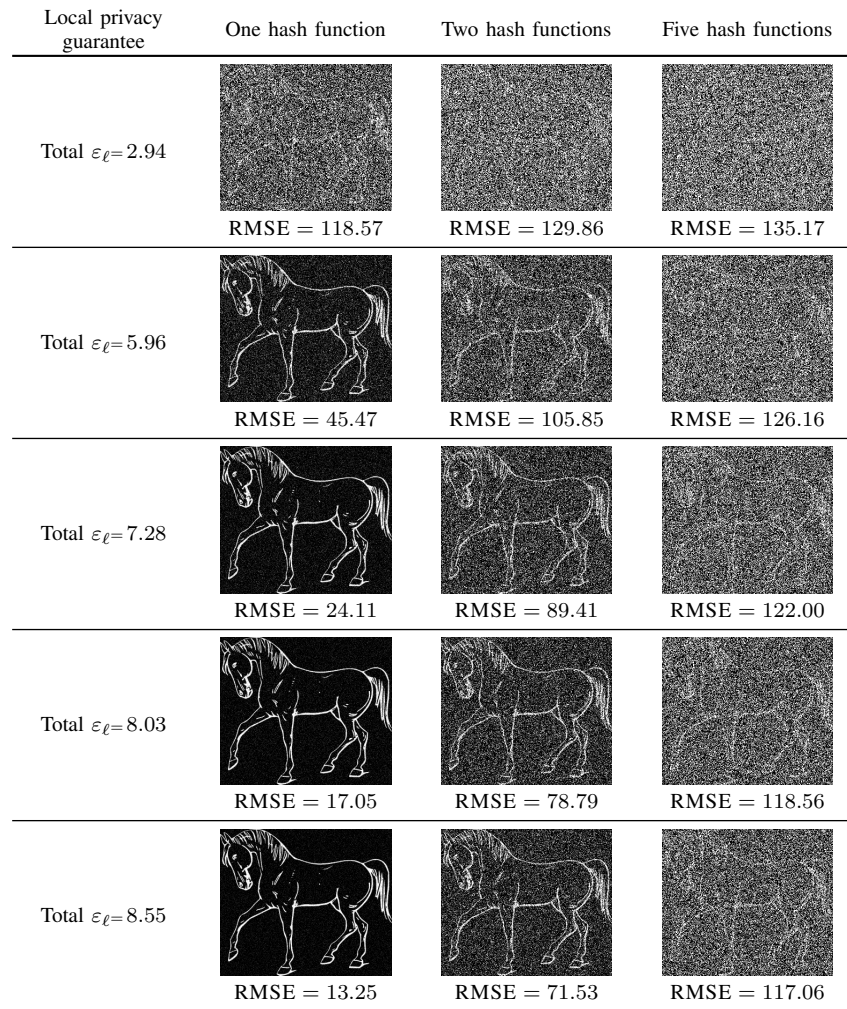<br>RMSE = 117.06 |
